# Supplementary material for: Privacy-Preserving Federated Learning on Partitioned Attributes
Source: arXiv:2104.14383 source file (2021-04-29)
Supplement: Supplementary file 1 [file appendix.tex]

\appendix
\section{Related Work}
%\textbf{Federated learning.} Federated learning was first proposed by Google\cite{konevcny2016federated1,konevcny2016federated2,mcmahan2017communication} with the goal of training models with datasets distributed among different mobile devices without sharing raw data. Based on the dataset distribution characteristics, federated learning can be categorized into three types: horizontal federated learning, vertical federated learning, and federated transfer learning. We concentrate on vertical federated learning where distributed datasets share the same feature space but different samples. 

Most previous works have demonstrated the threat of privacy leakage in horizontal federated learning. \cite{nasr2019comprehensive,melis2019exploiting} launch the membership inference attack which aims to determine whether a specific record is in a client’s training dataset or not. Other attacks including \cite{melis2019exploiting,geiping2020inverting,zhu2019deep,bagdasaryan2020backdoor} exploit the iteratively exchanged gradients during training. \cite{melis2019exploiting} shows the periodically exchanged model updates leak unintended information about participants’ training data. Likewise, \cite{geiping2020inverting} reconstructs input images from gradients. \cite{zhu2019deep} introduces an approach to obtain the local training data from public shared gradients. Different from them, \cite{luo2020feature} proposes feature inference attack to vertical FL but at the inference stage, rather than at the training phase.

Mainstream methods for privacy-preserving federated learning include differential privacy and crypto-based solutions. Differential privacy introduces additive noise to the features or the model \cite{geyer2017differentially,roy2020crypt} for privacy but degrades model performance. Homomorphic encryption (HE) supports model updates exchange in the encrypted domain without exposing any data in plaintext. \cite{hardy2017private} uses Taylor expansion to approximate the Sigmoid function and \cite{zhang2018gelu} splits each neuron into linear and nonlinear components and implement them separately on non-colluding parties. However, it is not feasible to approximate a deep neural network with a low-degree polynomial function accurately and efficiently, letting alone in the encrypted domain of high complexity.

\section{Datasets and Pre-processing}
\subsection{COCO-QA}
COCO~\cite{lin2014microsoft} is a large-scale dataset for object detection which is achieved by gathering images of complex everyday scenes containing common objects in their natural context. Each image in COCO has at least one object and the dataset contains photos of 90 objects types. COCO-QA~\cite{ren2015exploring} is a widely used dataset for visual question answering (VQA). The QA pairs which include an image and a corresponding question are generated automatically from the COCO captions using a question generating algorithm. COCO-QA contains 78,736 QA pairs for training and 38,948 pairs for testing. There are 11658 and 430 different words in questions and answers respectively and one word for one answer.

In our experiments, QA pairs are distributed between two clients: one client holds the image and the other holds the question. The adversary aims to predict whether the image contains a certain object.
\subsection{Purchase100}
The purchase100 dataset is generated from Kaggle's `acquire valued shopper' challenge which contains the shopping records from several thousand online customers. The goal of this dataset is to identify offers that would attract new shoppers. We adopt a processed and simplified version from \cite{shokri2017membership}. Each record is the shopping history of a single user which contains 600 binary feature. Each feature represents whether the customer has bought this item. The dataset has 197,324 data records and are clustered into 100 classes based on the similarity of the purchases.

\subsection{Credit}
The credit dataset is generated from Kaggle's `Credit Card Fraud Detection' challenge which contains transactions made by credit cards in September 2013 by european cardholders and is used to predict whether a transaction is 
fraud or not. The dataset is highly unbalanced containing 492 frauds out of 284,807 transactions which means the positive class (frauds) account for 0.172\% of all transactions. Due to the unbalanced distribution, we use the Area Under the Precision-Recall Curve (AUC) to measure the accuracy.

The datasets contains 30 numerical attributes including `Time', `Amount' and Features V1, V2, $\cdots$V28 which are the principal components obtained with PCA. Since the range of each attribute varies greatly, we drop the `Time' and `Amount' attribute and normalize the remaining attributes.

\subsection{UCI Adult}
This UCI Adult dataset is generated from Kaggle's `Adult Census Income' challenge which includes 48,842 records with 14 attributes such as age, gender, education, marital status, occupation, working hours, and native country. The classification task is to predict if a person makes over \$50K a year based on the census attributes. We convert all attributes including string and continuous numerical attributes to categorical types. For example, we convert age attribute to 10 classes with each class spanning 10 years.

\section{Models and Hyperparameters}
\subsection{Model structure}
\subsubsection{COCO-QA}
For COCO-QA, the client with image owns a VGG11 pre-trained on ImageNet and the last layer of VGG11 is replaced by a linear layer with 1024 output channels. We use Tanh as the activation function. The client with text possesses a model consisting of one embedding layer with dictionary size 11658 and embedding vector size 300, two LSTM layers with input size 300, hidden size 512, and a linear layer with input size 2048 and output size 1024. The activation function is Tanh. The top model contains two linear layers: the first one has input size 1024 and output size 430 and the second one has input size 430 and output size 430. Both linear layers are followed by a Tanh activation function and one Dropout layer. %The model is trained for 30 epoch using Adam optimizer. The initial learning rate is 0.001 and is dropped by 0.1 every 10 epochs. 
The structure of the decoder is shown in Tab.~\ref{tab:purchase_decoder} containing four UpConv layers with each UpConv layer followed by a BatchNorm layer and Tanh activation function. K, S and P represent kernel size, stride size and padding respectively. %For adaptive decoder, we train it for 10 epochs per round, totaling 10$\times$30 epochs throughout VFL. We use Adam optimizer with learning rate 0.0002 and batch size is 128. For static decoder, we train it 10 epochs using Adam optimizer with learning rate 0.01 and batch size is 128.
\begin{table}[!htbp]
	\centering
	\scalebox{0.95}{
		\begin{tabular}{ c | c | c | c | c | c }
			\toprule
			Layers & Input channel & K & S & P & Output channel \\ \hline
			UpConv & 1024 & 4 & 1 & 0 & 1024 \\ \hline
			UpConv & 1024 & 4 & 2 & 1 & 512 \\ \hline
			UpConv & 512 & 4 & 2 & 1 & 256 \\ \hline
			UpConv & 256  & 4 & 2 & 1 & 3 \\ 
			\bottomrule
	\end{tabular}}
	\centering
	\caption{Decoder structure for COCO-QA}
	\label{tab:purchase_decoder}
\end{table}
\subsubsection{Purchase}
For Purchase dataset, the model structures of each client, top model and decoder are shown in Tab.~\ref{tab:purchase_model}. All of them are Linear layers. %We train the model for 20 epochs with Adam optimizer and learning rate 0.0001. For adaptive decoder, we train it for 30 epochs per round, totaling 30$\times$20 epochs throughout VFL. We use Adam optimizer with learning rate 0.0001 and batch size is 128. For static decoder, we train it for 30 epochs using Adam optimizer with learning rate 0.01 and batch size is 128.
Each client holds data with 300 attributes. And the decoder aims to reconstruct all attributes of the victim client.

\begin{table*}[!htbp]
		\centering
		\begin{tabular}{c | c | c }
			\toprule
			\multirow{2}{*}{Client model} & Client1 & Client2 \\ \cline{2-3}
			& \begin{tabular}[c]{@{}c@{}}Linear(300, 512)\\ Relu() \end{tabular} & \begin{tabular}[c]{@{}c@{}}Linear(300, 512)\\ Relu()\end{tabular} \\ \hline
			\multirow{2}{*}{Top model} & Linear(512, 256) & Linear(512, 256) \\ \cline{2-3} 
			& \multicolumn{2}{c}{\begin{tabular}[c]{@{}c@{}}Concatenate intermediate outputs\\Relu() \\ Linear(512, 100)\end{tabular}} \\ \hline
			\multicolumn{1}{c|}{Decoder model} &\multicolumn{2}{c}{\begin{tabular}[c]{@{}c@{}}Relu()\\ Linear(512, 300)\end{tabular}} \\
			\bottomrule
	\end{tabular}
	\centering
	\caption{Models for Purchase}
	\label{tab:purchase_model}
\end{table*}

\begin{table}[t]
	\centering
	\scalebox{0.95}{
		\begin{tabular}{ c | c | c | c | c | c }
			\toprule
			Layers & Input channel & K & S & P & Output channel \\ \hline
			UpConv & 5           & 4 & 1 & 0 & 8      \\ \hline
			UpConv & 8           & 4 & 2 & 1 & 4      \\ \hline
			Conv   & 4           & 4 & 2 & 1 & 8      \\ \hline
			Conv   & 8           & 4 & 1 & 0 & 14     \\ 
			\bottomrule
	\end{tabular}}
	\centering
	\caption{Decoder structure for Credit}
	\label{tab:credit_decoder}
\end{table}
\begin{table}[t]
	\centering
	\scalebox{0.90}{
		\begin{tabular}{c | c | c }
			\toprule
			\multirow{2}{*}{Client model} & Client1 & Client2 \\ \cline{2-3}
			& \begin{tabular}[c]{@{}c@{}}Linear(5,32)\\ Relu()\\ Linear(32,64)\\ Relu()\end{tabular} & \begin{tabular}[c]{@{}c@{}}Linear(6,32)\\ Relu()\\ Linear(32,64)\\ Relu() \end{tabular} \\ \hline
			\multirow{2}{*}{Top model} & Linear(64, 32) & Linear(64, 32) \\ \cline{2-3} 
			& \multicolumn{2}{c}{\begin{tabular}[c]{@{}c@{}}Concatenate intermediate outputs\\ ReLU() \\ Linear(64, 2) \\ Sigmoid()\end{tabular}} \\ \hline
			\multicolumn{1}{c|}{Decoder model} &\multicolumn{2}{c}{\begin{tabular}[c]{@{}c@{}}Linear(64, 32) \\ Relu()\\ Linear(32, 9)\end{tabular}} \\
			\bottomrule
	\end{tabular}}
	\centering
	\caption{Models for Adult}
	\label{tab:adult_model}
\end{table}
\subsubsection{Credit}
For Credit dataset, the model structures of each client and top model are shown in Tab.~\ref{tab:credit_model} which are Linear layers. Each client hold the data with 14 attributes. The decoder is shown in Tab.~\ref{tab:credit_decoder} and each UpConv and Conv layer are followed by a BatchNorm layer and a Tahn activation function. K, S and P represent kernel size, stride size and padding respectively.
%We train the model for 20 epochs with Adam optimizer and learning rate 0.0001. The structure of decoder is shown in Tab.~\ref{tab:credit_decoder} and each UpConv and Conv layer are followed by a BatchNorm layer and a Tahn activation function. K, S and P represent kernel size, stride size and padding respectively. %For adaptive decoder, we train it for 30 epochs per round, totaling 30$\times$20 throughout VFL. We use Adam optimizer with learning rate 0.0001 and batch size is 128. For static decoder, we train it for 15 epochs using Adam optimizer with learning rate 0.01 and batch size is 128.
\begin{table*}[!htbp]
	\scalebox{0.98}{
		\centering
		\begin{tabular}{c | c | c }
			\toprule
			\multirow{2}{*}{Client model} & Client1 & Client2 \\ \cline{2-3}
			& \begin{tabular}[c]{@{}c@{}}Linear(14, 5)\\ BatchNorm() \end{tabular} & \begin{tabular}[c]{@{}c@{}}Linear(14, 5)\\ BatchNorm() \end{tabular} \\ \hline
			\multirow{2}{*}{Top model} & Linear(5, 5) & Linear(5, 5) \\ \cline{2-3} 
			& \multicolumn{2}{c}{\begin{tabular}[c]{@{}c@{}}Concatenate intermediate outputs\\BatchNorm() \\ Linear(10, 1) \\ Sigmoid()\end{tabular}} \\ 
			\bottomrule
		\end{tabular}
		\centering}
	\caption{Models for Credit}
	\label{tab:credit_model}
\end{table*}

\subsubsection{Adult}
For Adult dataset, the model structure of each client, top model and decoder are shown in Tab.~\ref{tab:adult_model} and all of them are Linear layers. One client holds 5 attributes and the other holds 6 attributes. The decoder aims to reconstruct one certain attribute and the output channel of the last Linear layer depends on the number of classes of the attribute. %We train the model for 30 epochs with Adam optimizer and learning rate 0.0001. For adaptive decoder, we train it for 100 epochs per round, totaling 100$\times$30 epochs overall. We use Adam optimizer with learning rate 0.0001 and batch size is 128. For static decoder, we train it for 100 epochs using Adam optimizer with learning rate 0.0001 and batch size is 128.

\subsection{Hyperparameters}
The hyperparameters for each dataset is shown in Tab.~\ref{tab:hyper}. All models are trained using Adam optimizer. Let's explain COCO-QA for example. The vertical model including local model for each client and the top model is trained for 30 epoch using Adam optimizer and the batch size is 100. The initial learning rate is 0.001 and dropped by 0.1 every 10 epochs. For static attack, we train static decoder 10 epochs using Adam optimizer with learning rate 0.01 and batch size is 128. For adaptive attack, we train adaptive decoder for 10 epochs per round, totaling 10$\times$30 epochs throughout vertical federated learning. We use Adam optimizer with learning rate 0.0002 and batch size is 128 for adaptive attack. 
\begin{table*}[h]
	\centering
	\scalebox{0.85}{
	\begin{tabular}{ c | c | c | c | c | c | c | c | c | c }
		\toprule
		\multirow{2}{*}{$\sim$} & \multicolumn{3}{c|}{Vertical federated learning}  & \multicolumn{3}{c|}{Static attack} & \multicolumn{3}{c}{Adaptive attack} \\ \cline{2-10} 
		& Lr & Epoch number & Batch size & Lr & Epoch number & Batch size & Lr& Epoch number  & Batch size  \\ \hline
		Purchase & 0.0001 & 20 & 32 & 0.01 & 30 & 128 & 0.0001 & 30$\times$20 & 128 \\ \hline
		Adult & 0.0001 & 30 & 32 & 0.0001 & 100 & 128 & 0.0001 & 100$\times$30 & 128 \\ \hline
		COCO-QA & \begin{tabular}[c]{@{}c@{}}0.001\\ $\times$0.1 every 10 epochs\end{tabular} & 30  & 100 & 0.01 & 10 & 128 & 0.0002  & 10$\times$30 & 128 \\ \hline
		Credit & 0.0001 & 20 & 128 & 0.01 & 15 & 128 & 0.0001 & 30$\times$20 & 128 \\ \bottomrule
	\end{tabular}}
	\centering
	\caption{Hyperparameters for each dataset. Lr is the learning rate.}
	\label{tab:hyper}
\end{table*}
\section{Metrics and Loss Function}
\subsection{Accuracy}
We use AUC to measure the accuracy for Credit because the dataset is highly unbalanced with only 0.172\% positive instances. For other datasets, we use the normal accuracy which equals to the number of correct predictions divided by the total instances. For binary classification, we use BCE as loss function and for multi-classification, we use CrossEntropy as loss function.

\subsection{Privacy}
For classification attack, there are five privacy metrics:
\begin{equation}
\text{recall} = \frac{\text{TP}}{\text{TP+FN}},
\end{equation}
\begin{equation}
\text{error rate} = \frac{\text{FP+FN}}{\text{TP+TN+FP+FN}},
\end{equation}
\begin{equation}
\text{precision} = \frac{\text{TP}}{\text{TP+FP}},
\end{equation}
\begin{equation}
\text{f1-score} = \frac{2\times \text{recall} \times \text{precison}}{\text{recall} + \text{precision}}.
\end{equation}
High error rate, low recall, low precision, or low f1-score means a high privacy level. For regression attack, we use MSE as the privacy metrics and higher MSE means a higher privacy level.

The privacy loss $g(\cdot)$ is a non-increasing function of reconstruction loss $l(\cdot)$. We have three choices: $g(\cdot) = -l(\cdot)$, $g(\cdot) = \frac{1}{l(\cdot)}$ and $g(\cdot) = e^{-l(\cdot)}$. For regression attack, $l(\cdot)$ is MSE and for classification attack, $l(\cdot)$ is BCE or CrossEntropy.

\section{Results}
\subsection{Attack}
Fig.~\ref{fig:all_attack_1}, Fig.~\ref{fig:all_attack_2} and 
Fig.~\ref{fig:all_attack_3} are the results for Purchase using different privacy metrics including error rate, precision and f1-score. The results are consistent across different metrics. 
Fig.~\ref{fig:all_attack_6} is the result for COCO-QA with a different privacy metric: f1-score, which is also a consistent result.
Fig.~\ref{fig:all_attack_4} and Fig.~\ref{fig:all_attack_5} show the static attack and adaptive attack performance throughout the vertical federated learning for Credit.
Fig.~\ref{fig:all_attack_7} and Fig.~\ref{fig:all_attack_8} are for Adult.

On Purchase (Fig.~\ref{fig:all_attack_1},~\ref{fig:all_attack_2},~\ref{fig:all_attack_3}) and COCO-QA (Fig.~\ref{fig:all_attack_6}), the adaptive attack has better performance than the static one which is consistent with what we have discussed before. And we think it is attributed to more data collected and the attack can transfer across features obtained in different rounds. 

On Credit (Fig.~\ref{fig:all_attack_4},~\ref{fig:all_attack_5}) and Adult (Fig.~\ref{fig:all_attack_7}, ~\ref{fig:all_attack_8}), the static attack performs better than the adaptive attack. The convergent MSE value of adaptive attack for Credit is $3.43\times10^{-4}$ which is higher than static attack. It may be because the training data in each batch lacks similarity and the decoder cannot transfer across them.

The static attack performance for Purchase (Fig.~\ref{fig:all_attack_1},~\ref{fig:all_attack_2},~\ref{fig:all_attack_3}) and Credit (Fig.~\ref{fig:all_attack_4}) gets slightly worse which is consistent with what we have discussed before, indicating the features learned to be less revealing towards the end of training. Interestingly, on Adult (Fig.~\ref{fig:all_attack_7}), the static decoder gets stronger with the training in vertical federated learning. It may be because the accuracy and privacy objectives are contradictory in nature. In this case, it is not possible to learn in a privacy-preserving way without accuracy decline. 

\begin{figure}[!htbp]
	\centering  %图片全局居中
	\subfigure[Purchase, error rate]{
		\label{fig:all_attack_1}
		\includegraphics[width=0.22\textwidth]{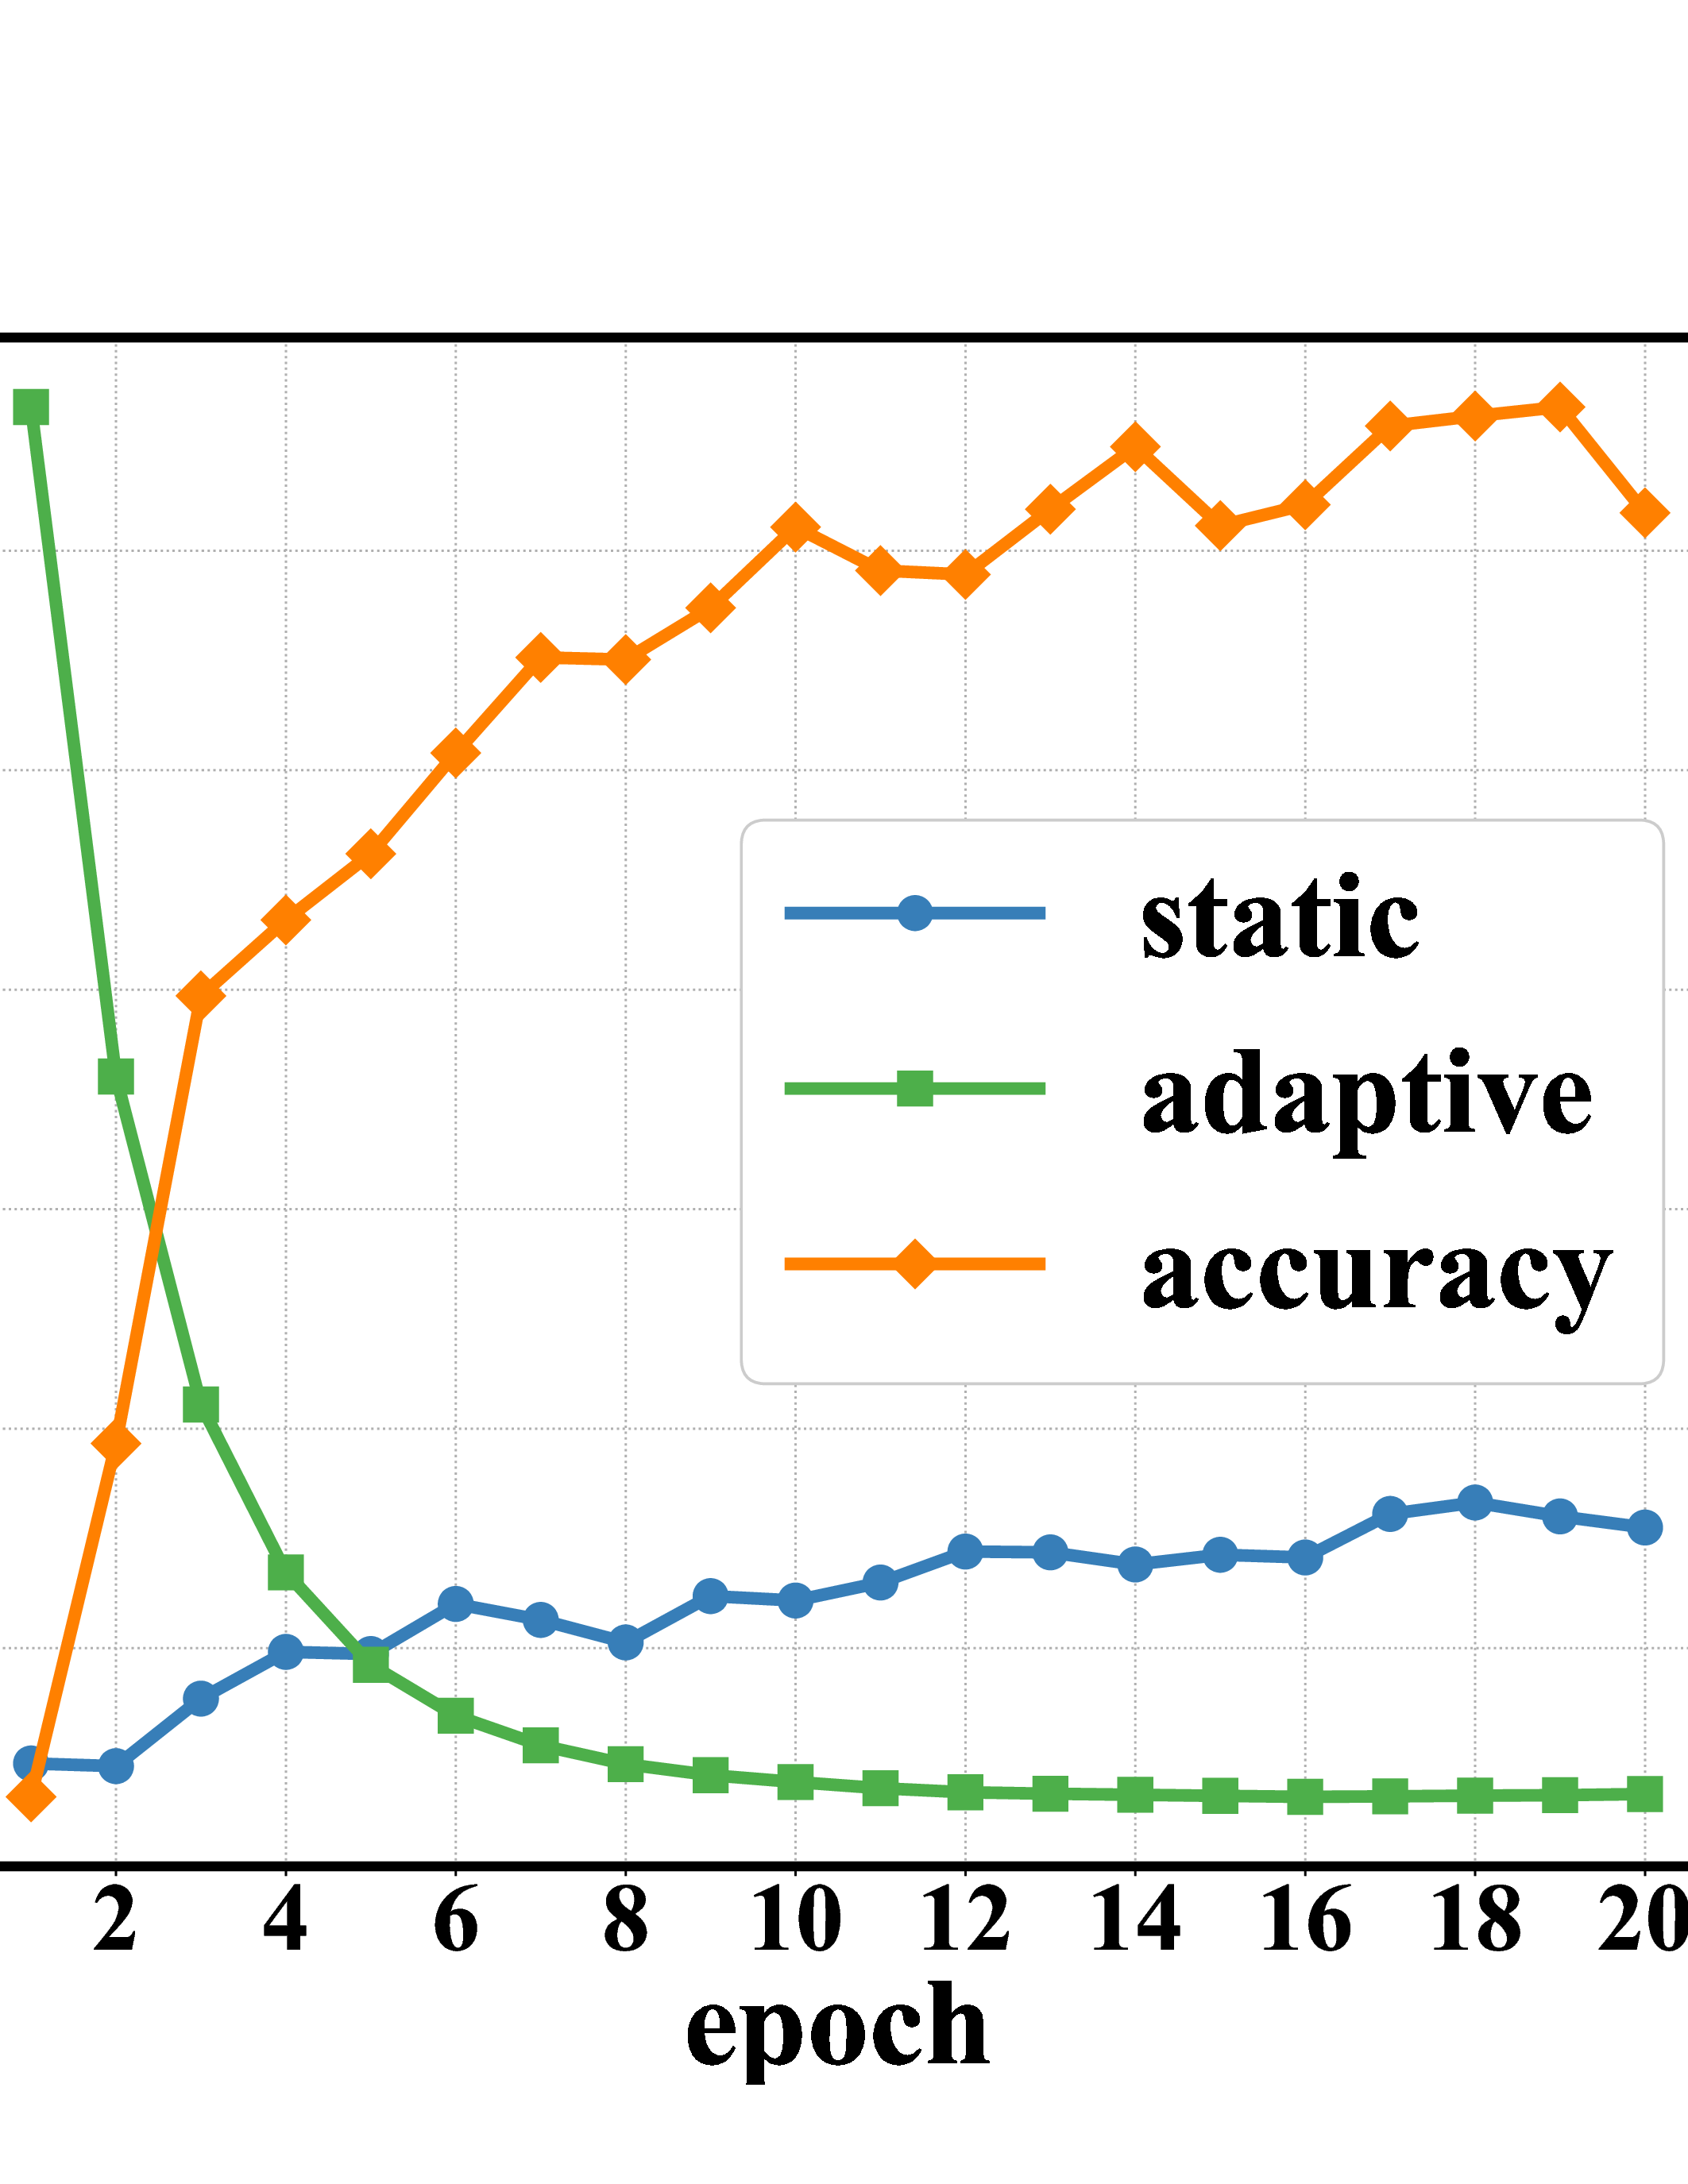}}
	\subfigure[Purchase, precision]{
		\label{fig:all_attack_2}
		\includegraphics[width=0.22\textwidth]{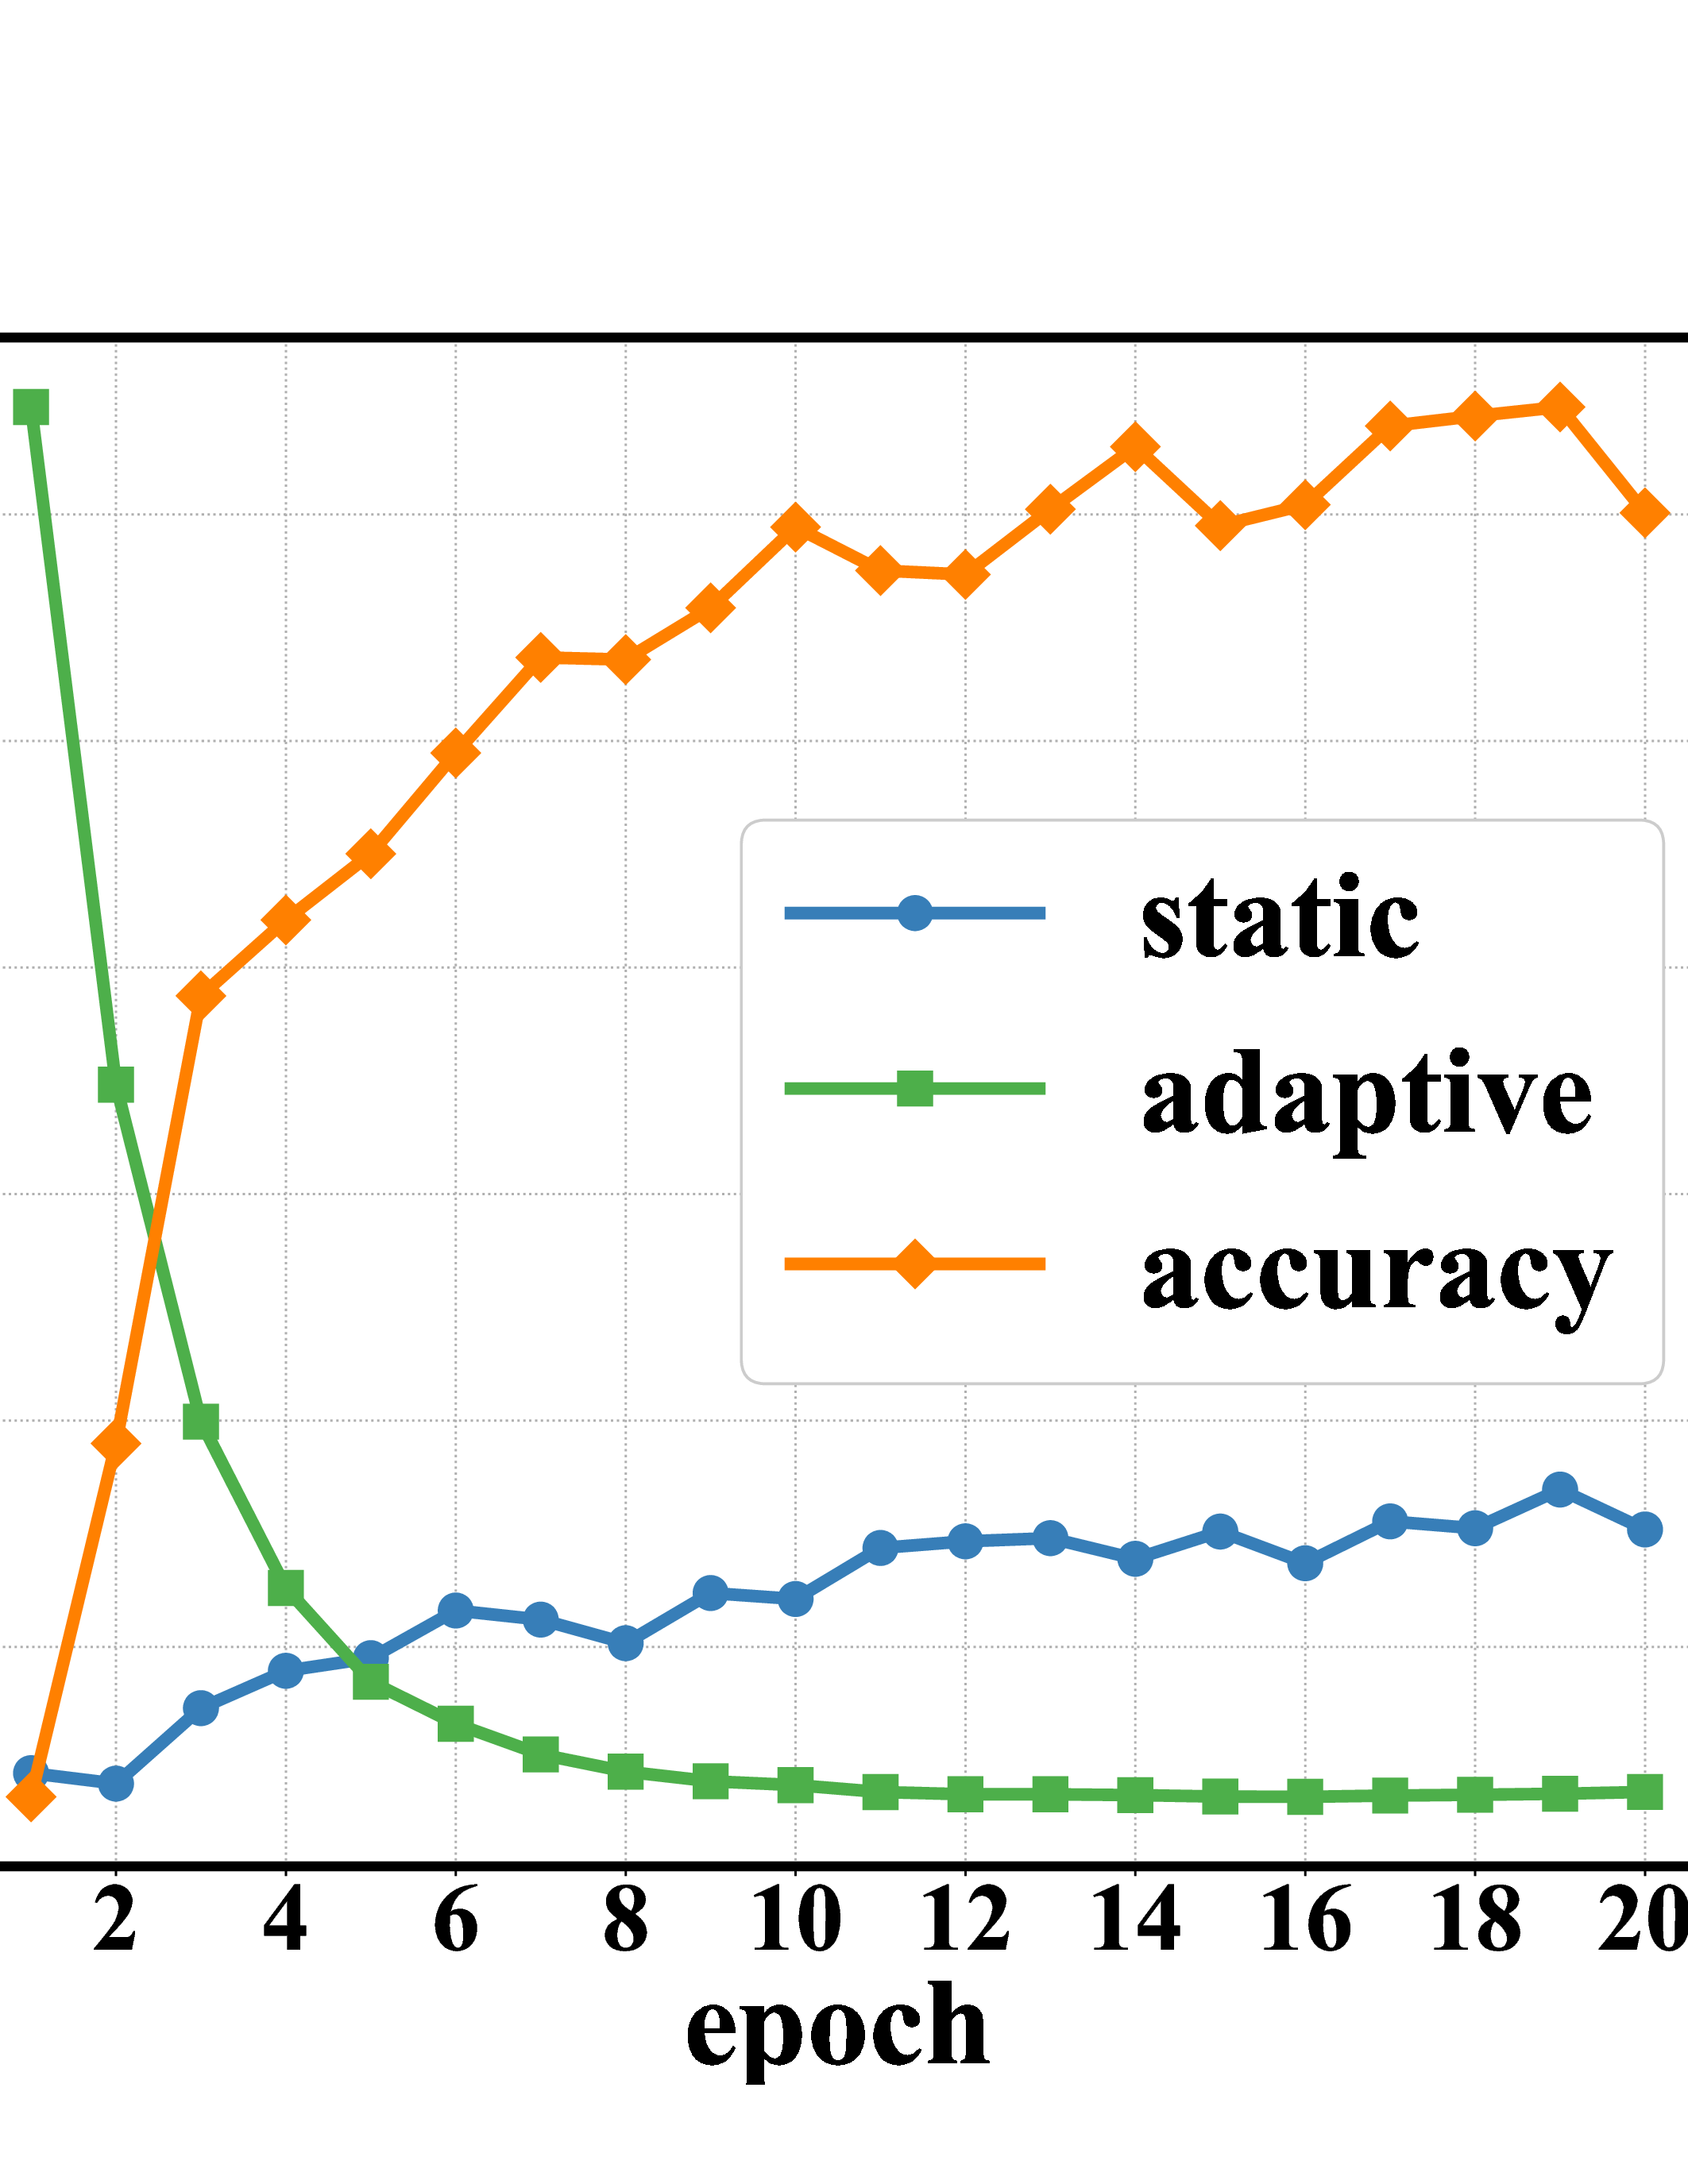}}
	\subfigure[Purchase, f1-score]{
		\label{fig:all_attack_3}
		\includegraphics[width=0.22\textwidth]{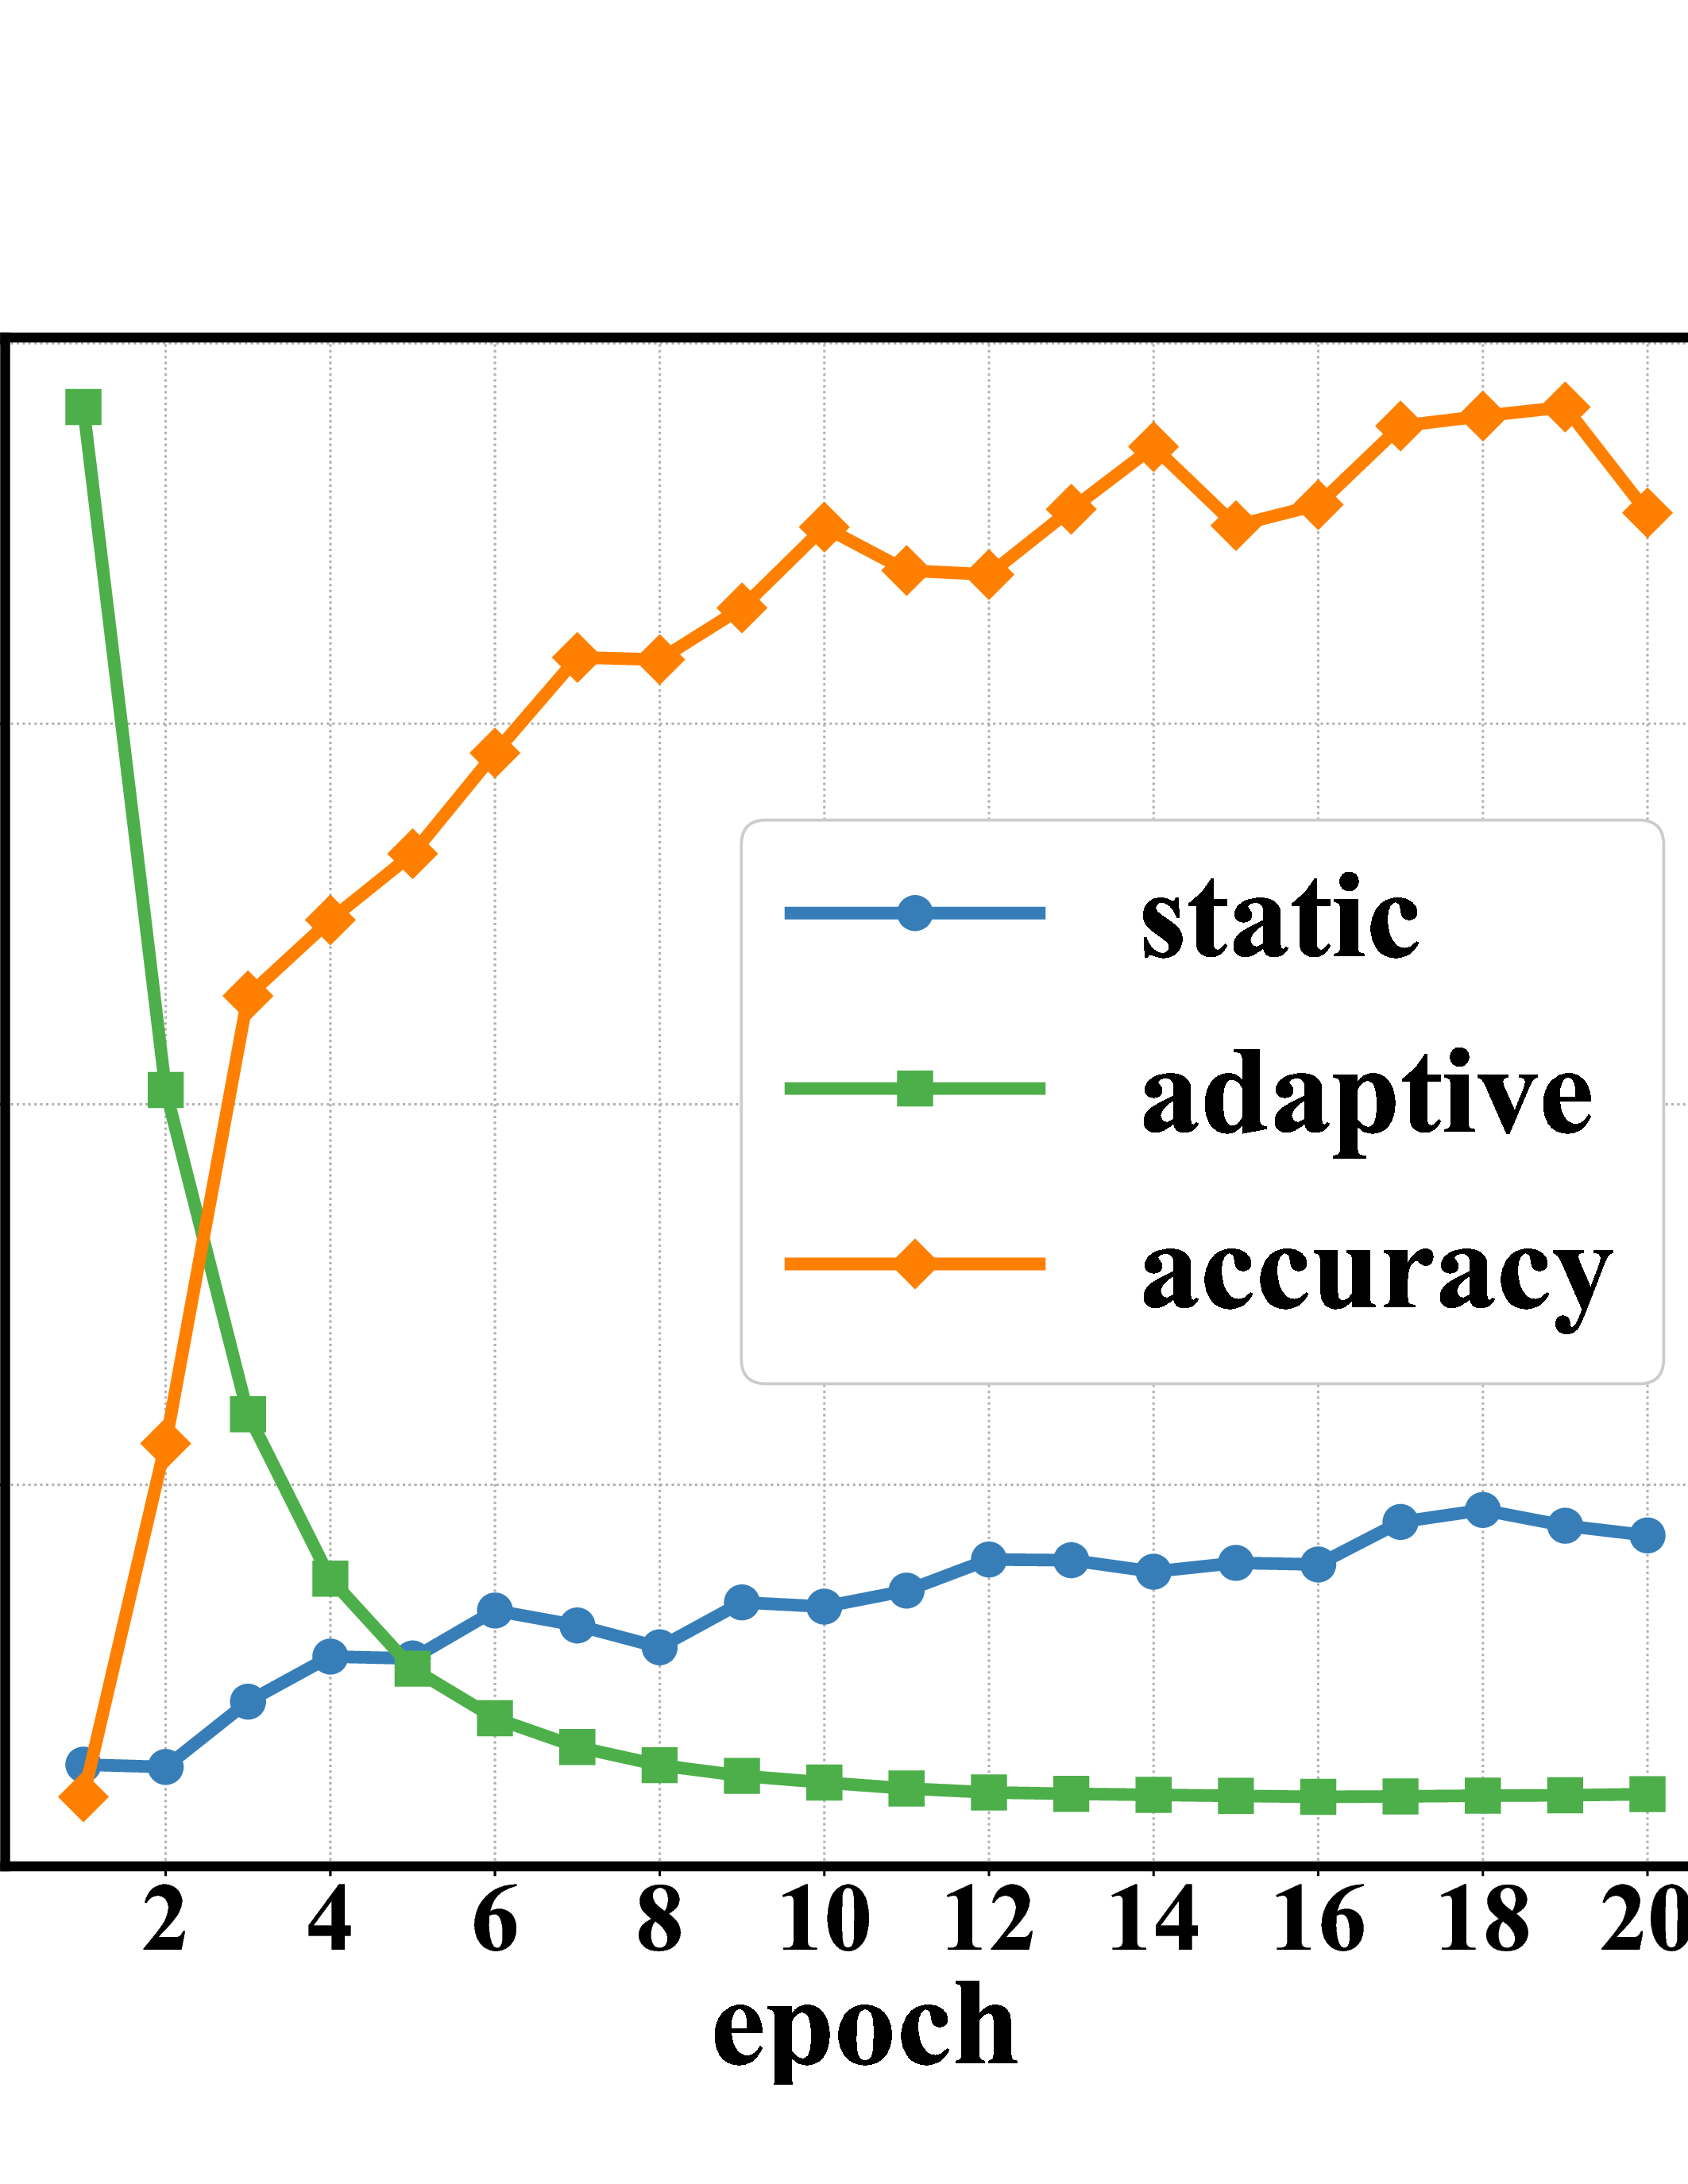}}
	\subfigure[COCO-QA]{
		\label{fig:all_attack_6}
		\includegraphics[width=0.22\textwidth]{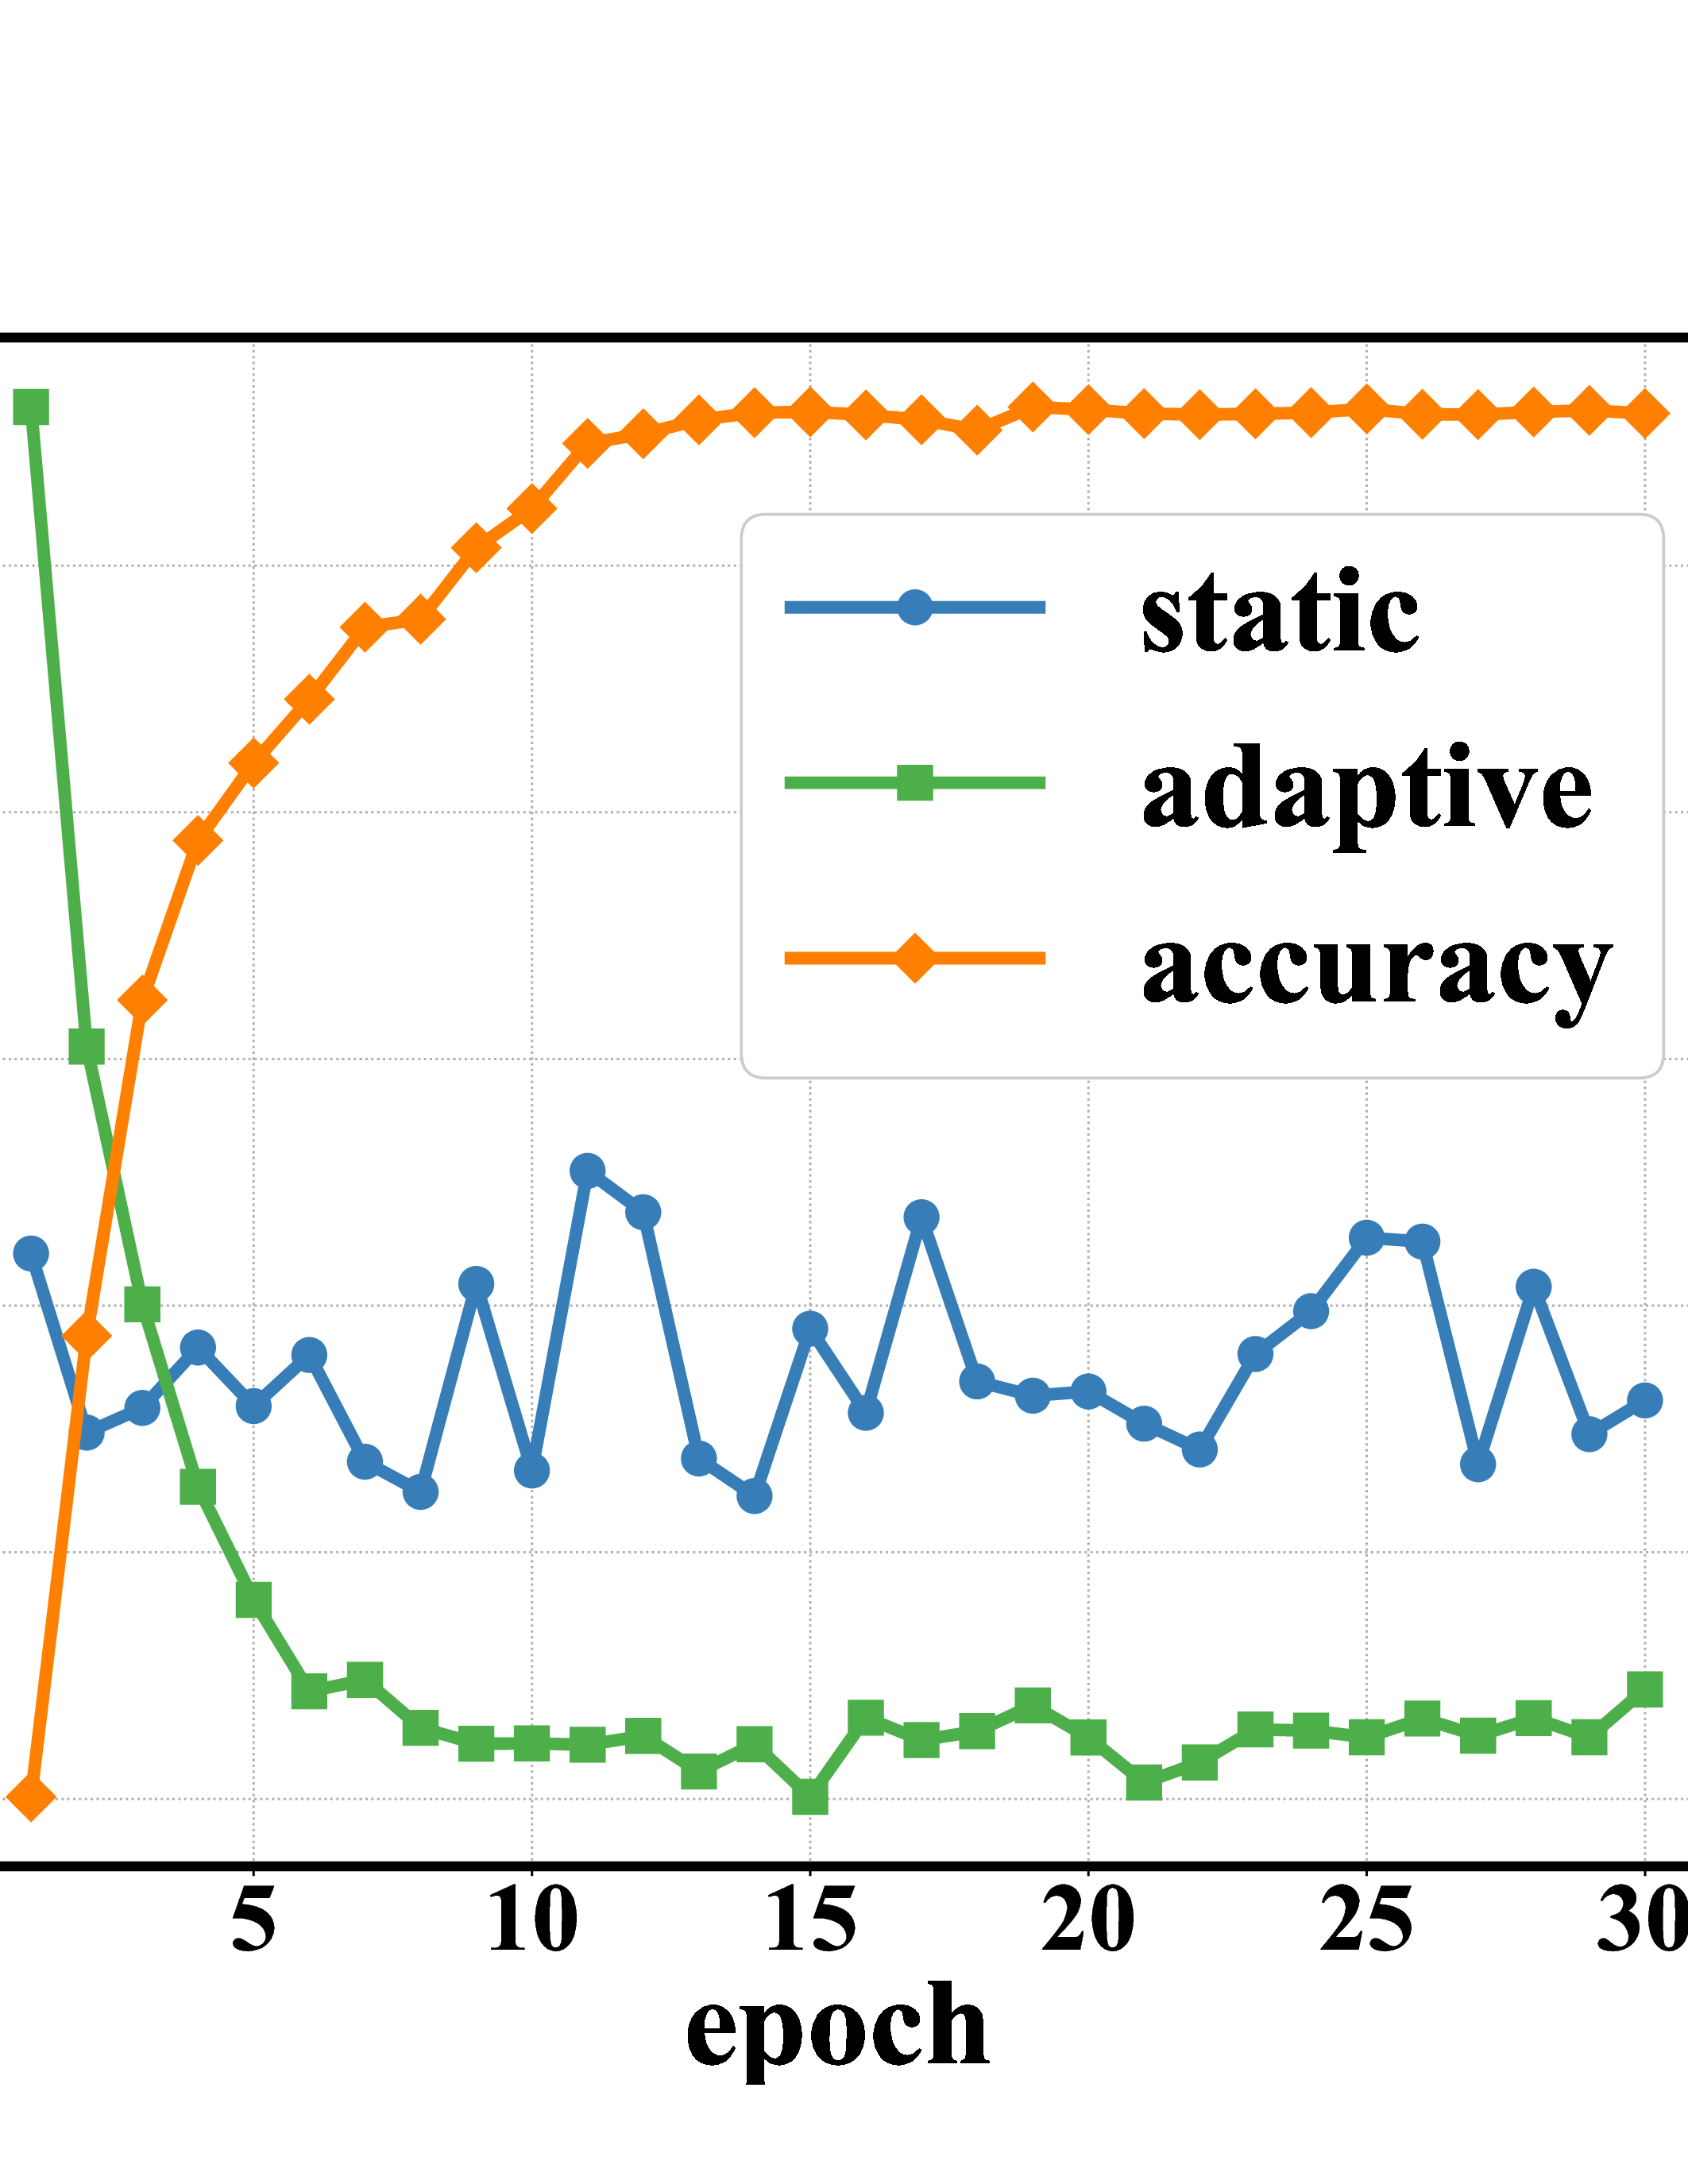}}
	\subfigure[Credit, static attack]{
		\label{fig:all_attack_4}
		\includegraphics[width=0.22\textwidth]{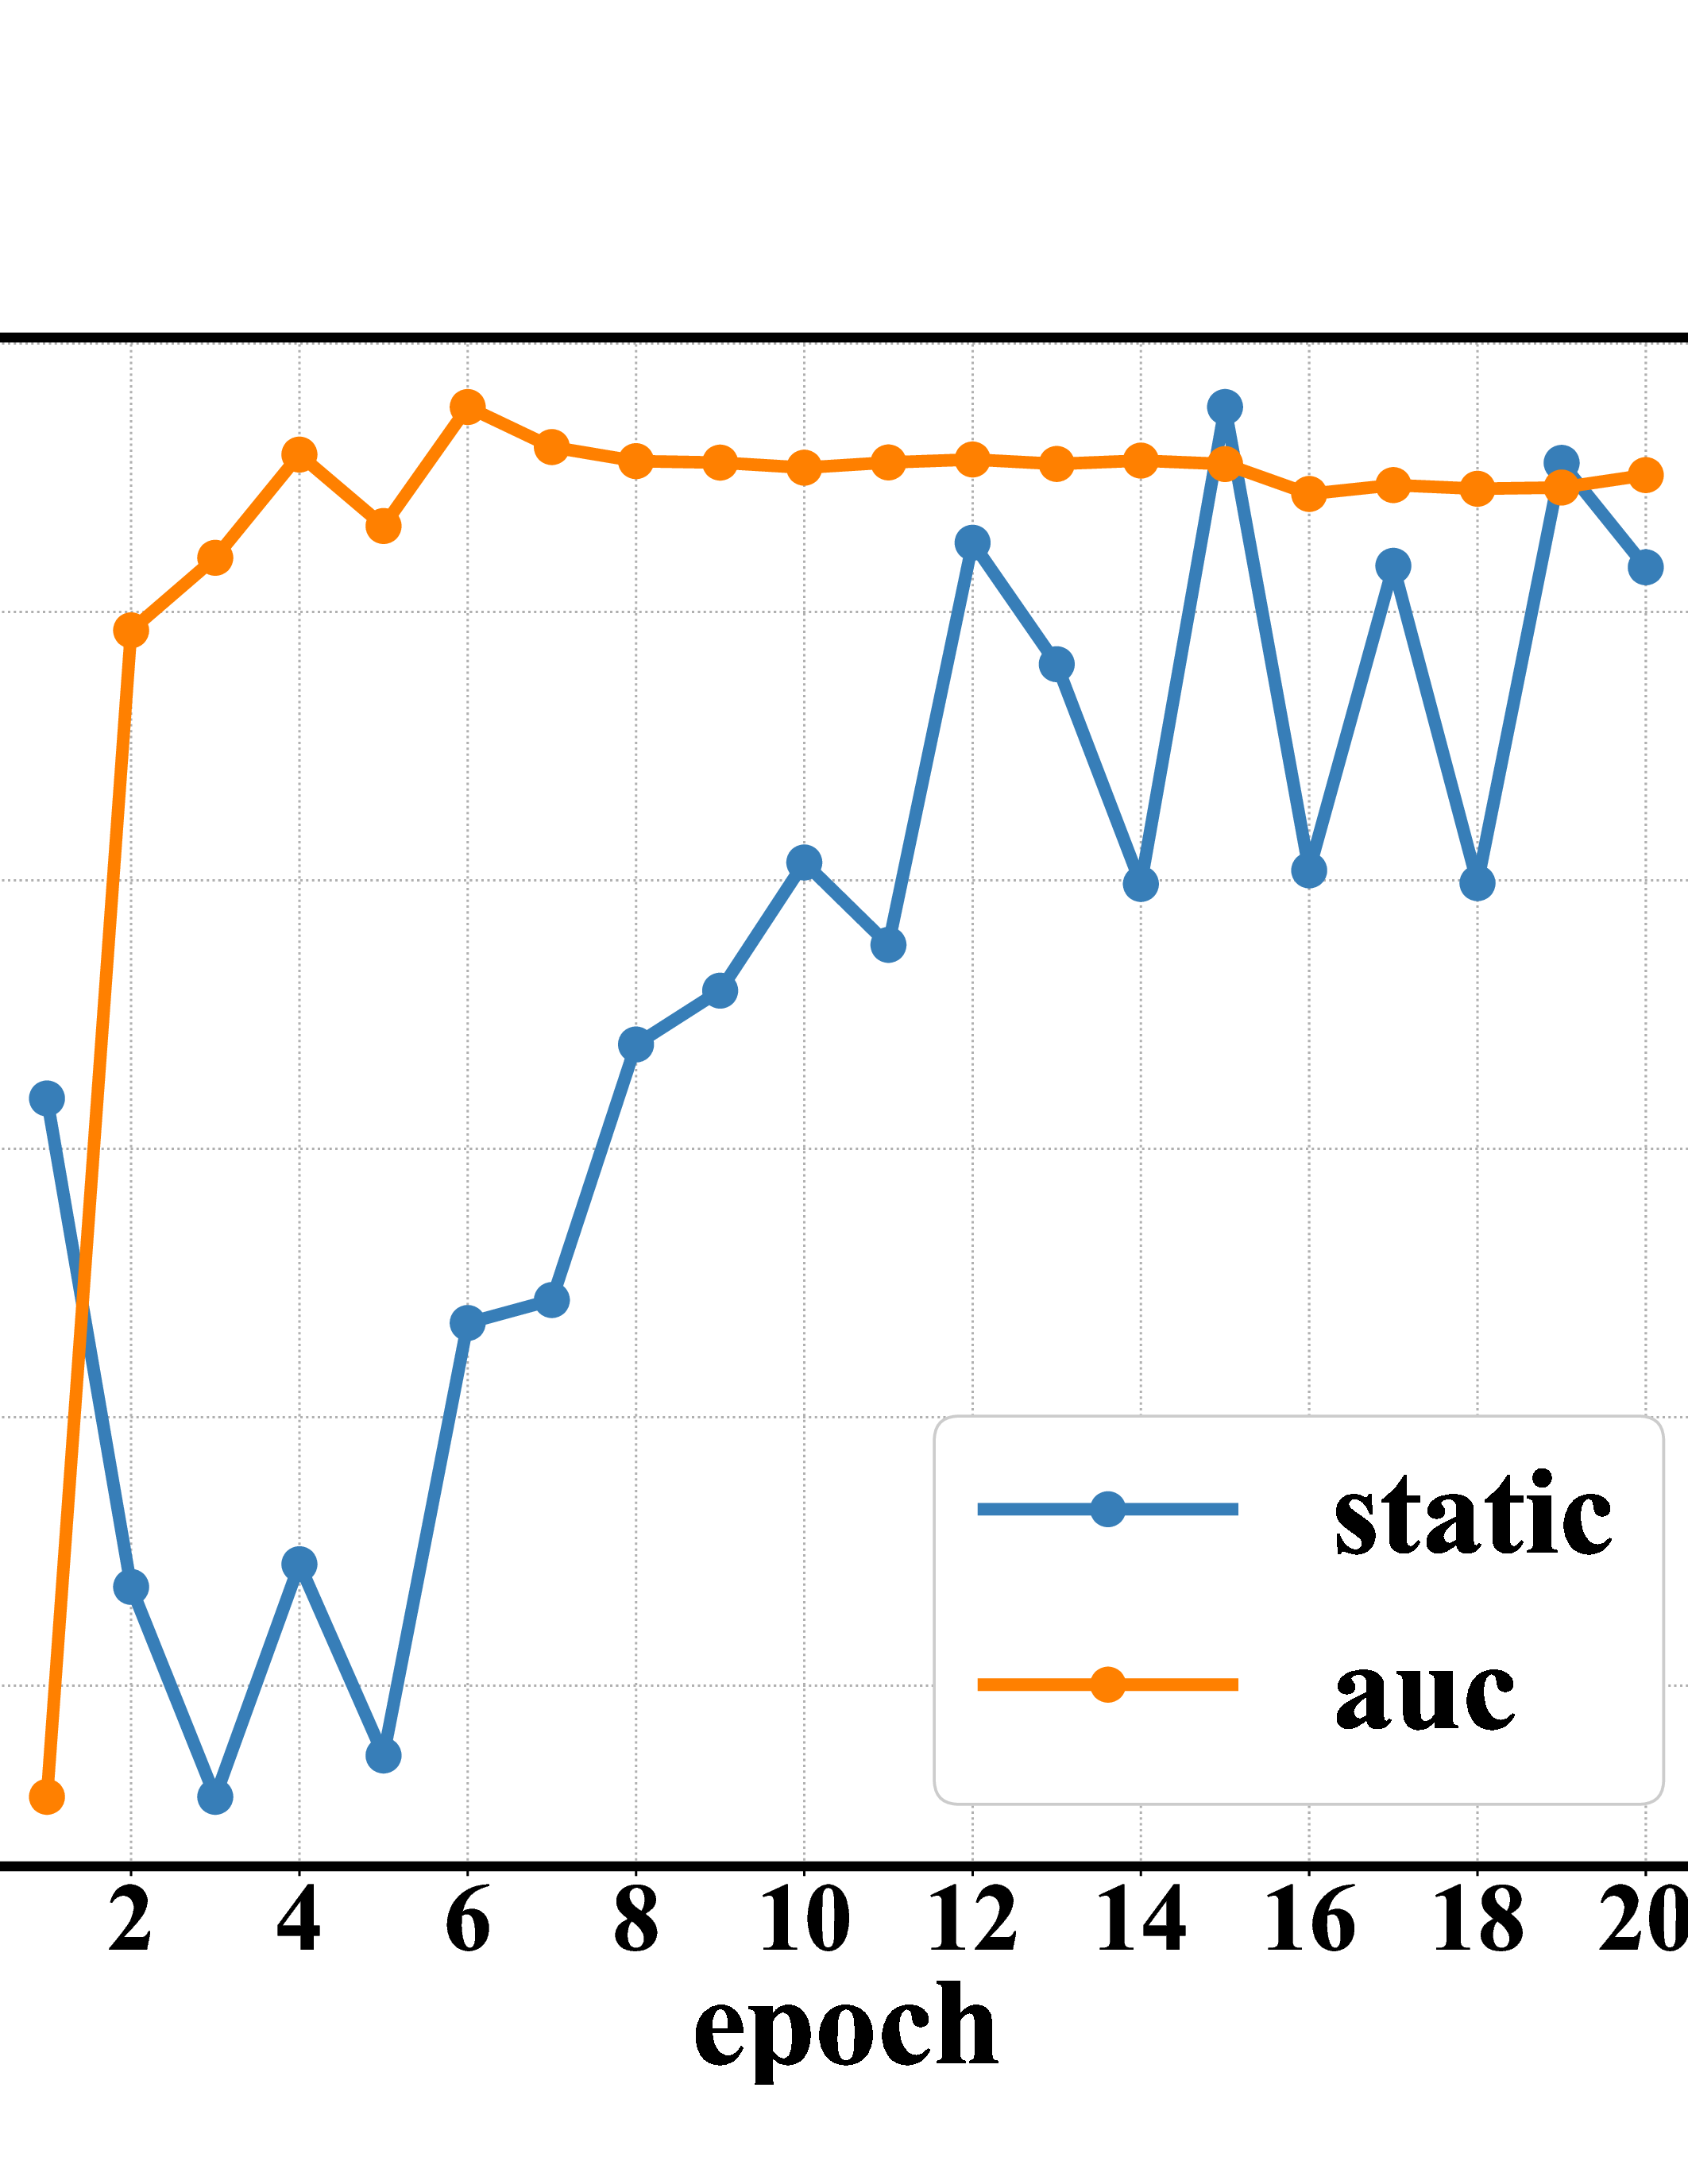}}
	\subfigure[Credit, adaptive attack]{
		\label{fig:all_attack_5}
		\includegraphics[width=0.22\textwidth]{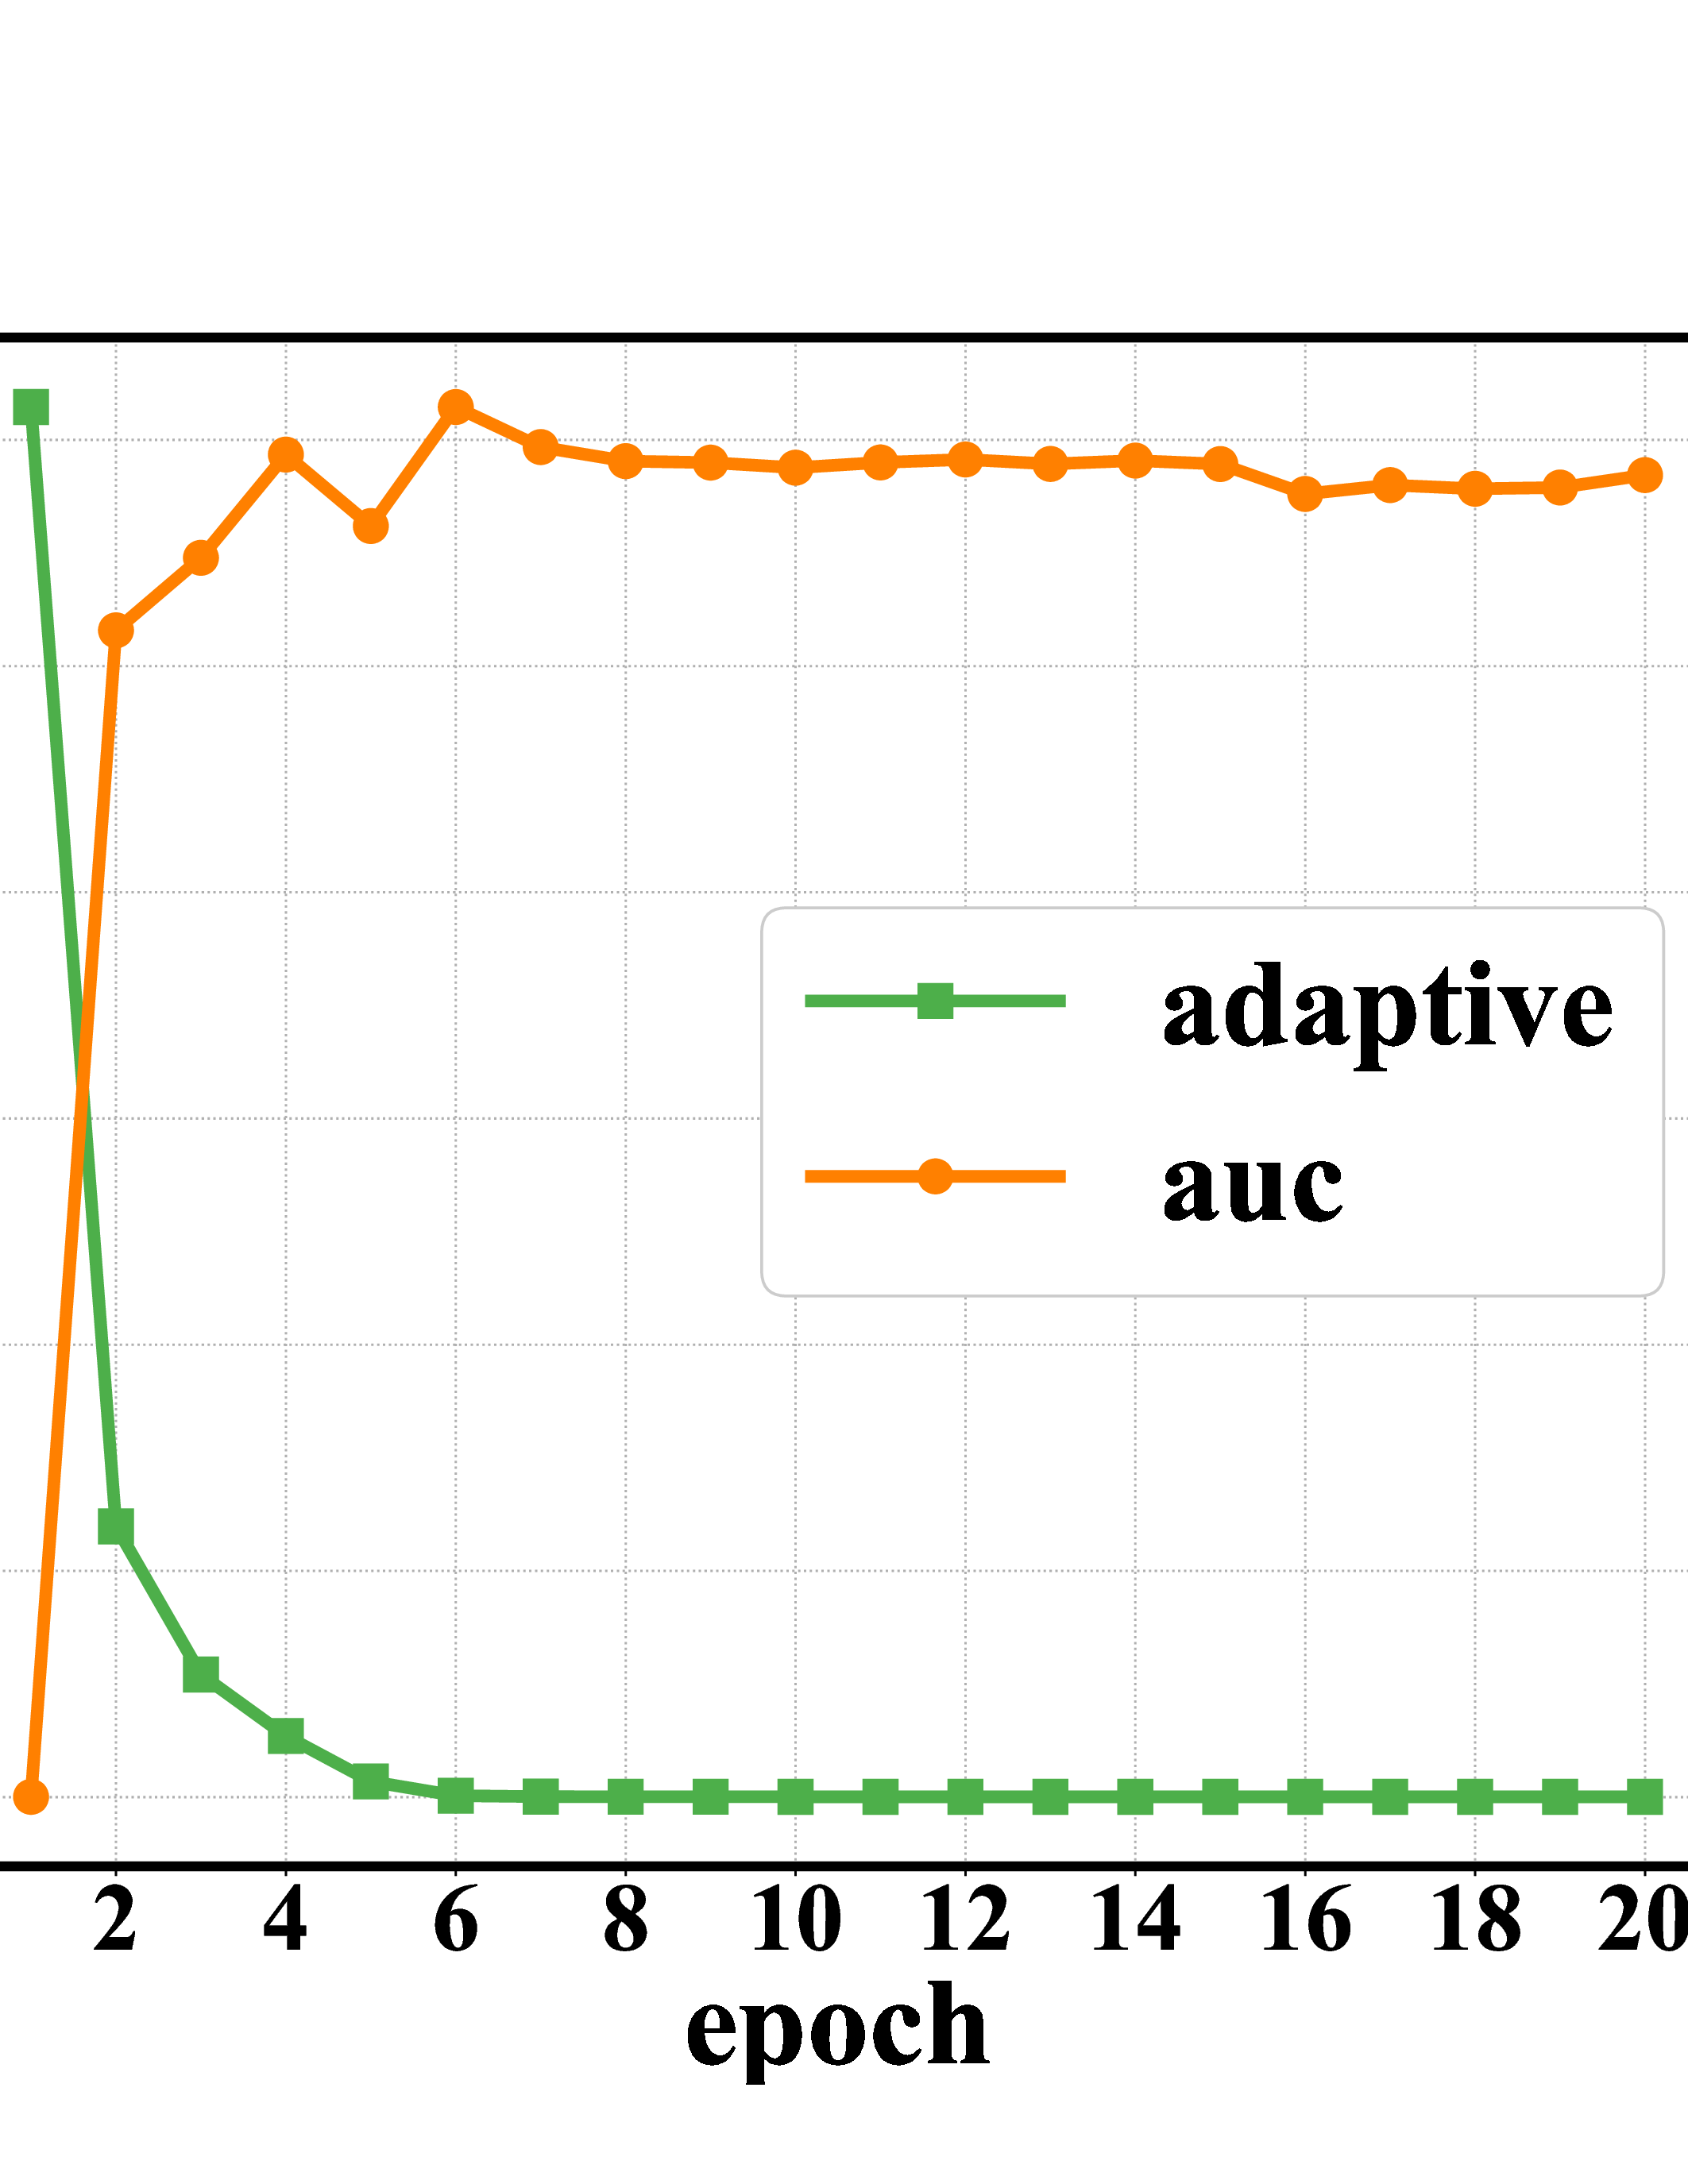}}
	\subfigure[Adult, static attack]{
		\label{fig:all_attack_7}
		\includegraphics[width=0.22\textwidth]{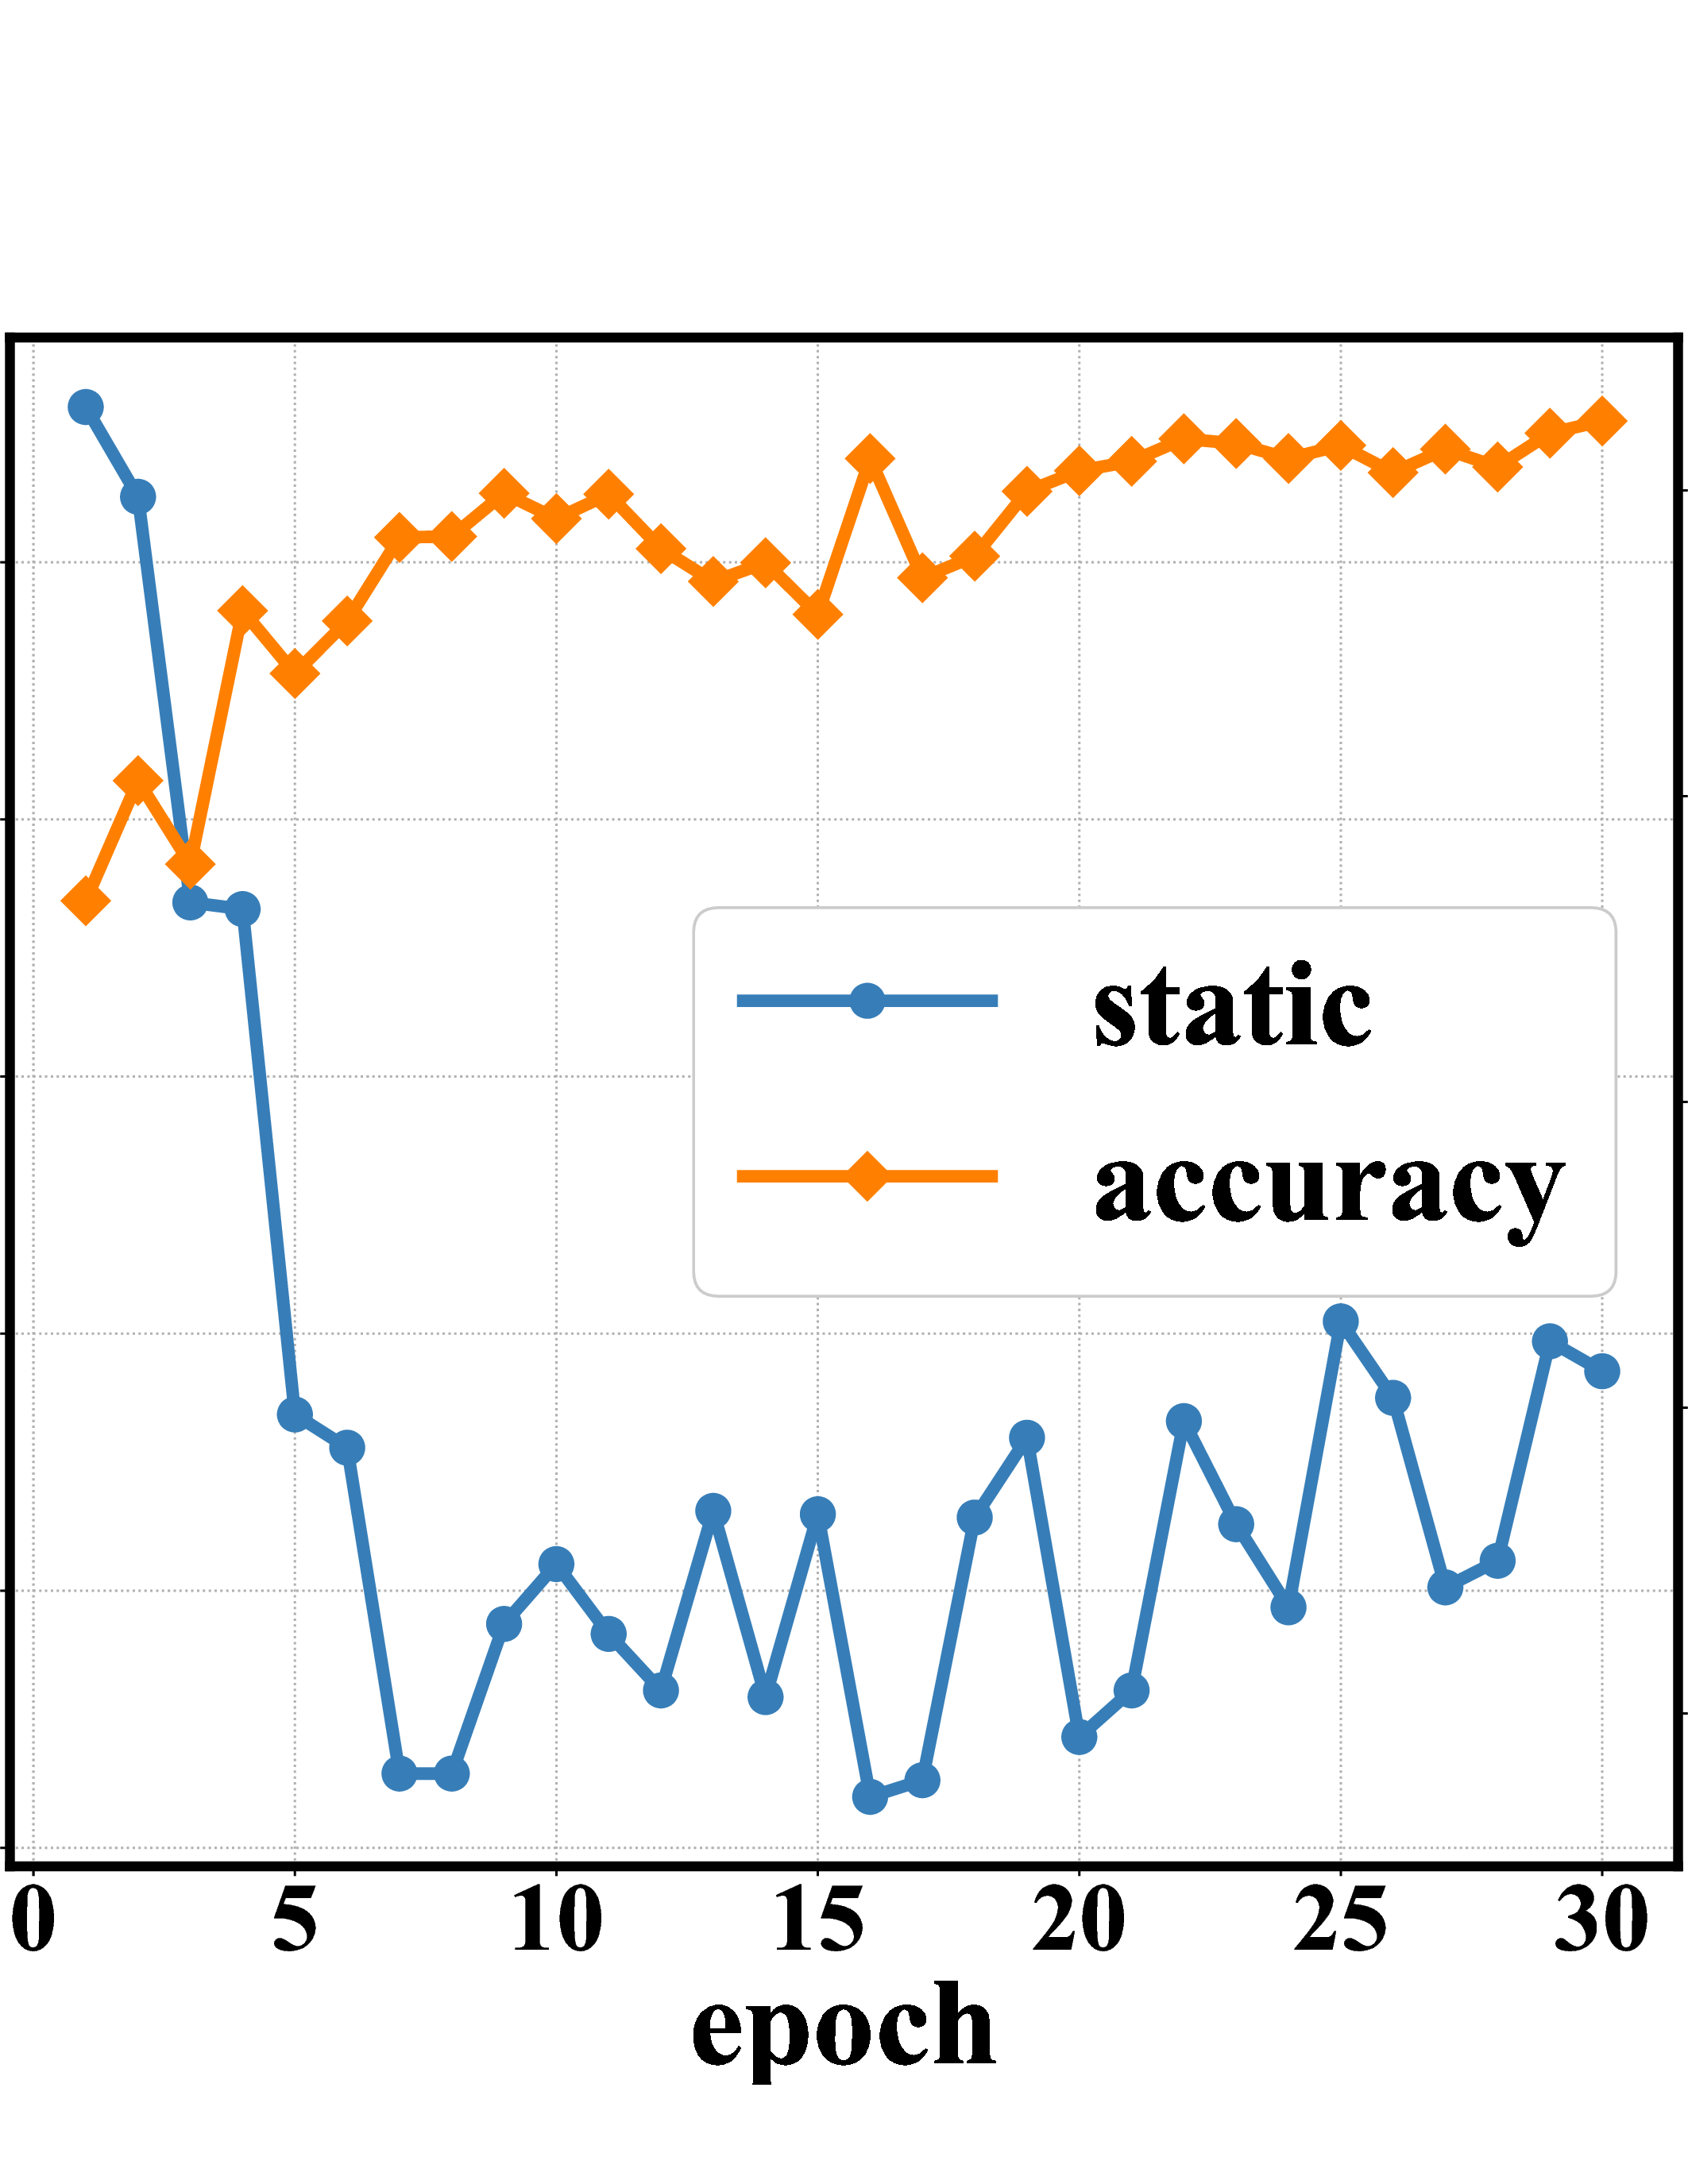}}
	\subfigure[Adult, adaptive attack]{
		\label{fig:all_attack_8}
		\includegraphics[width=0.22\textwidth]{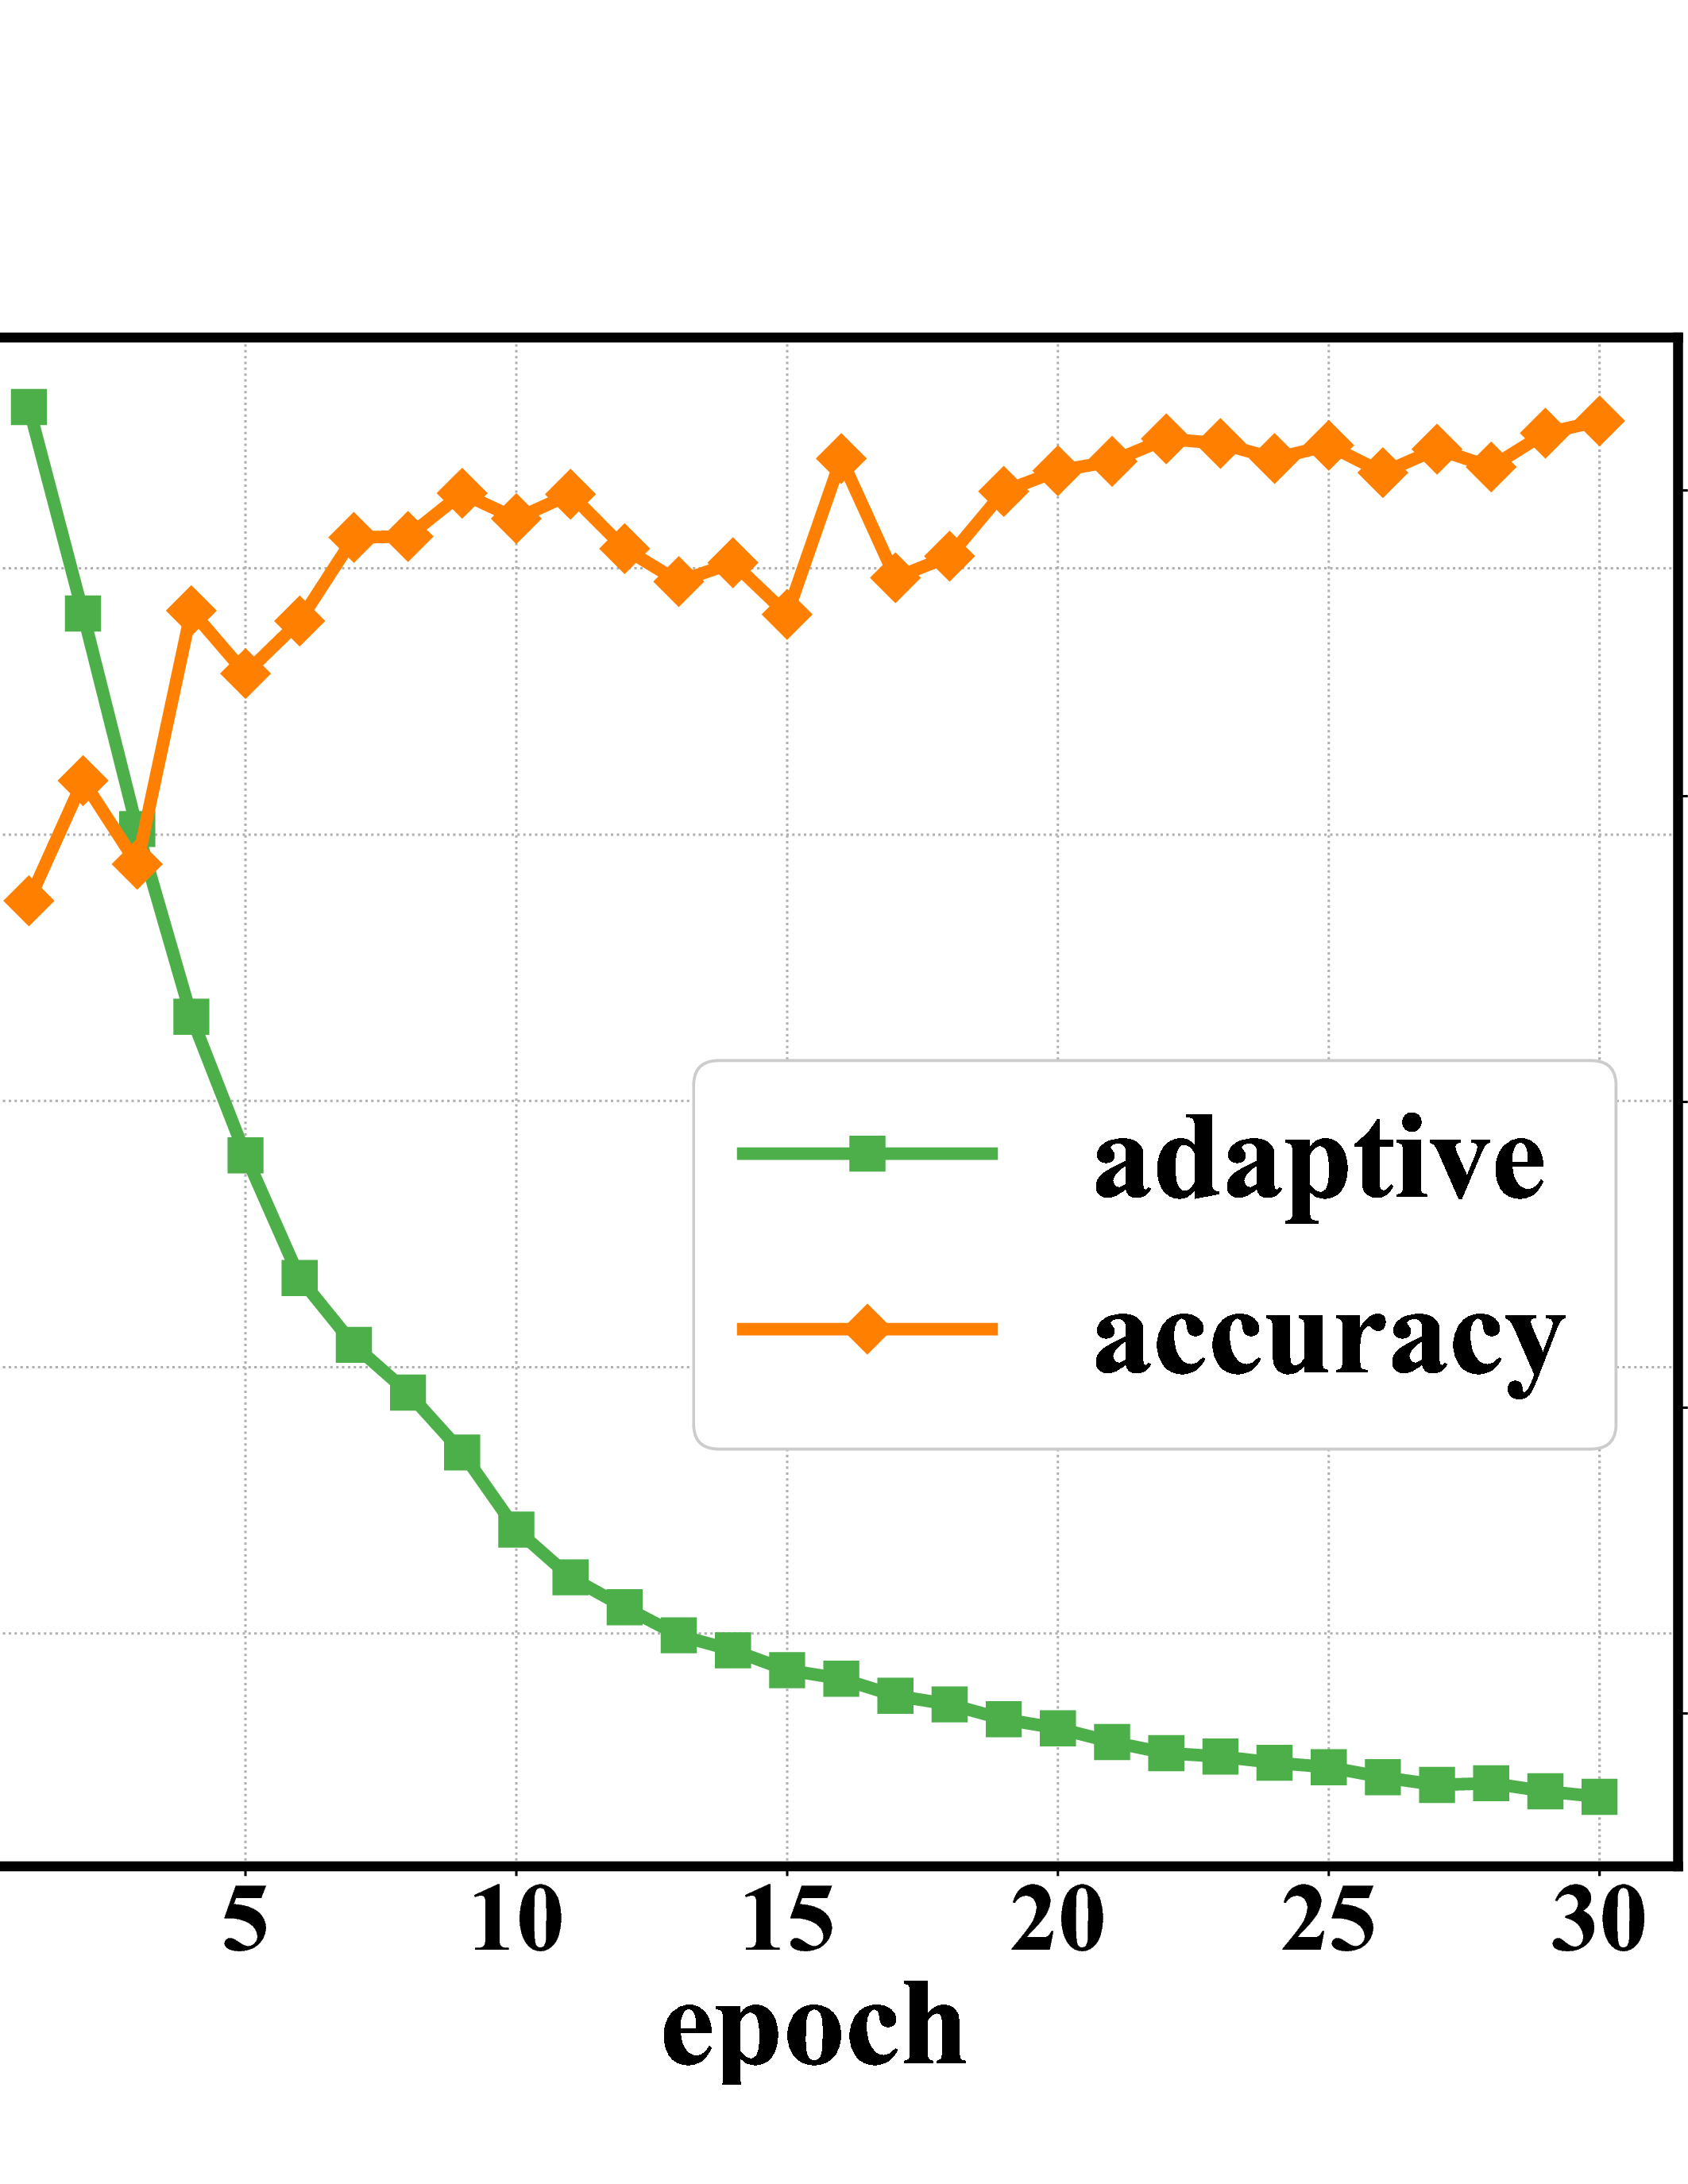}}
	\caption{Attack performance and accuracy of each epoch during VFL. Default poison ratio $\alpha=0.05$.}
	\label{fig:all_attack}
\end{figure}
\begin{figure}[h]
	\centering  %图片全局居中
	\subfigure[Purchase, error rate]{
		\label{fig:all_poison_ratio1}
		\includegraphics[width=0.22\textwidth]{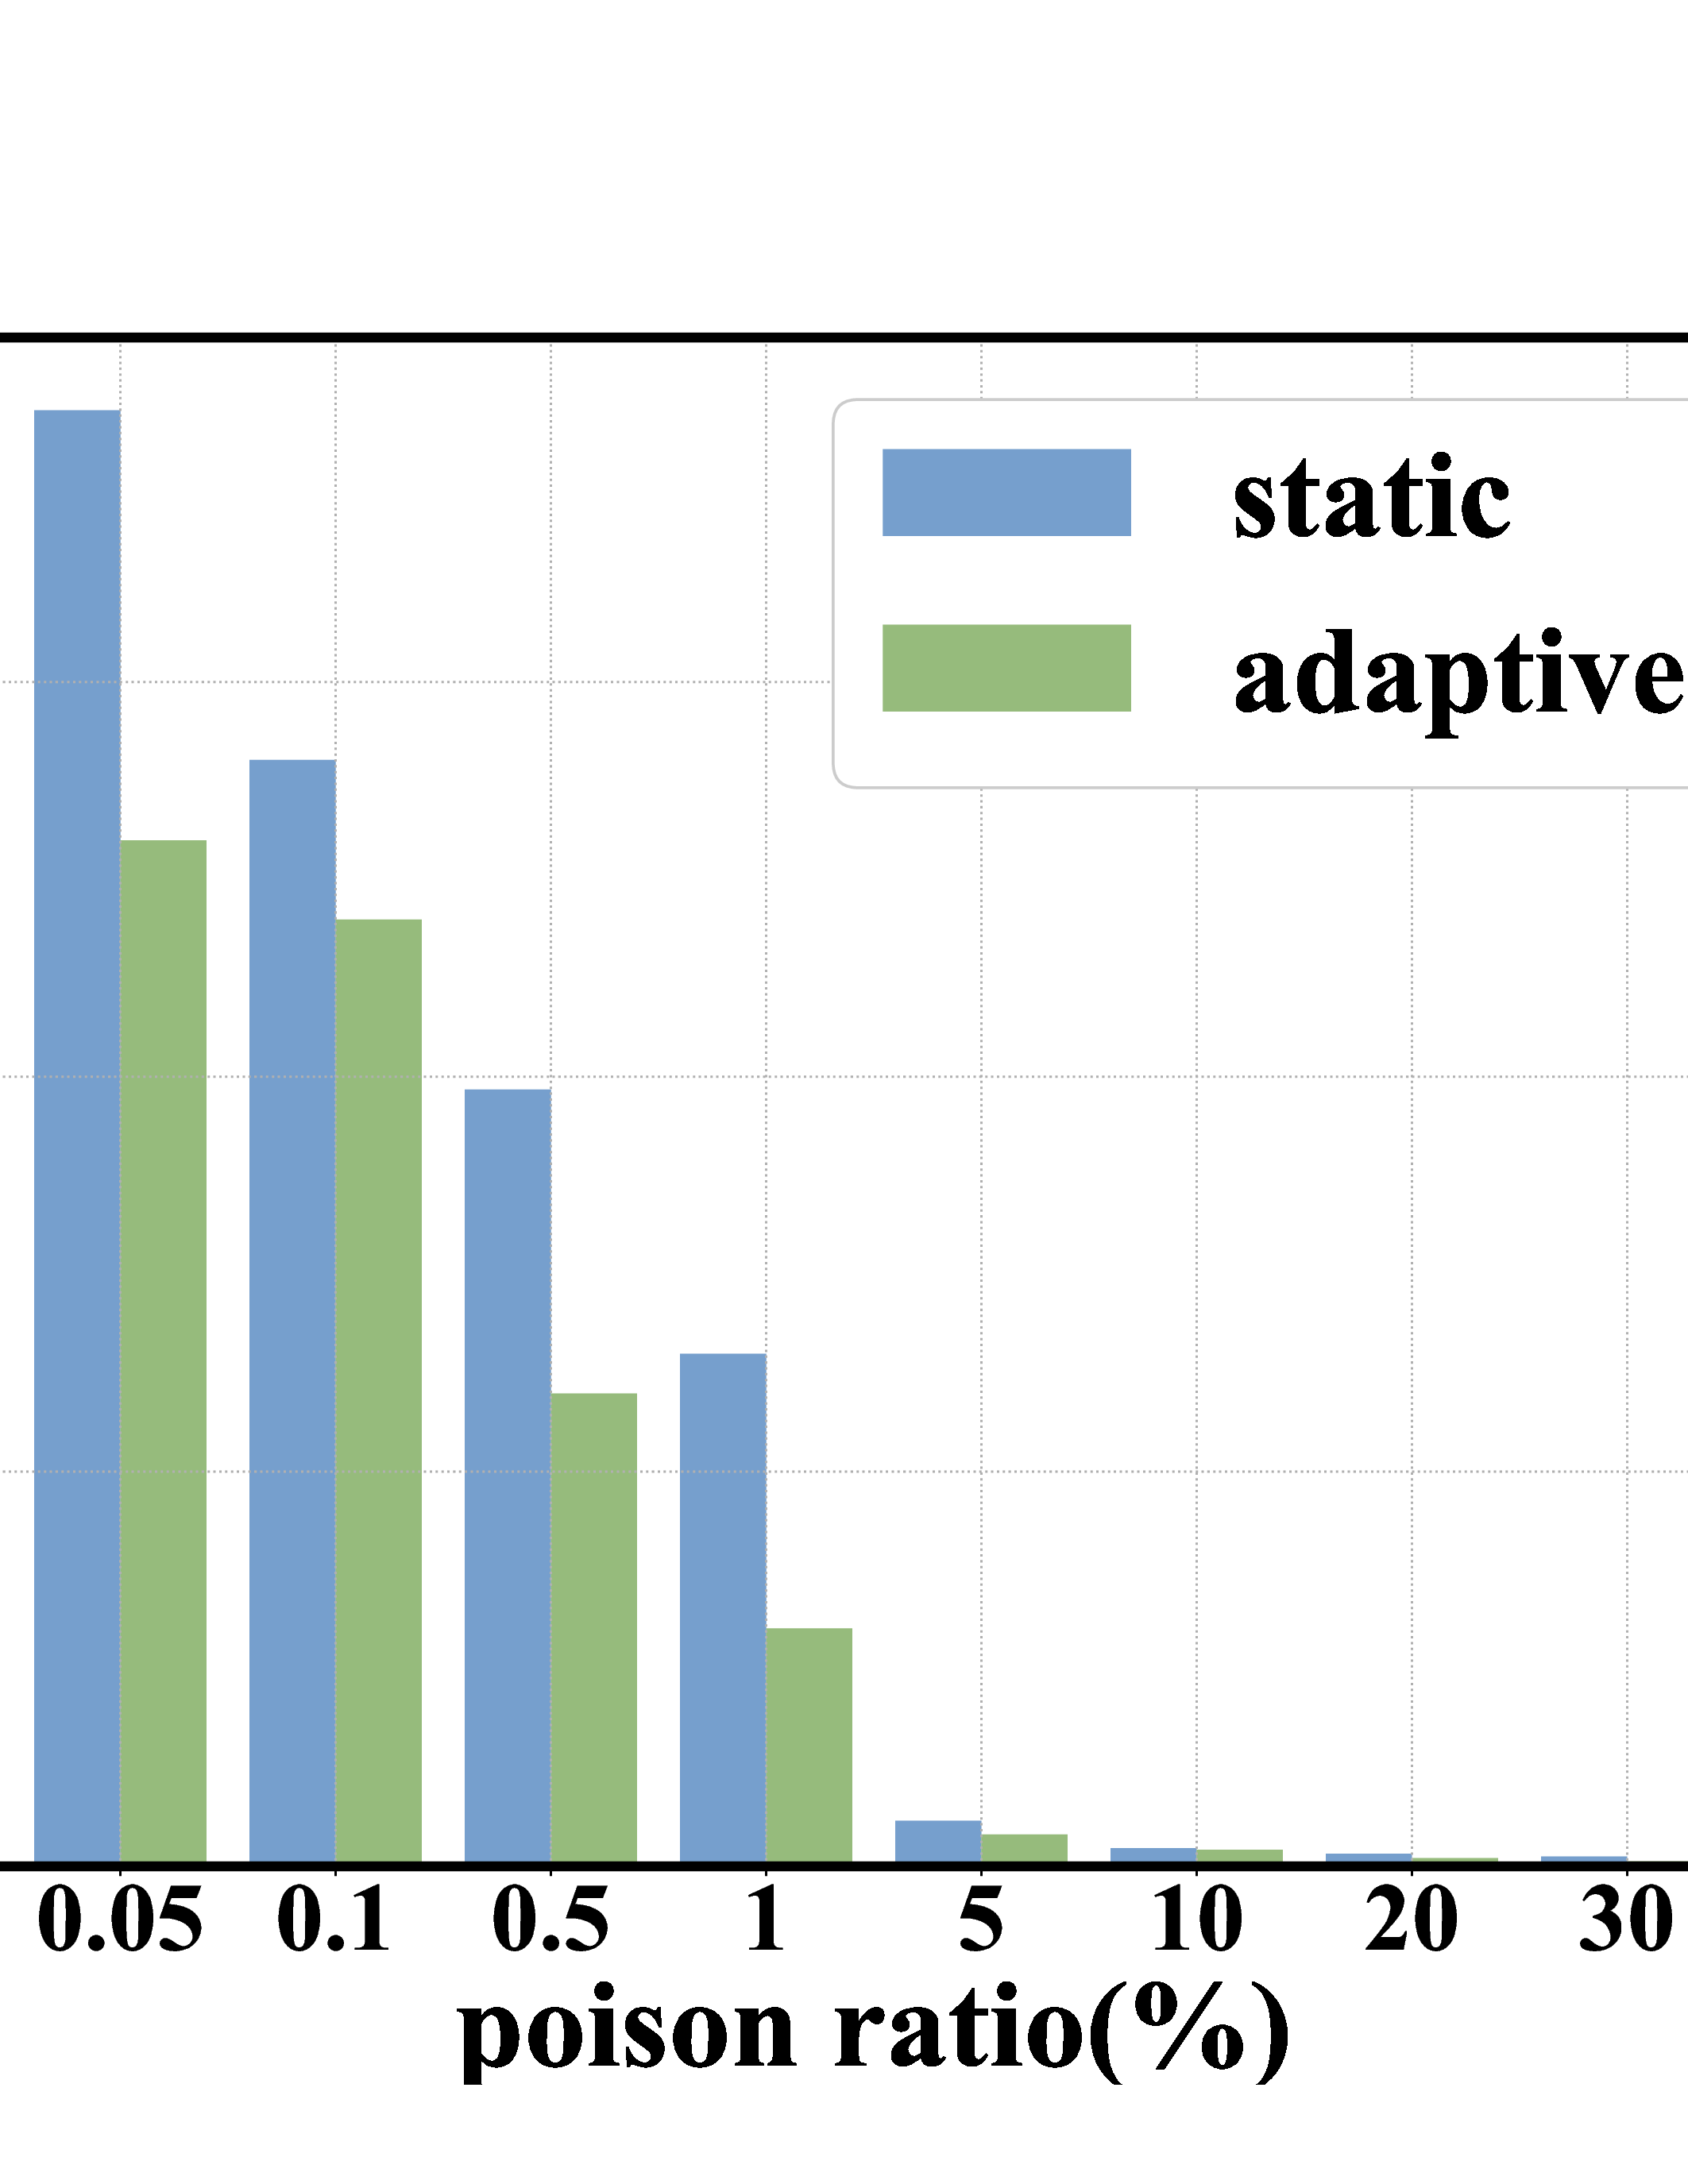}}
	\subfigure[Purchase, precision]{
		\label{fig:all_poison_ratio2}
		\includegraphics[width=0.22\textwidth]{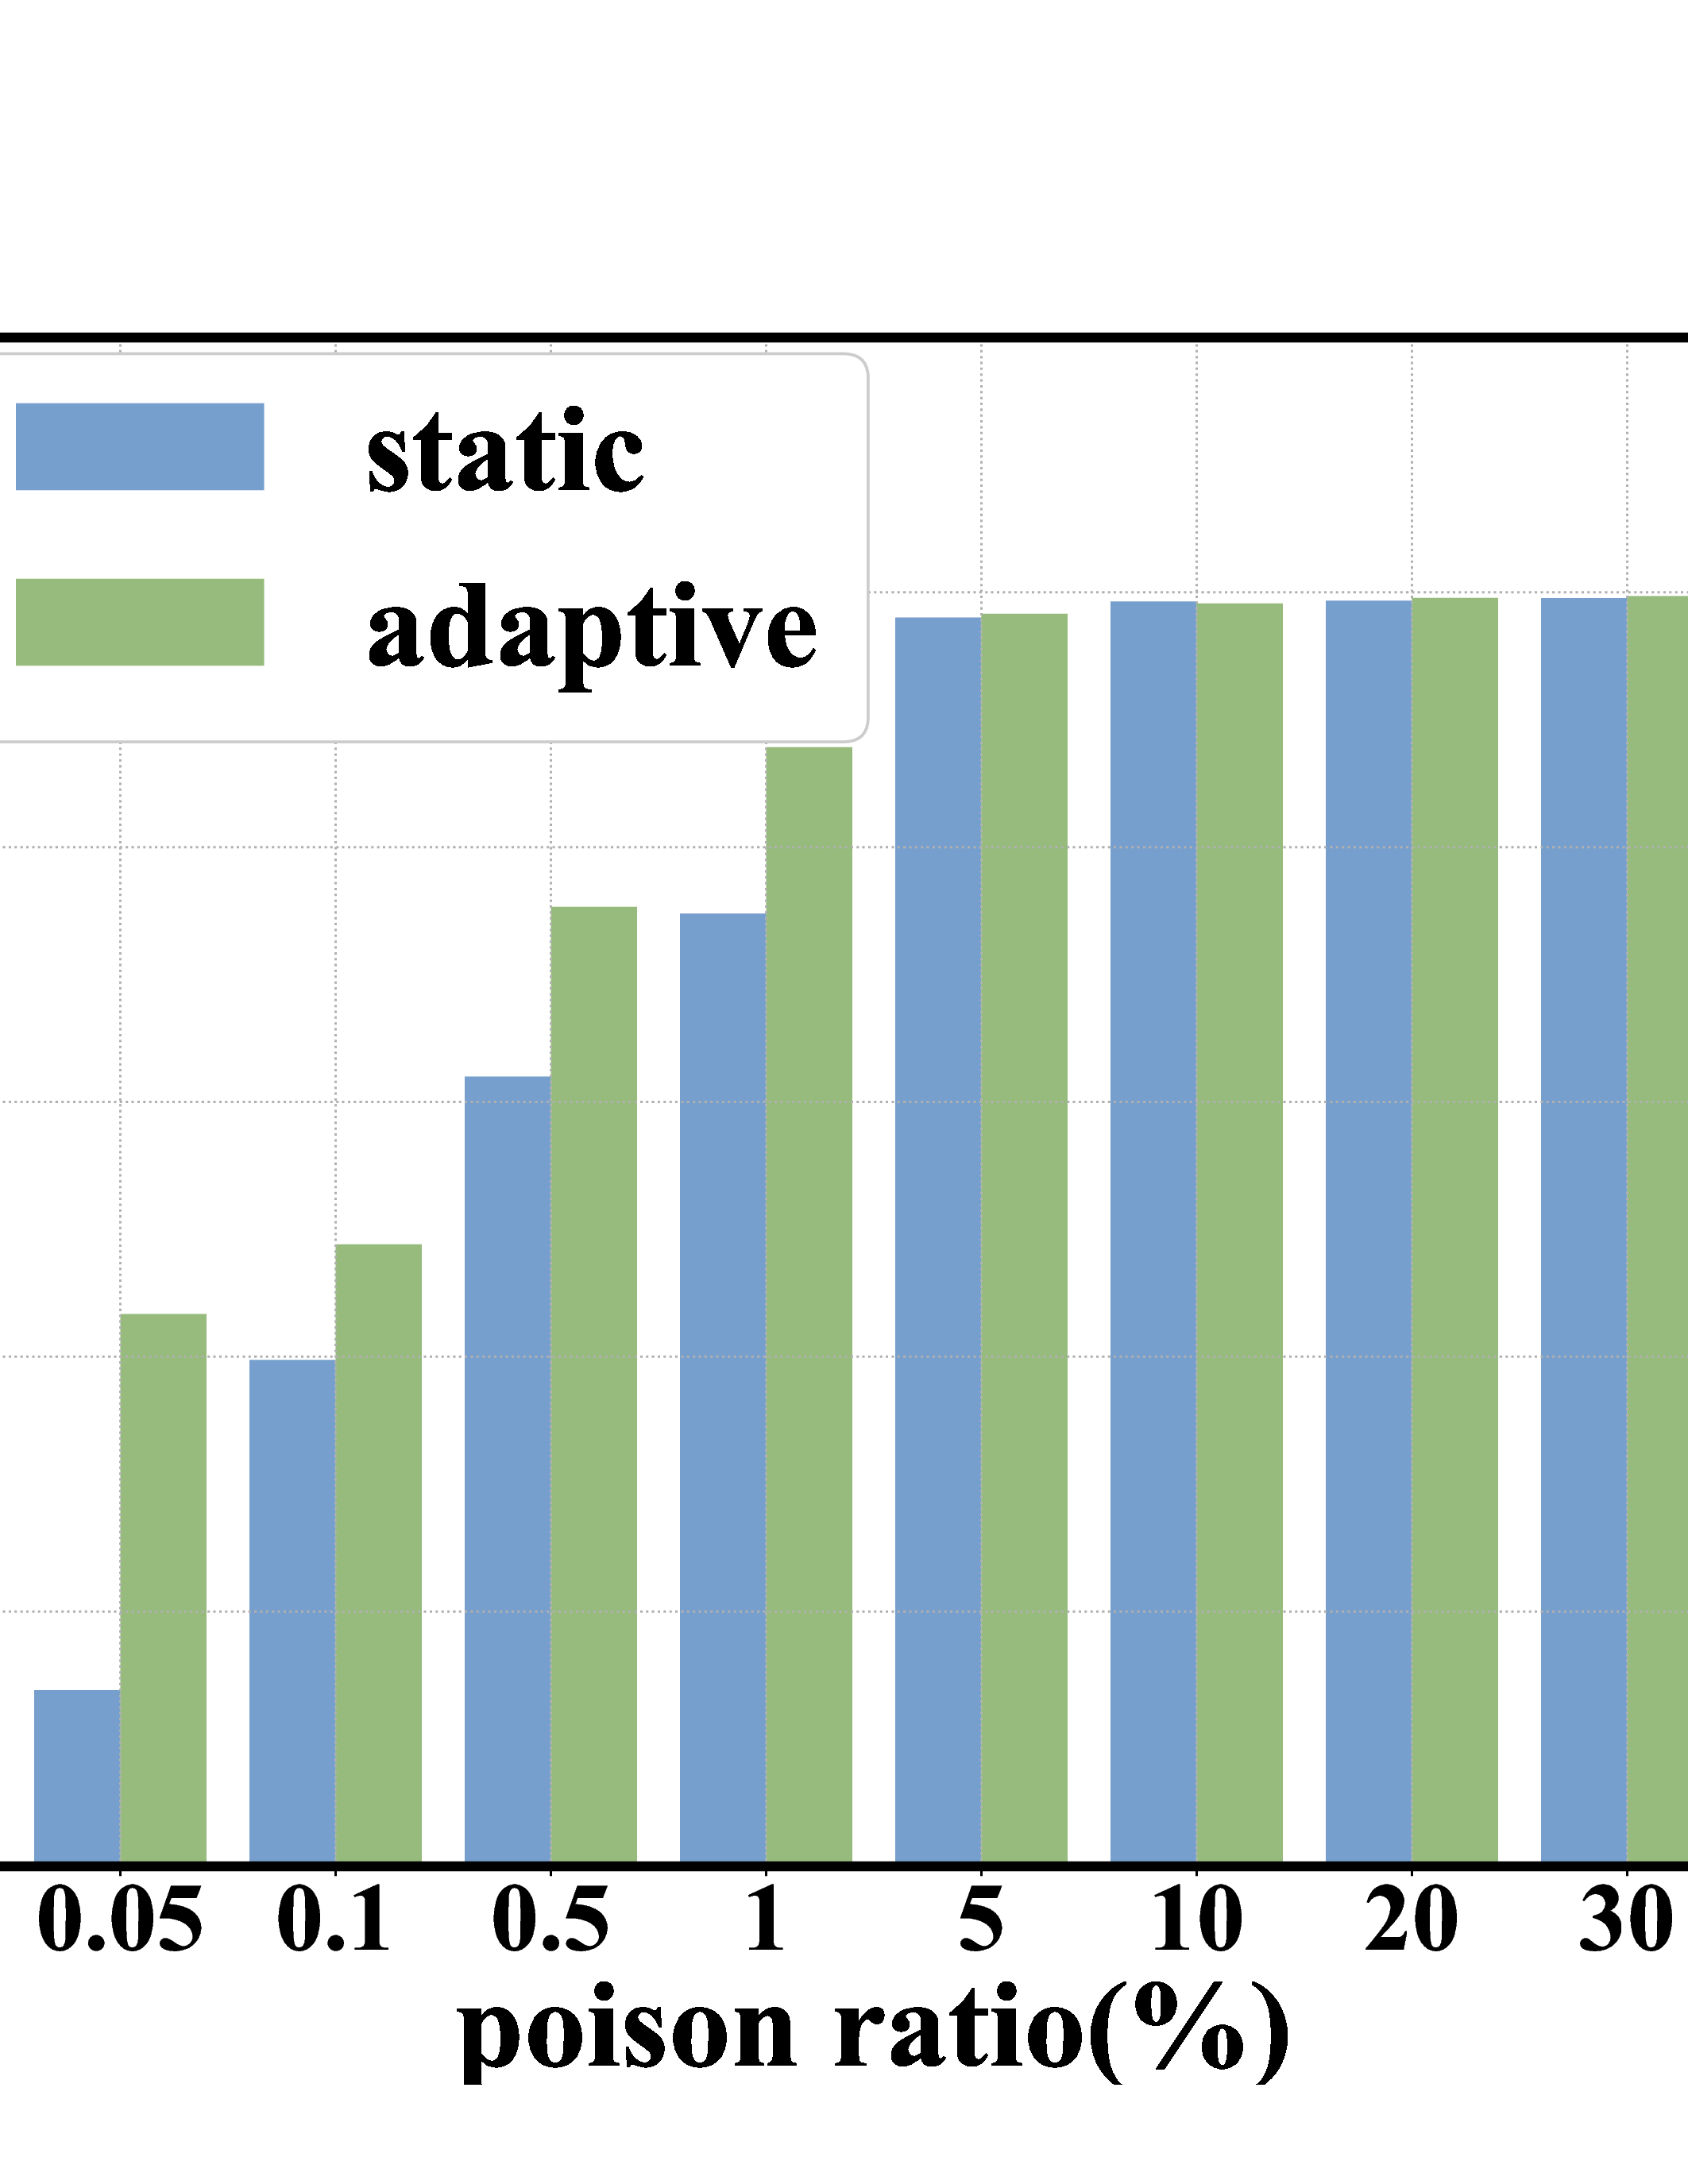}}
	%	\subfigure[Purchase, recall]{
	%		\label{fig:all_poison_ratio3}
	%		\includegraphics[width=0.22\textwidth]{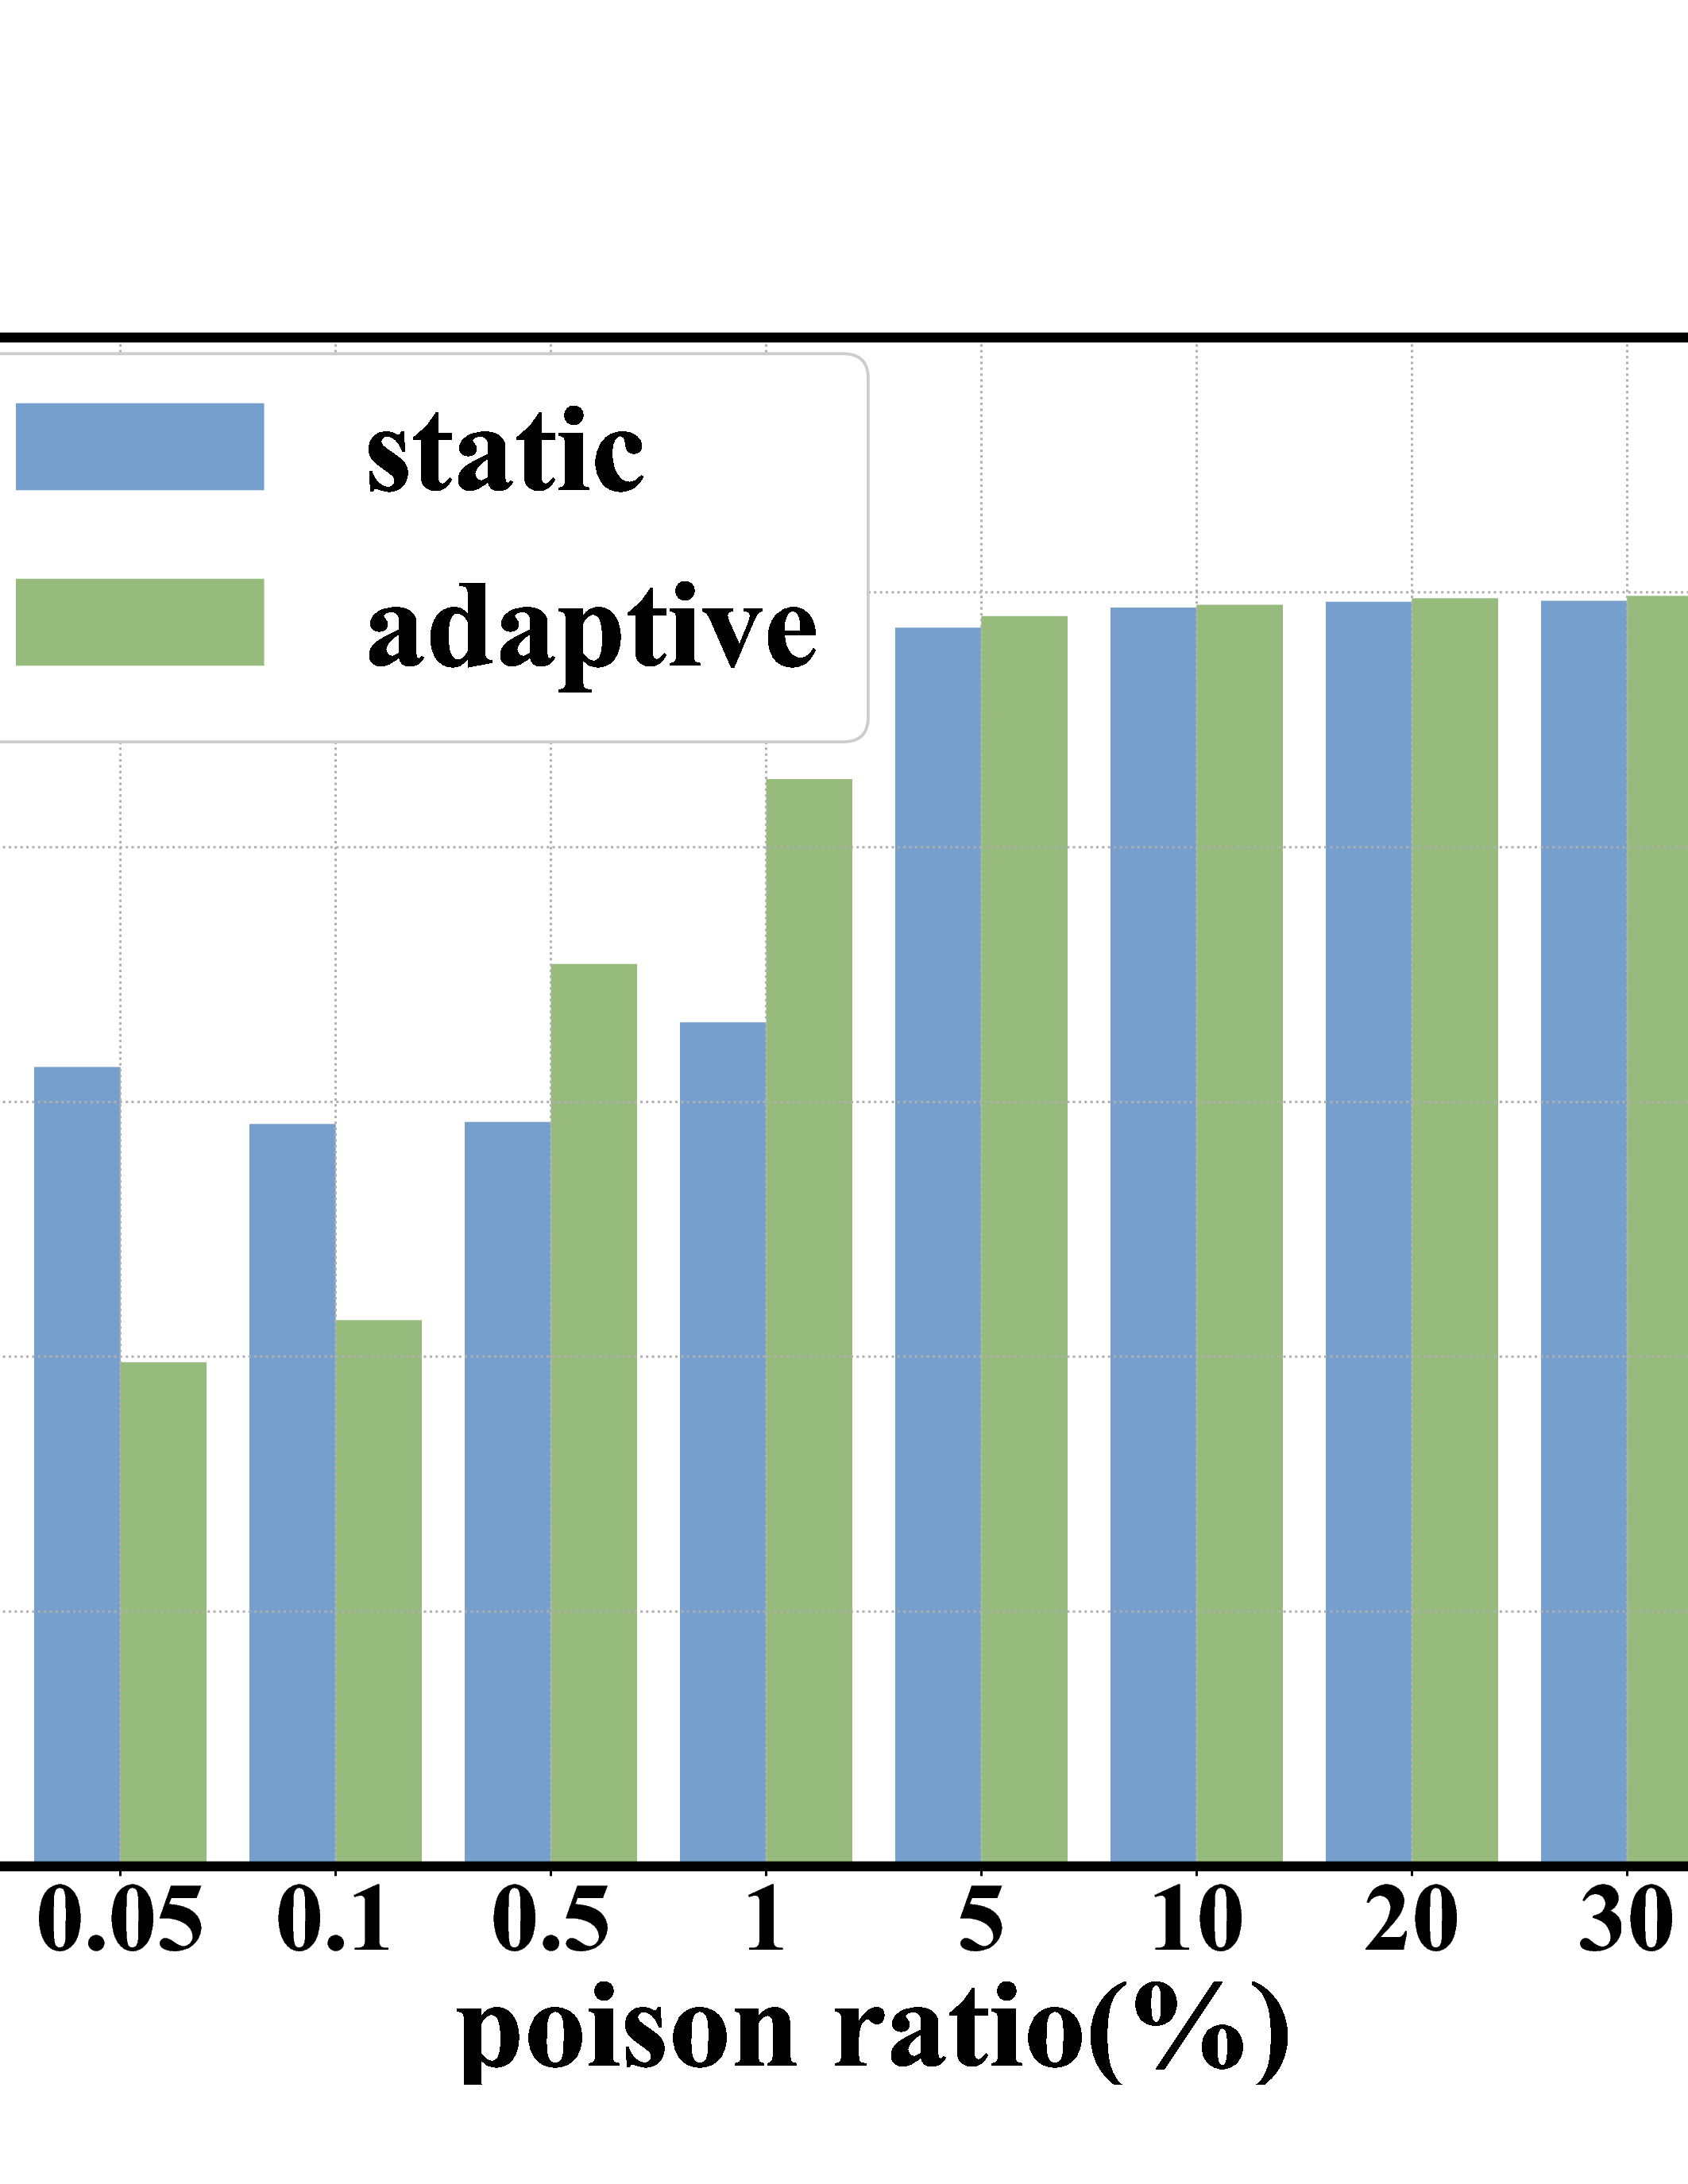}}
	%	\subfigure[{\color{red} Delete}Credit, adaptive attack]{
	%		\label{fig:all_poison_ratio4}
	%		\includegraphics[width=0.22\textwidth]{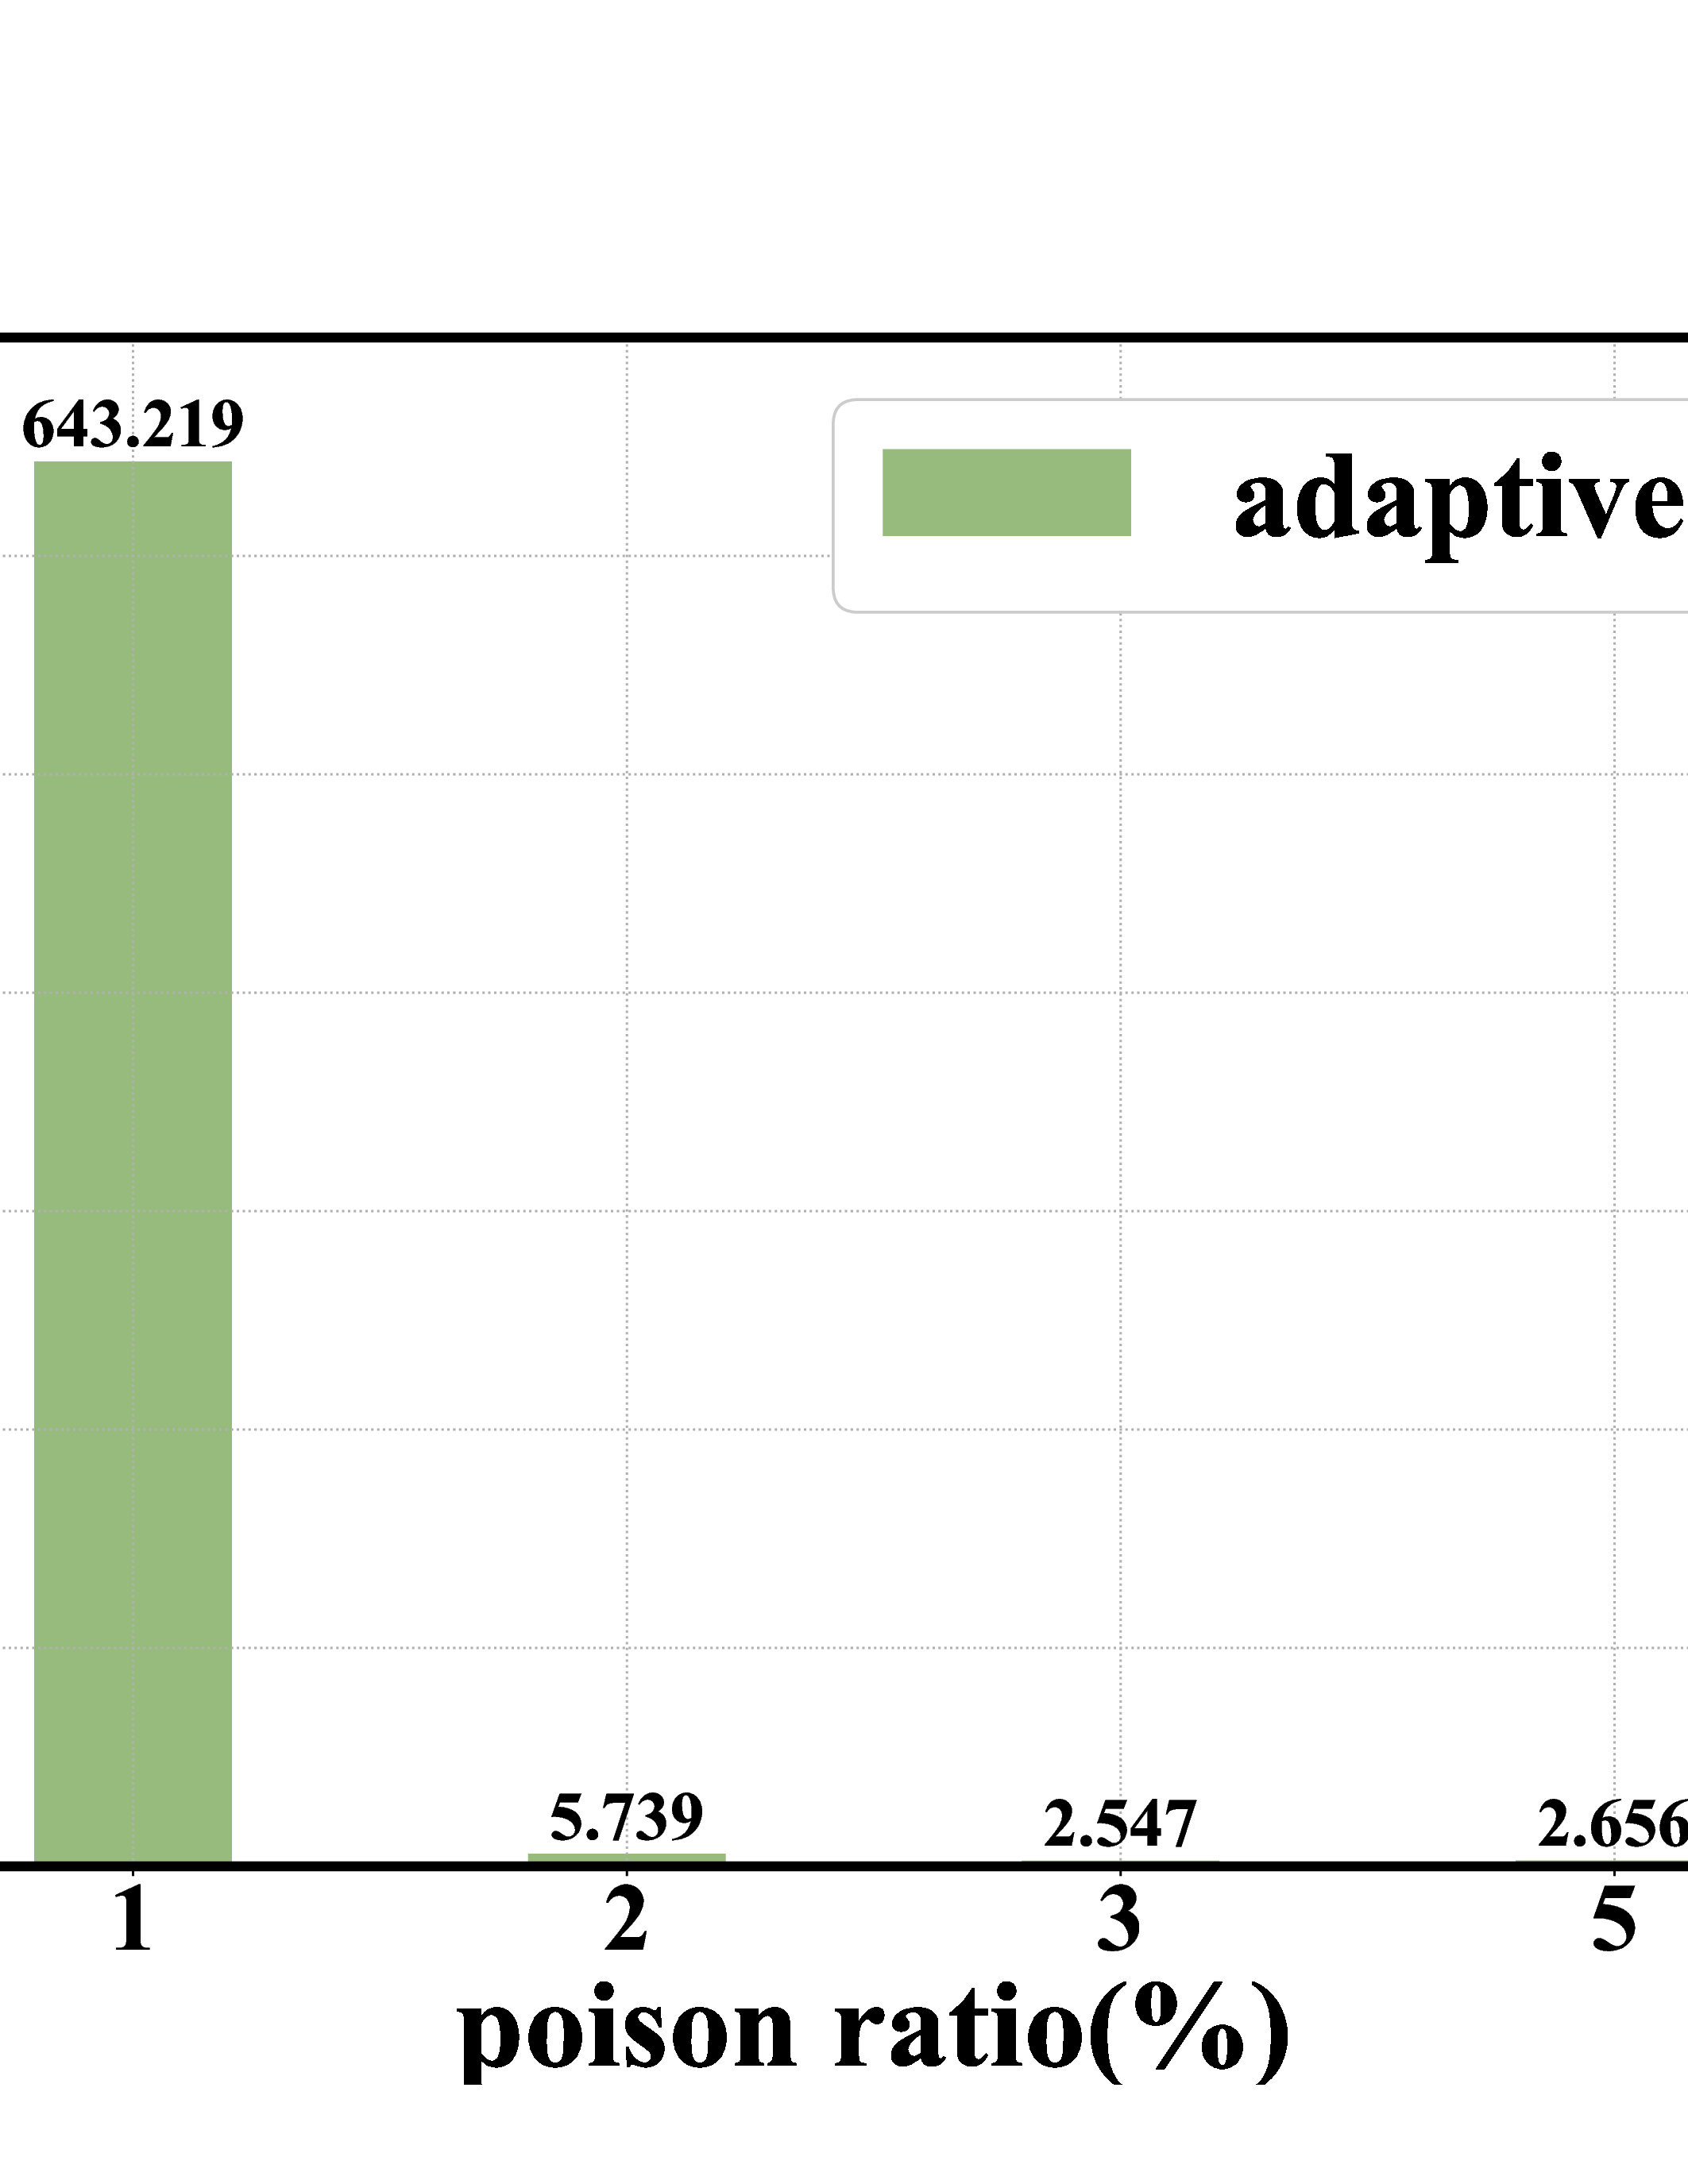}}
	%	\subfigure[Credit, static attack]{
	%		\label{fig:all_poison_ratio5}
	%		\includegraphics[width=0.22\textwidth]{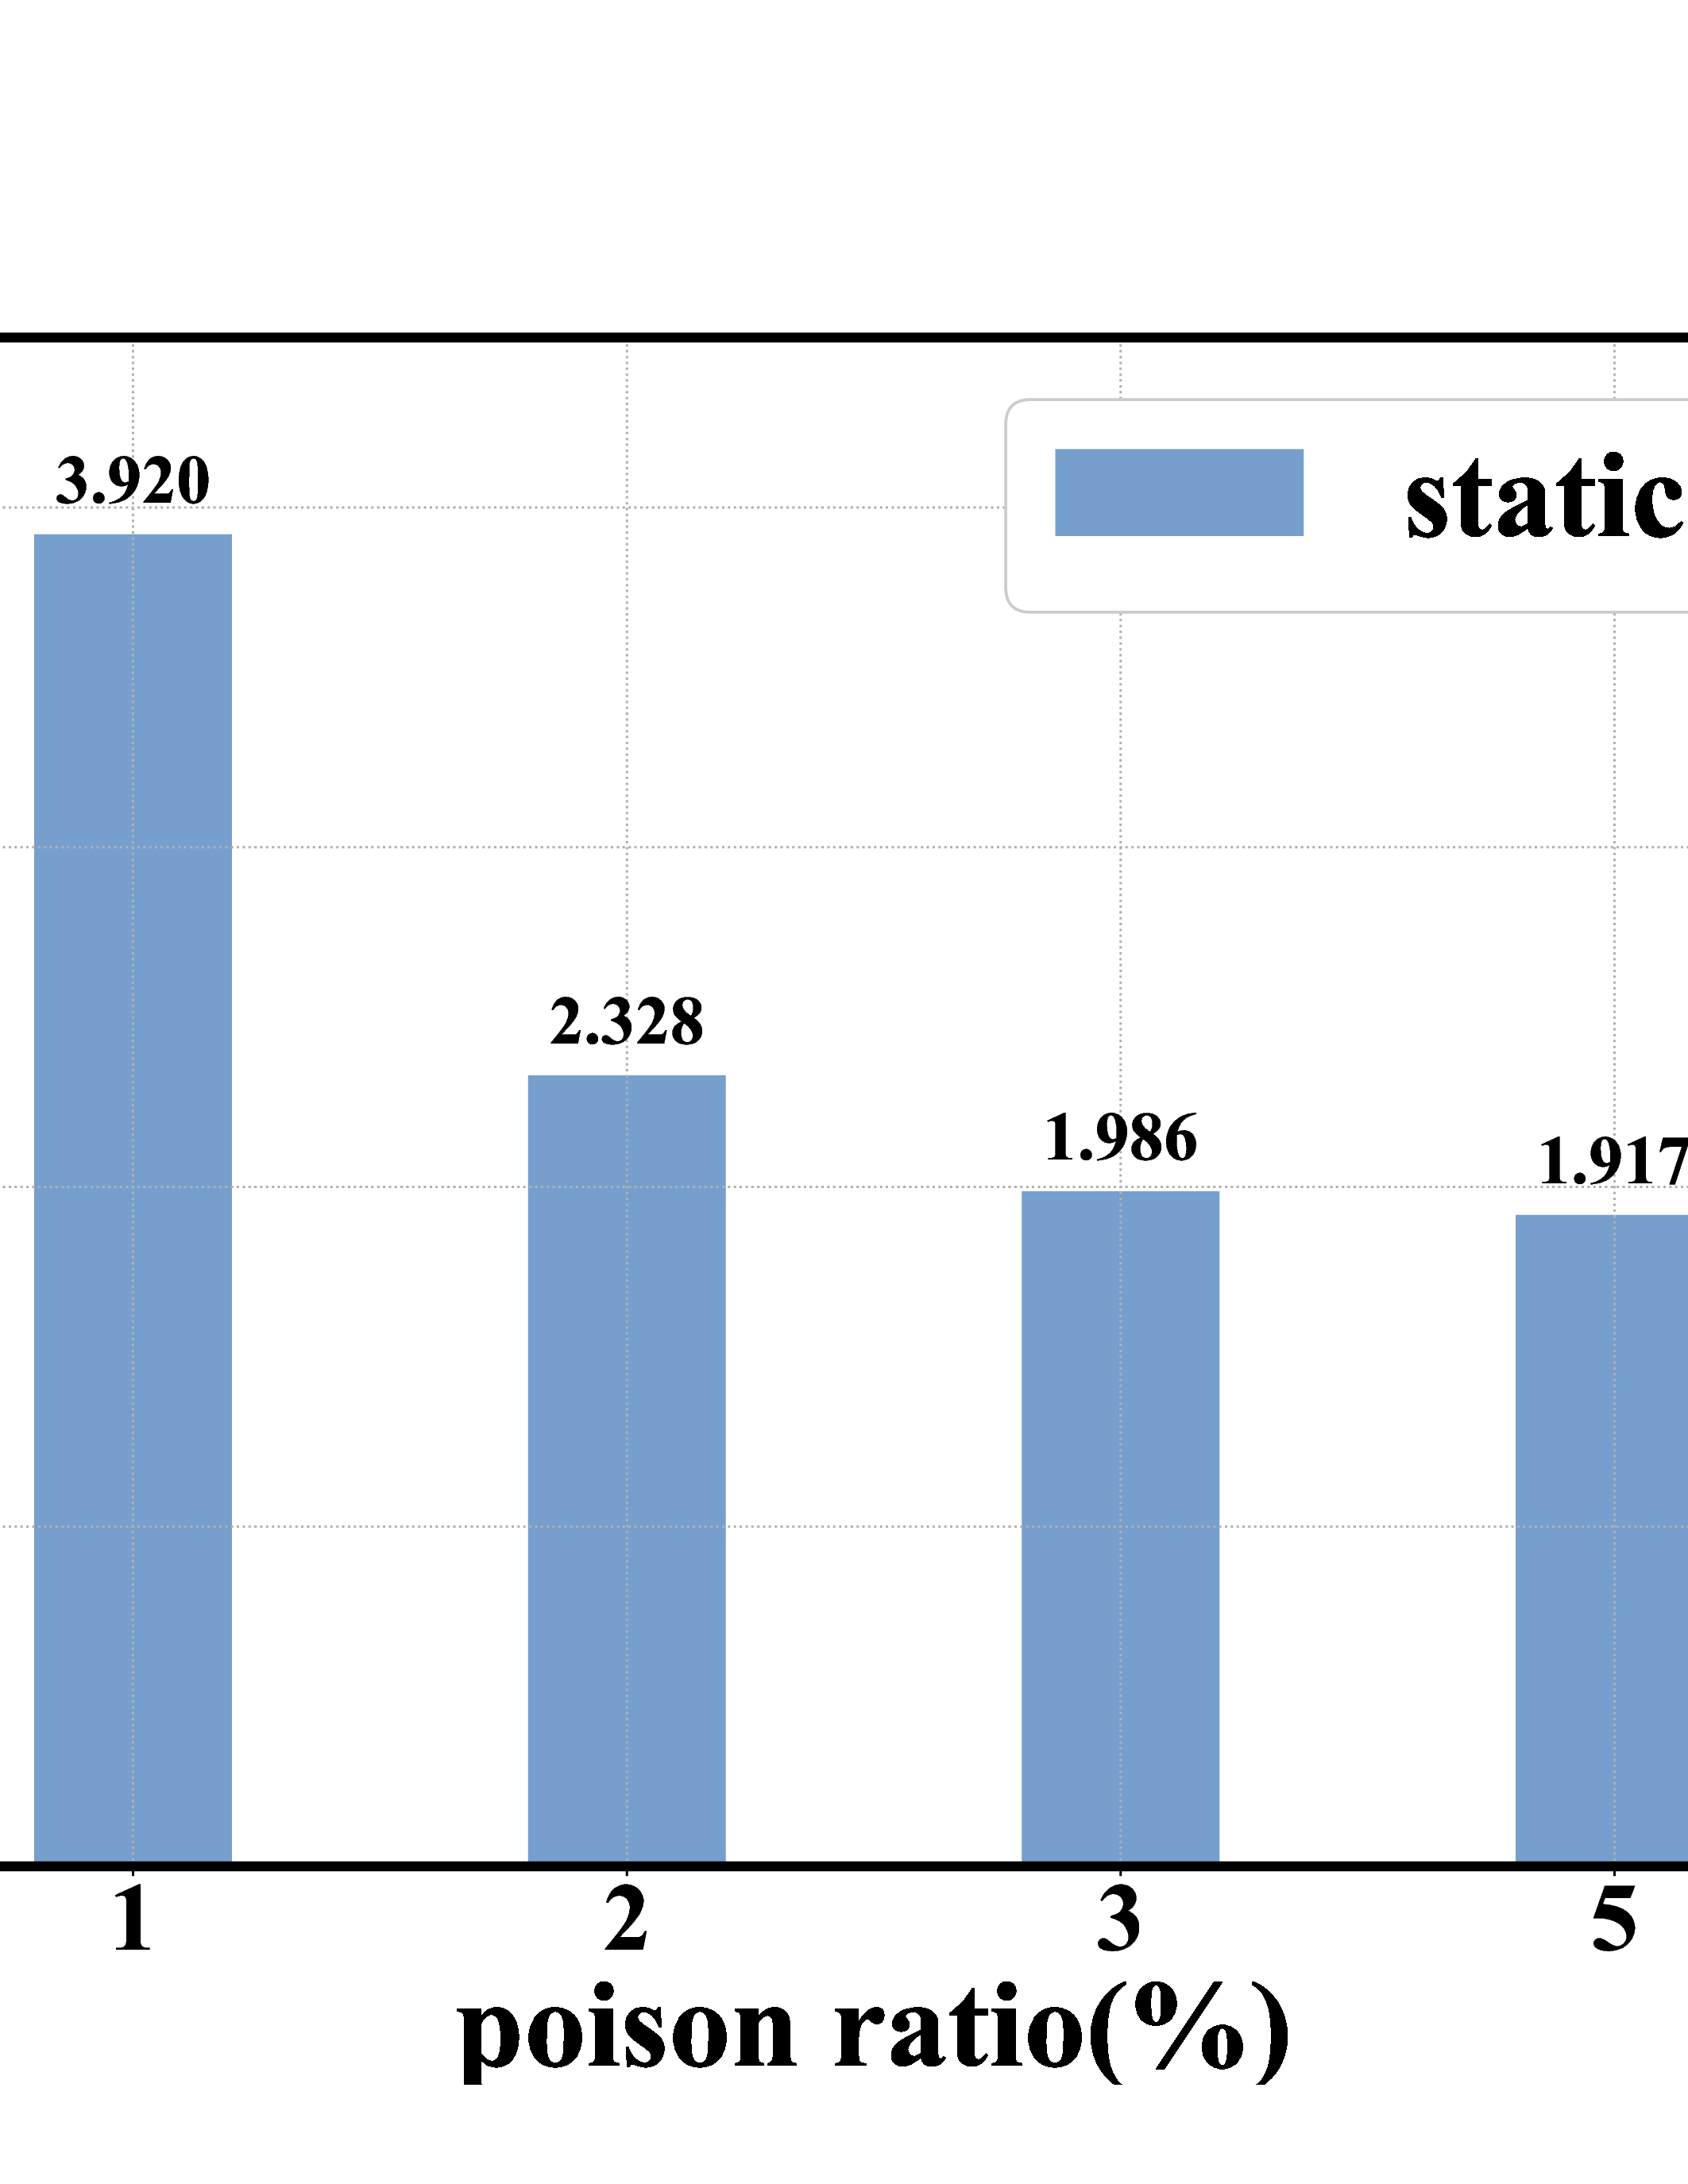}}
	\subfigure[COCO-QA, f1-score]{
		\label{fig:all_poison_ratio6}
		\includegraphics[width=0.22\textwidth]{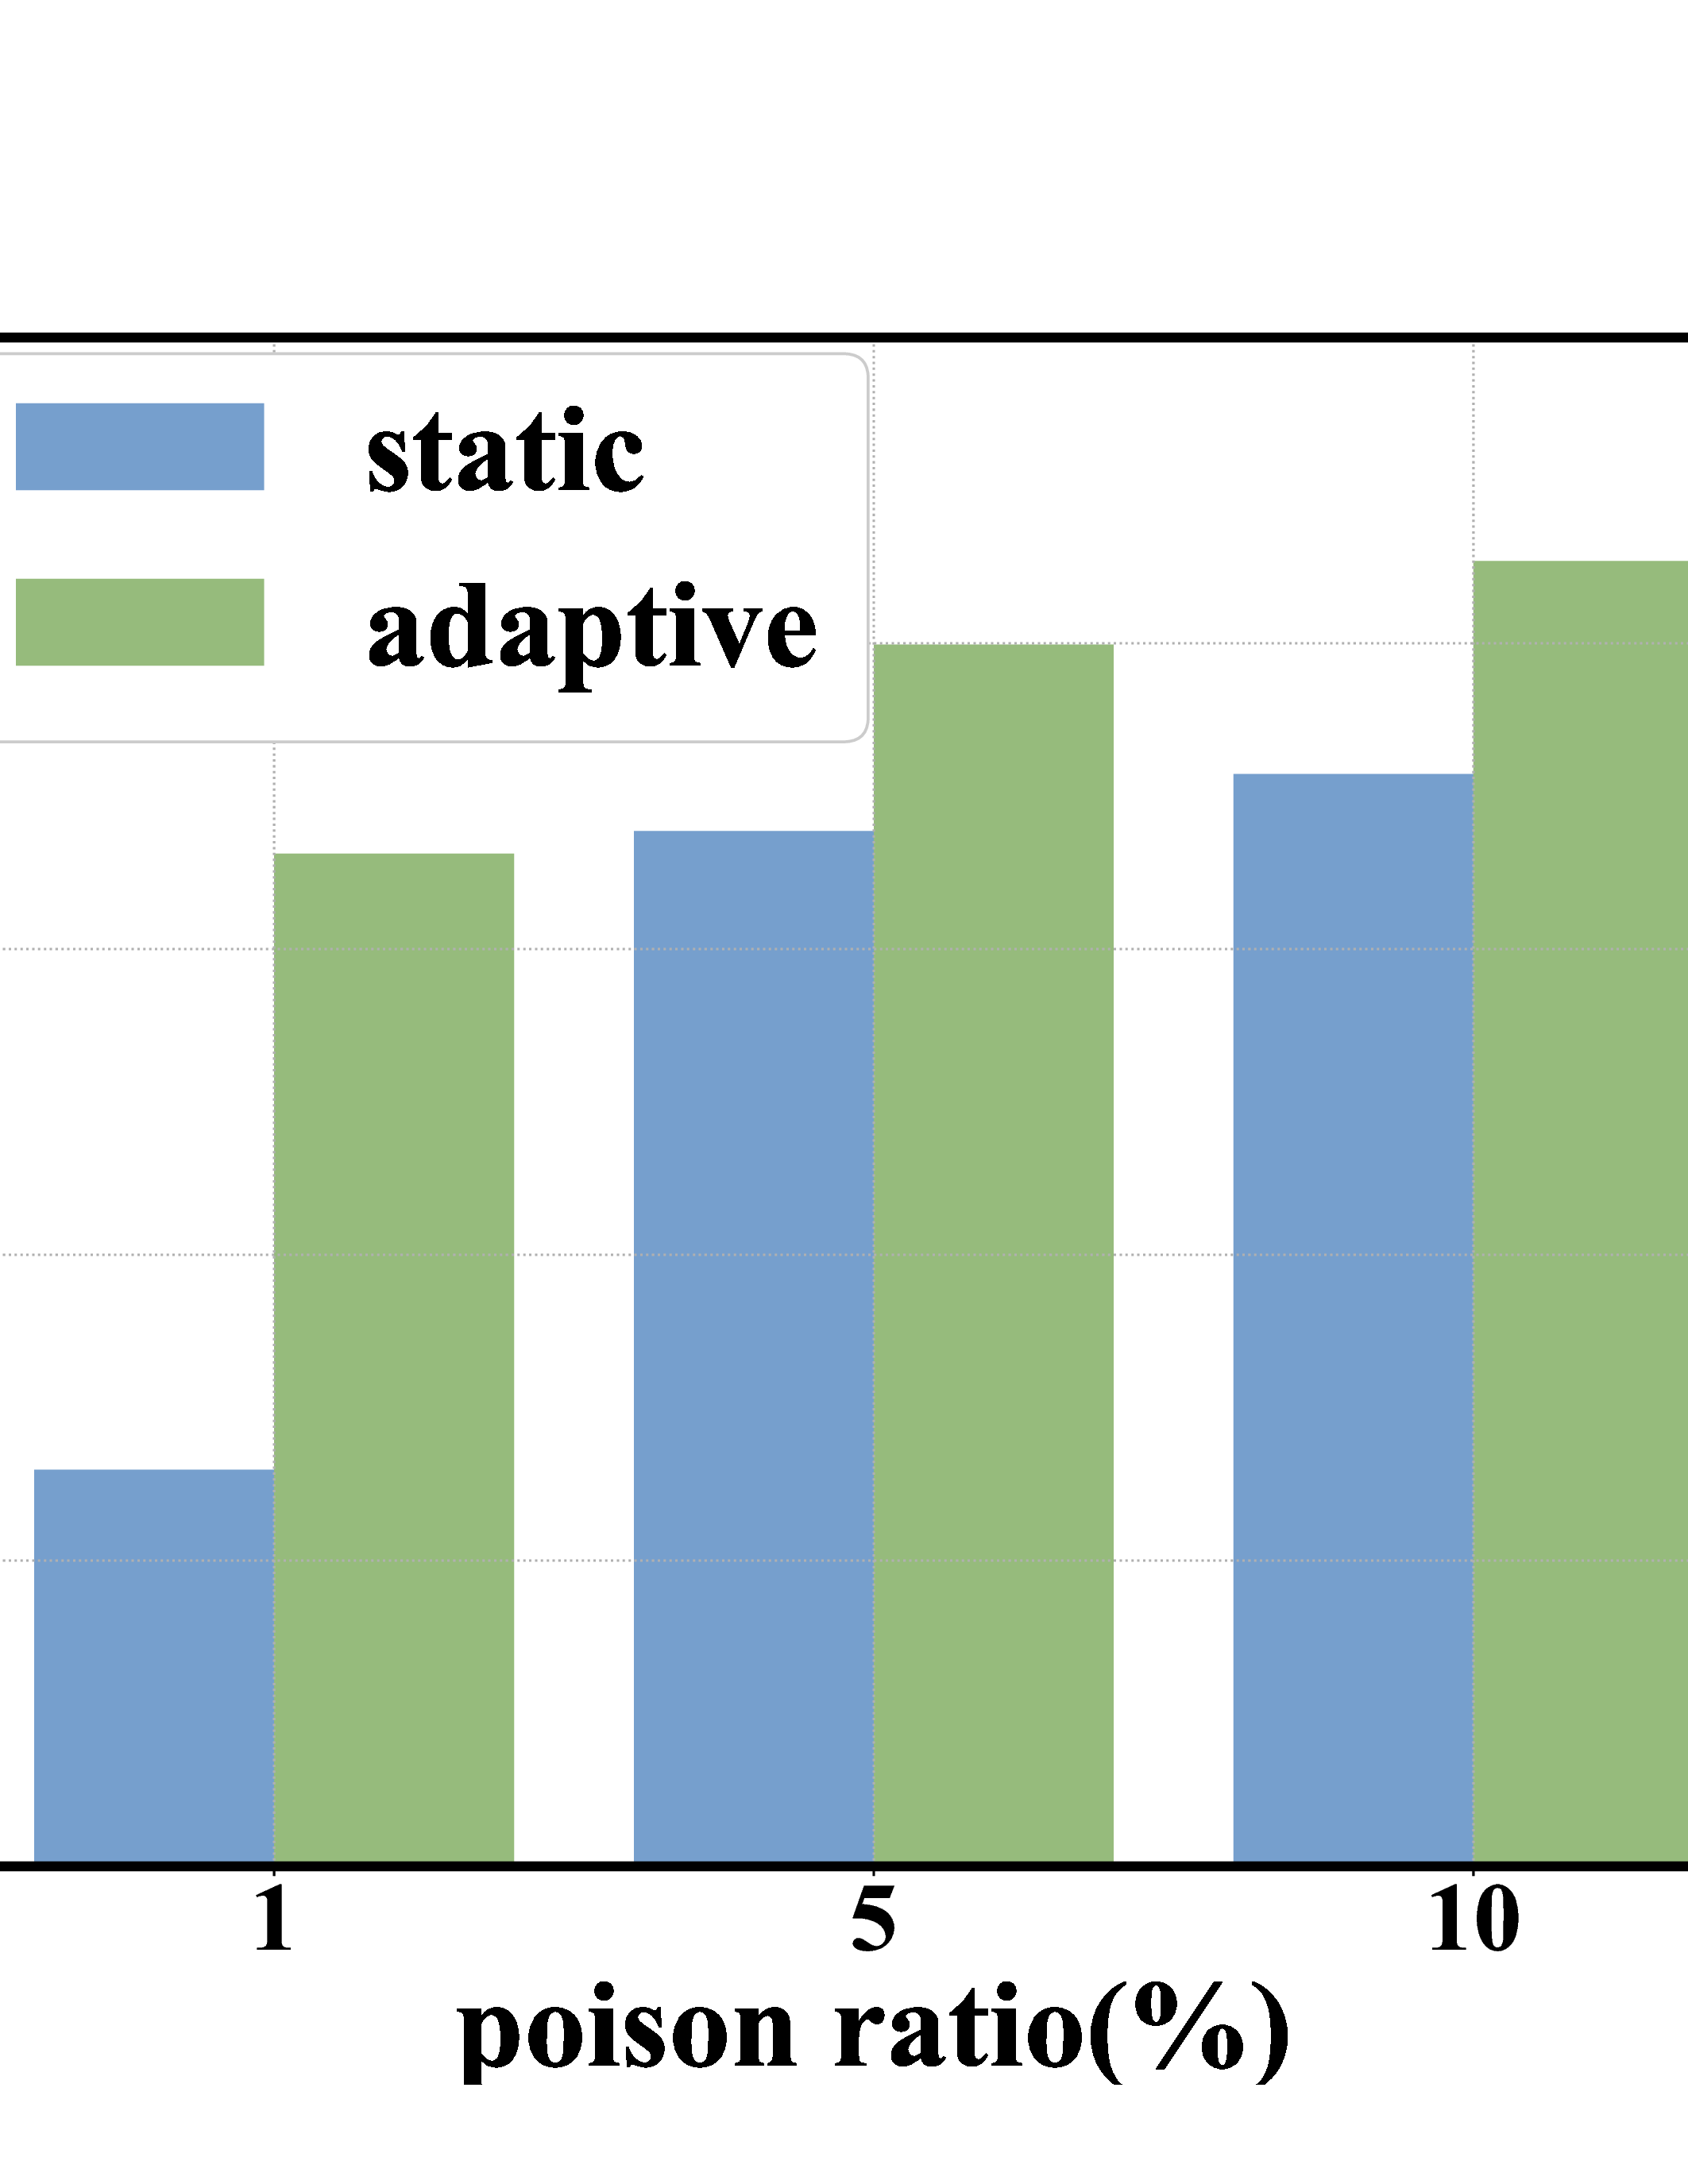}}
	\subfigure[Adult, error rate]{
		\label{fig:all_poison_ratio8}
		\includegraphics[width=0.22\textwidth]{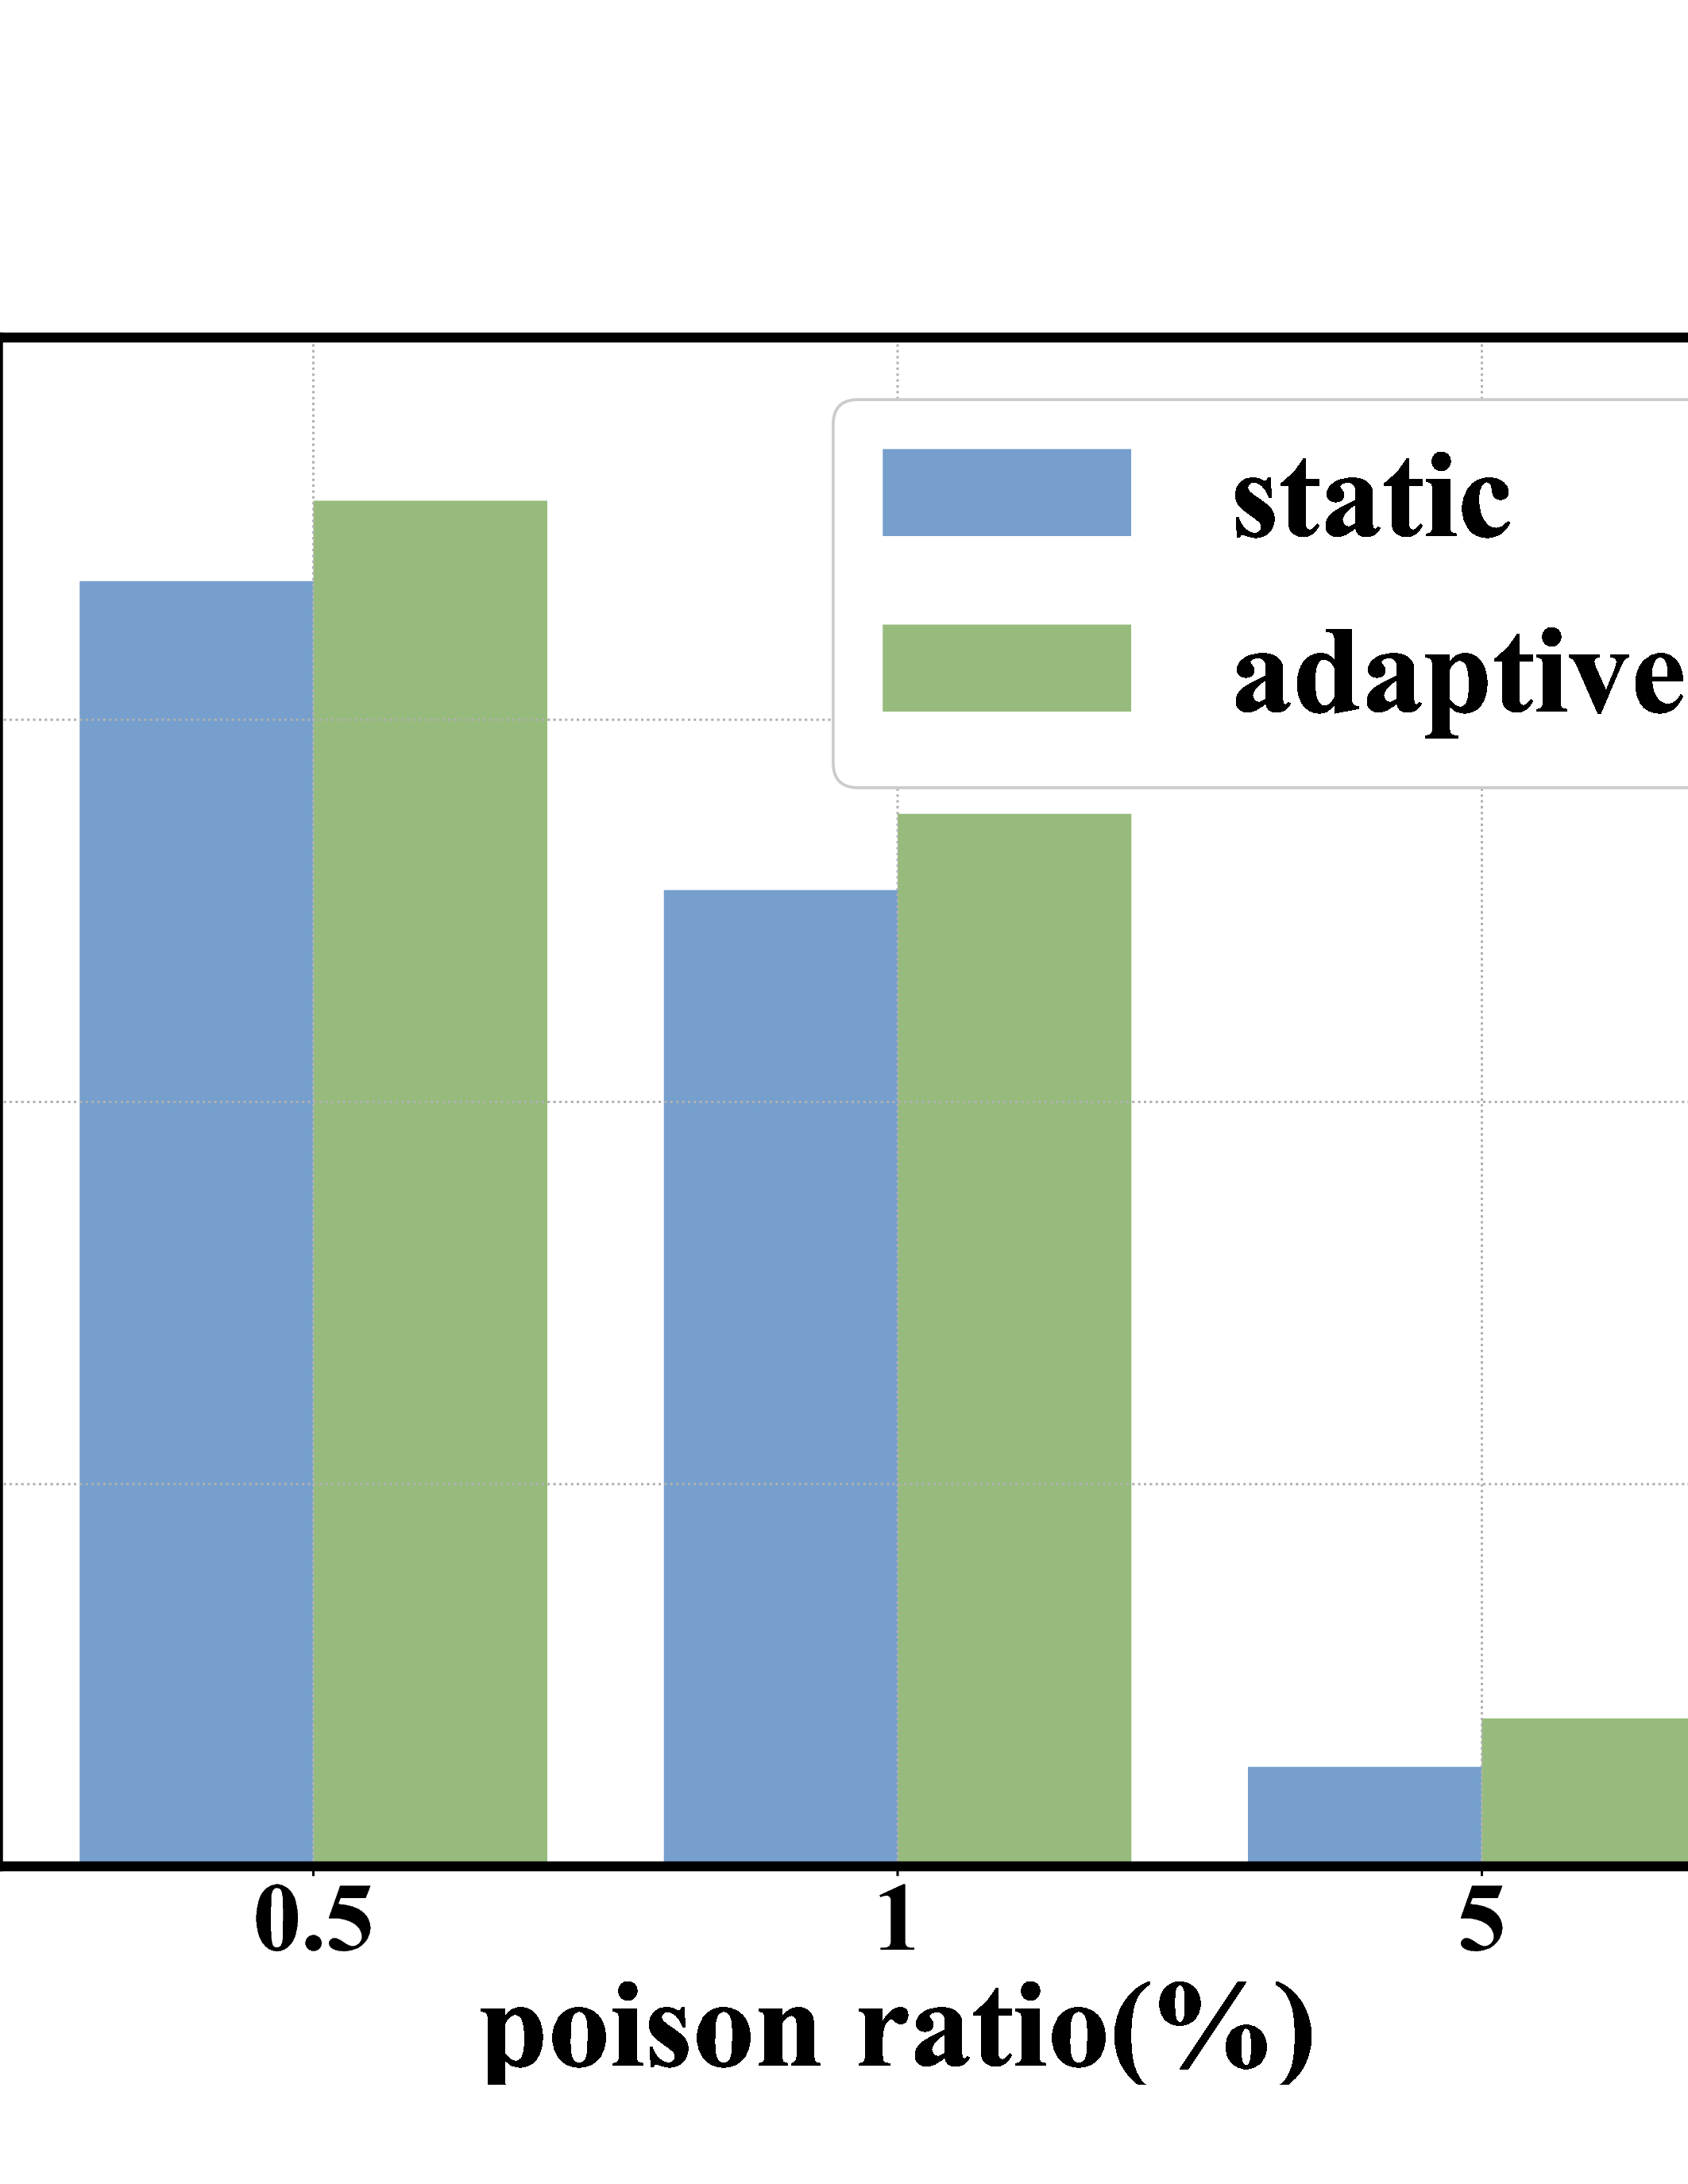}}
	\caption{Attack performance vs. poison ratio.}
	\label{fig:all_poison_ratio}
\end{figure}
\subsubsection{Attack performance vs. poison ratio.}
Fig.~\ref{fig:all_poison_ratio1} and Fig.~\ref{fig:all_poison_ratio2} show the attack performance over different poison ratios on Purchase measured by different privacy metrics (i.e. error rate and precision).
Fig.~\ref{fig:all_poison_ratio6} is the results for COCO-QA using f1-score.
Fig.~\ref{fig:all_poison_ratio8} is the results for Adult using error rate. 

All these results agree that a higher poison ratio leads to better attack performance for both static attack and adaptive attack as a larger poison ratio means more training data for the adversary.
\begin{figure}[H]
	\centering %图片全局居中
	%并排几个图，就要写几个minipage
	\begin{minipage}[b]{0.45\textwidth} %所有minipage宽度之和要小于1，否则会自动变成竖排
		\centering  %图片全局居中
		\subfigure[Purchase, recall, $\alpha=0.05$]{
			\label{fig:naive_defense1}
			\includegraphics[width=0.45\textwidth]{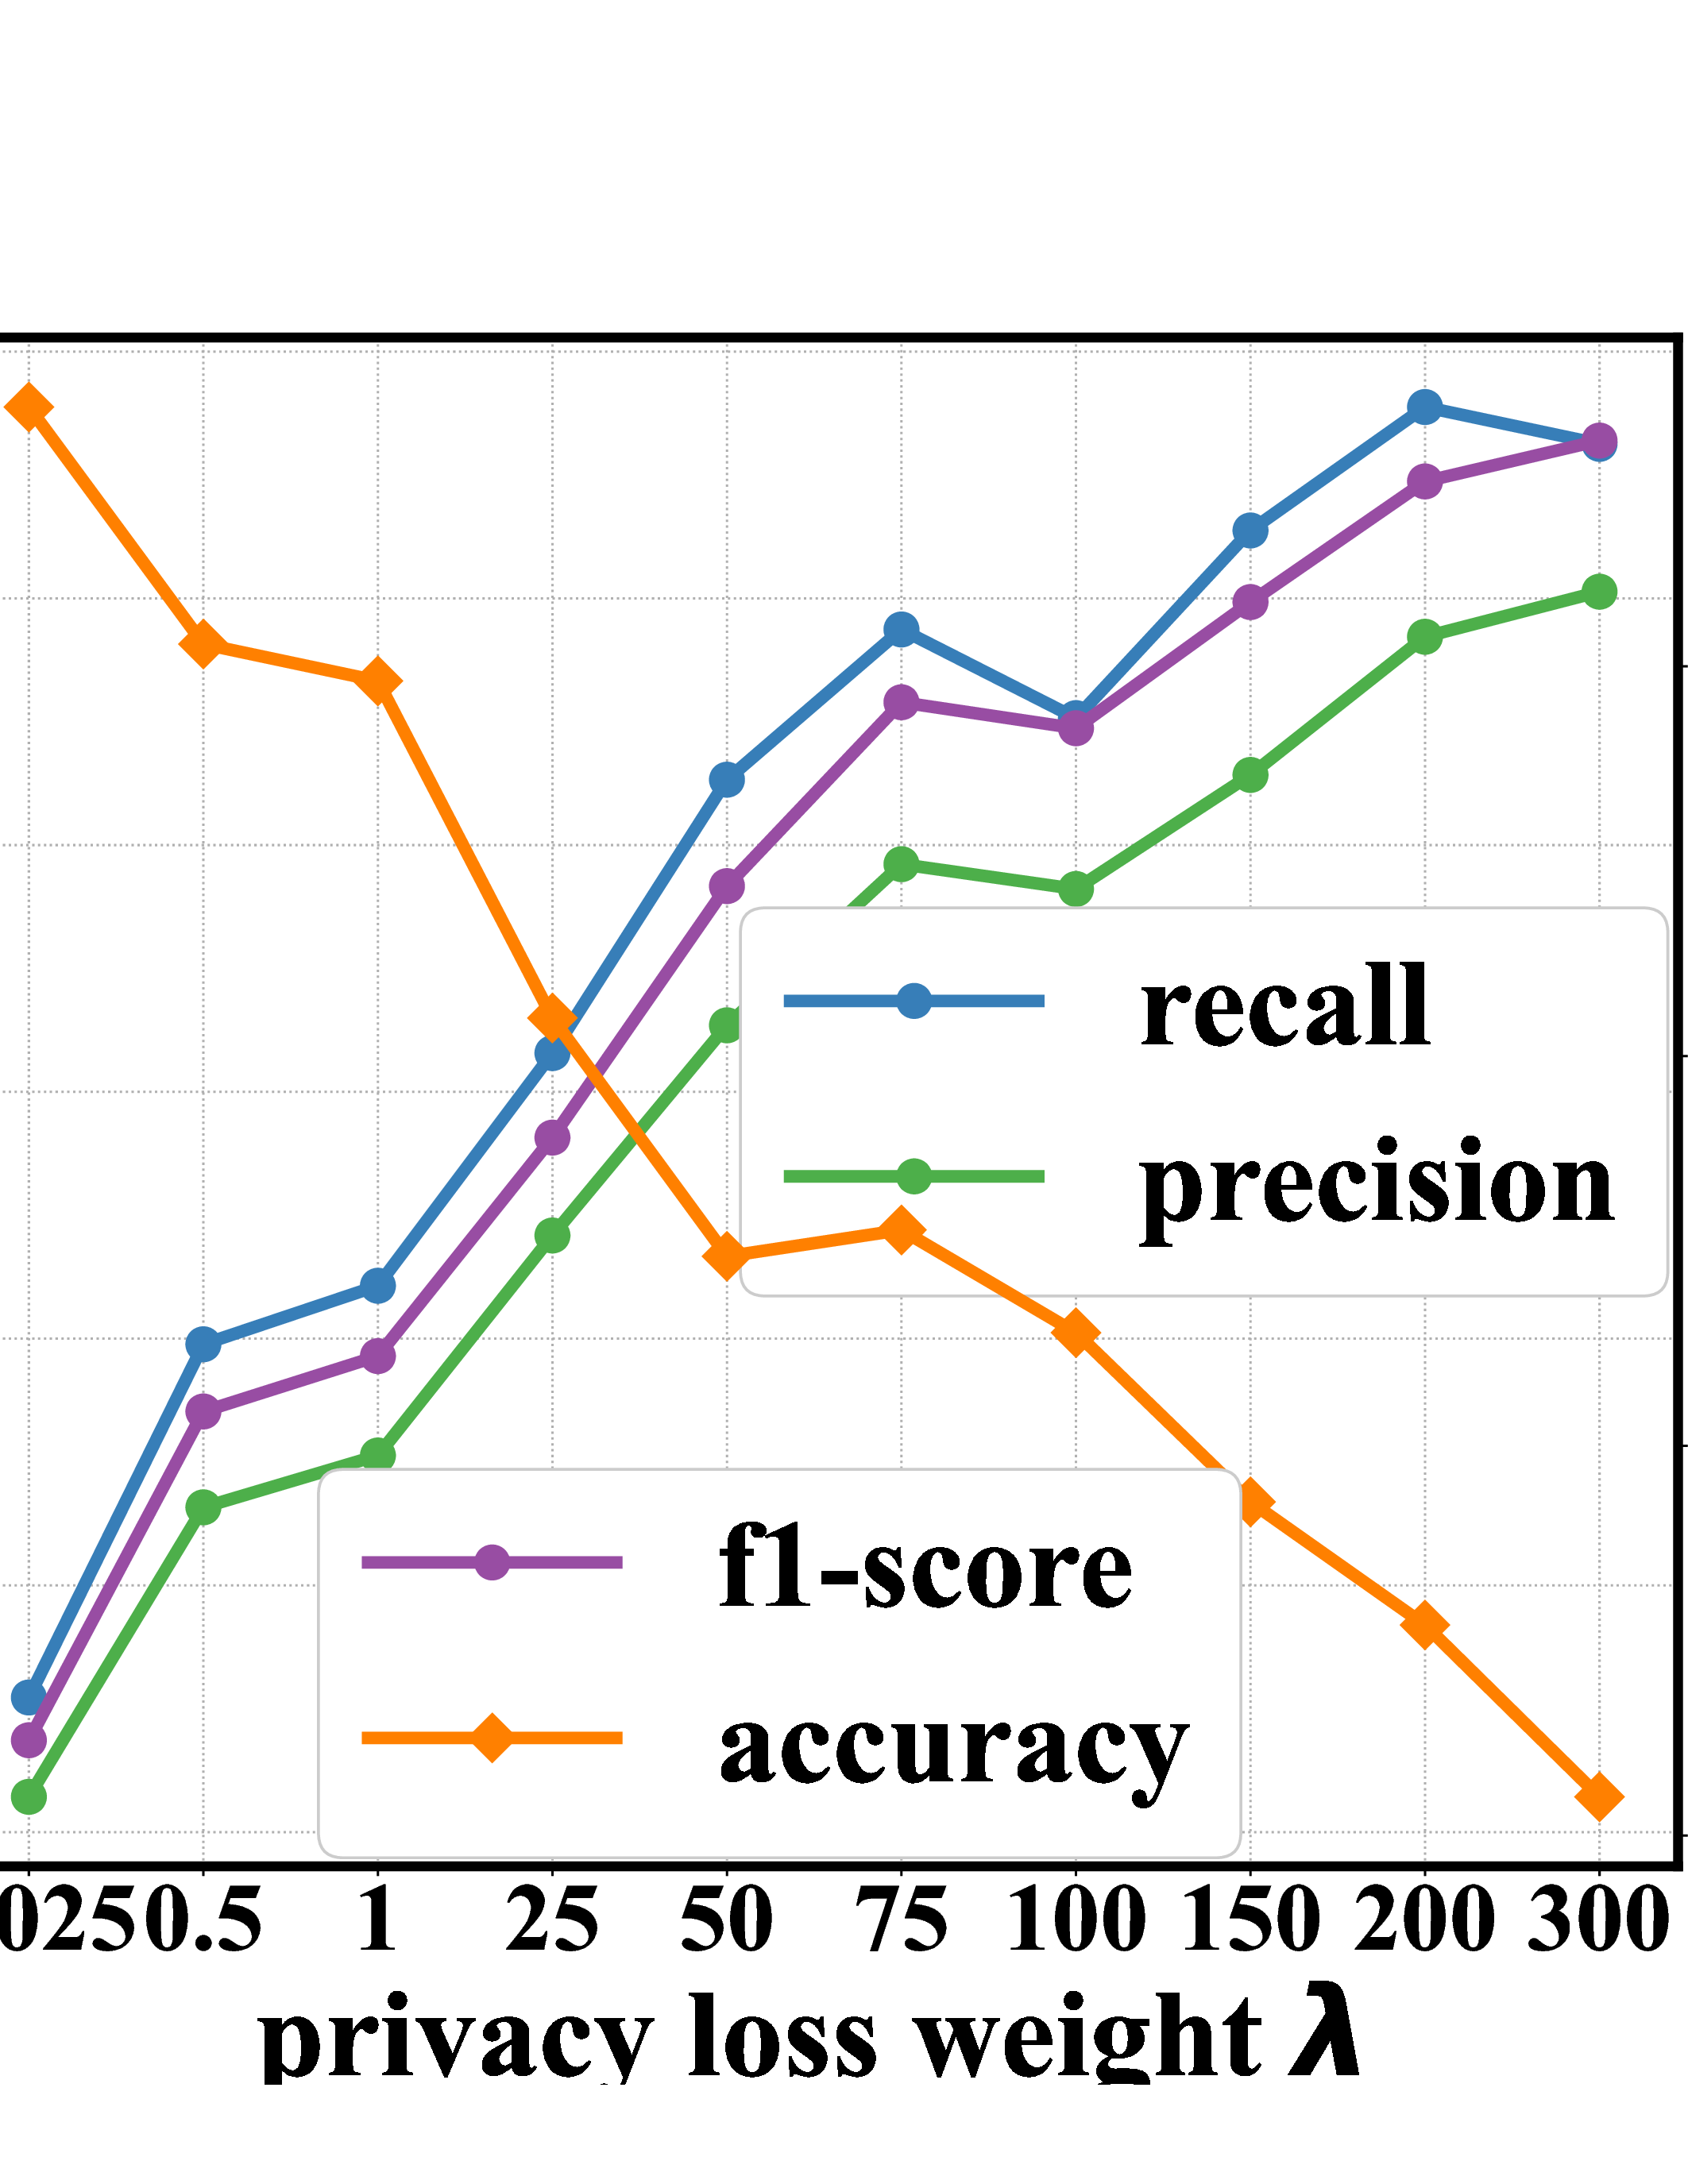}}
		\subfigure[Adult, error rate, $\alpha=0.05$]{
			\label{fig:naive_defense2}
			\includegraphics[width=0.45\textwidth]{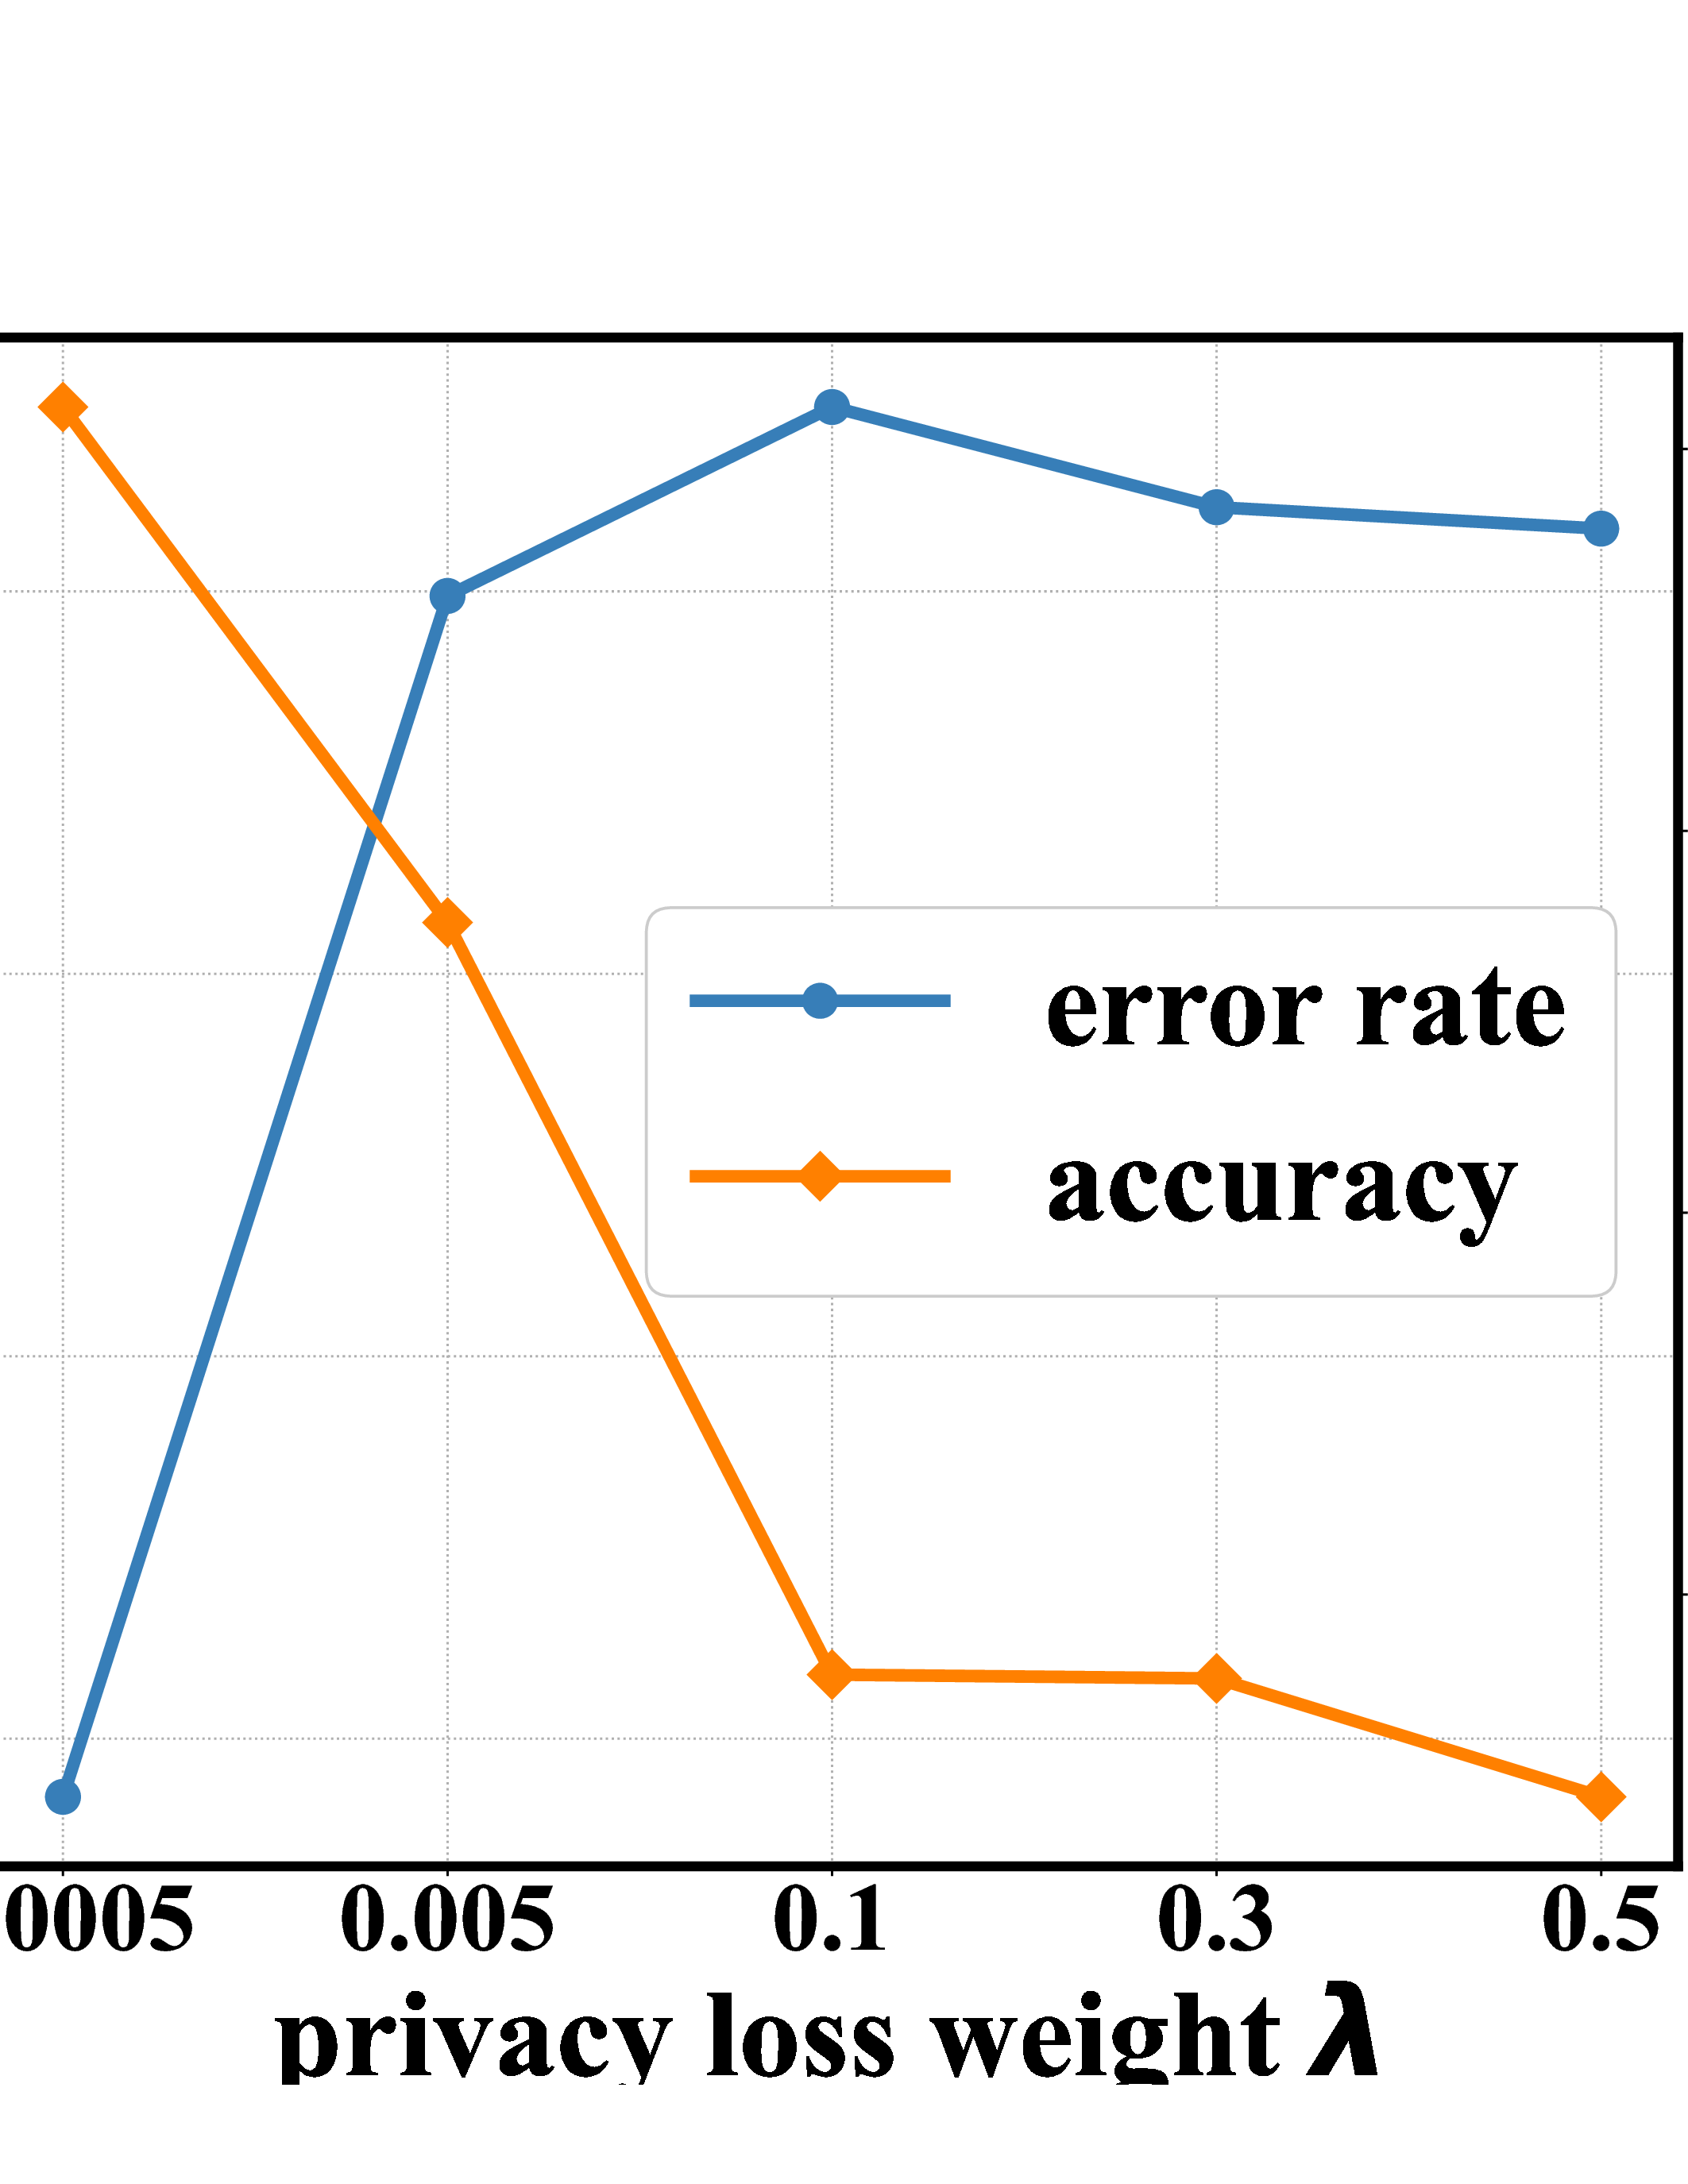}}
		\caption{The impact of privacy loss weight $\lambda$.}
		\label{fig:naive_defense}
	\end{minipage}
	\begin{minipage}[b]{0.45\textwidth} %所有minipage宽度之和要小于1，否则会自动变成竖排
		\centering  %图片全局居中
		\subfigure[Client1, attack 9-category attribute.]{
			\label{fig:adult_party1}
			\includegraphics[width=0.45\textwidth]{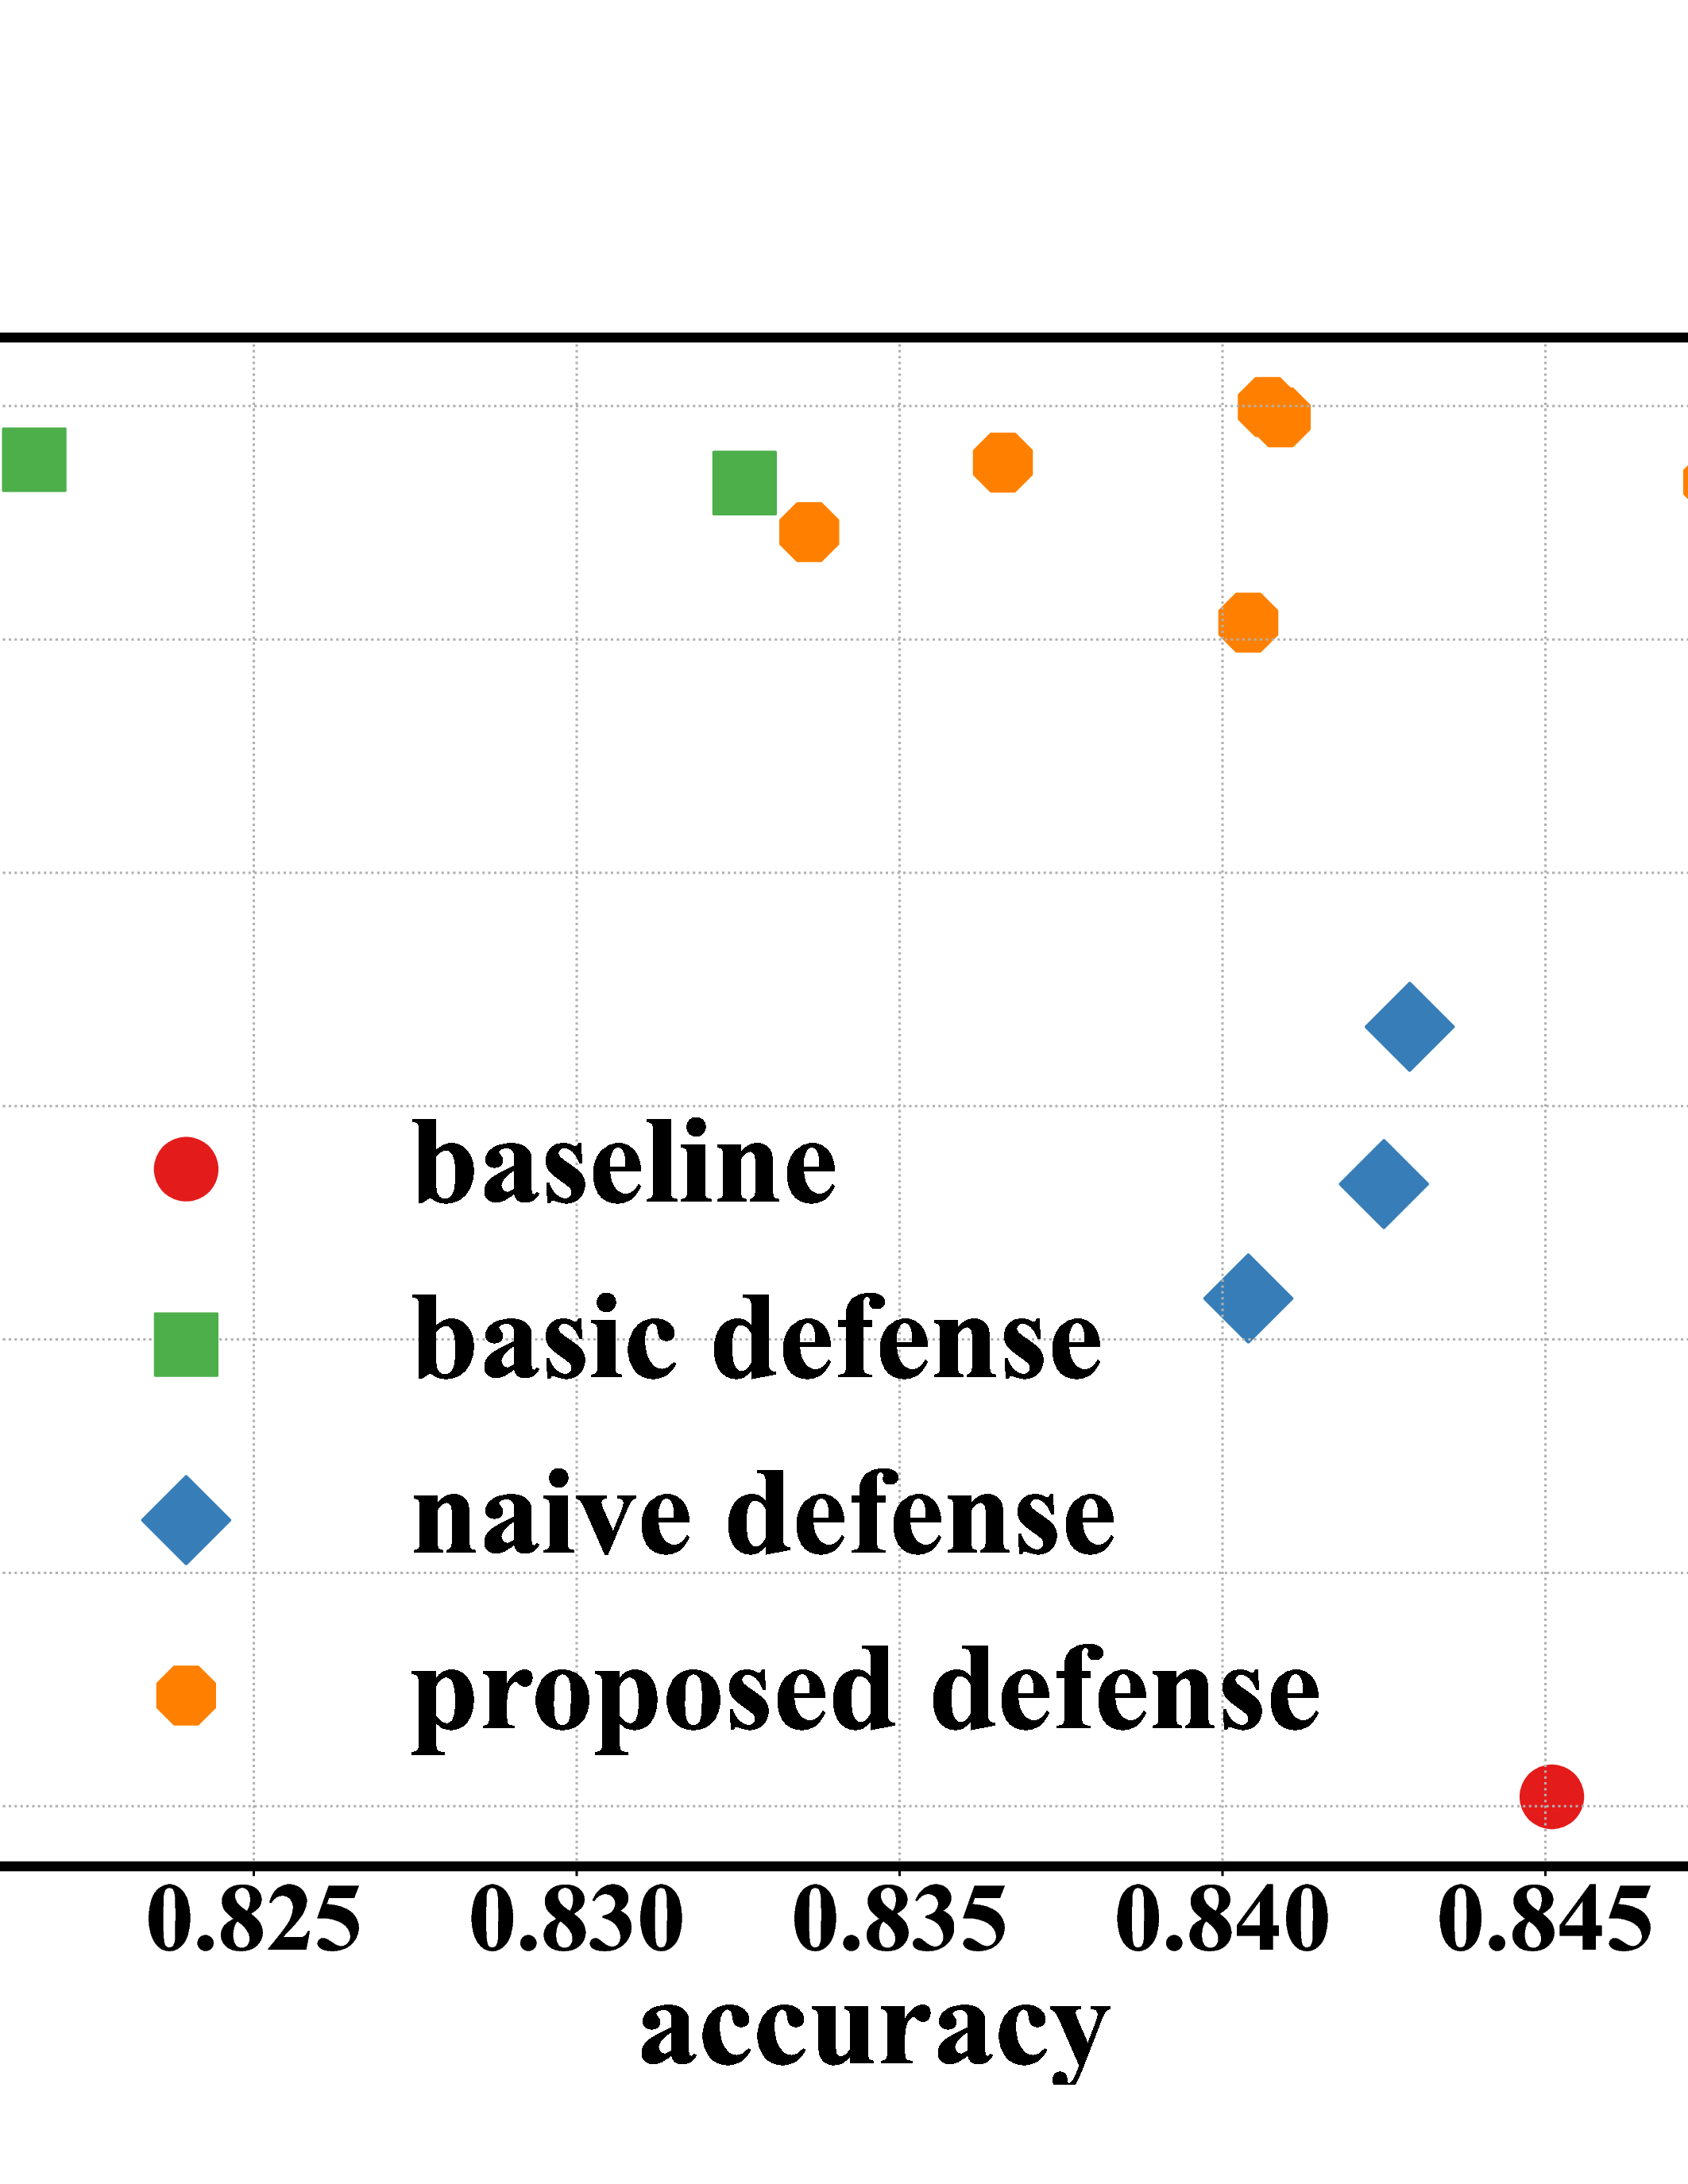}}
		\subfigure[Client2, attack 15-category attribute.]{
			\label{fig:adult_party2}
			\includegraphics[width=0.45\textwidth]{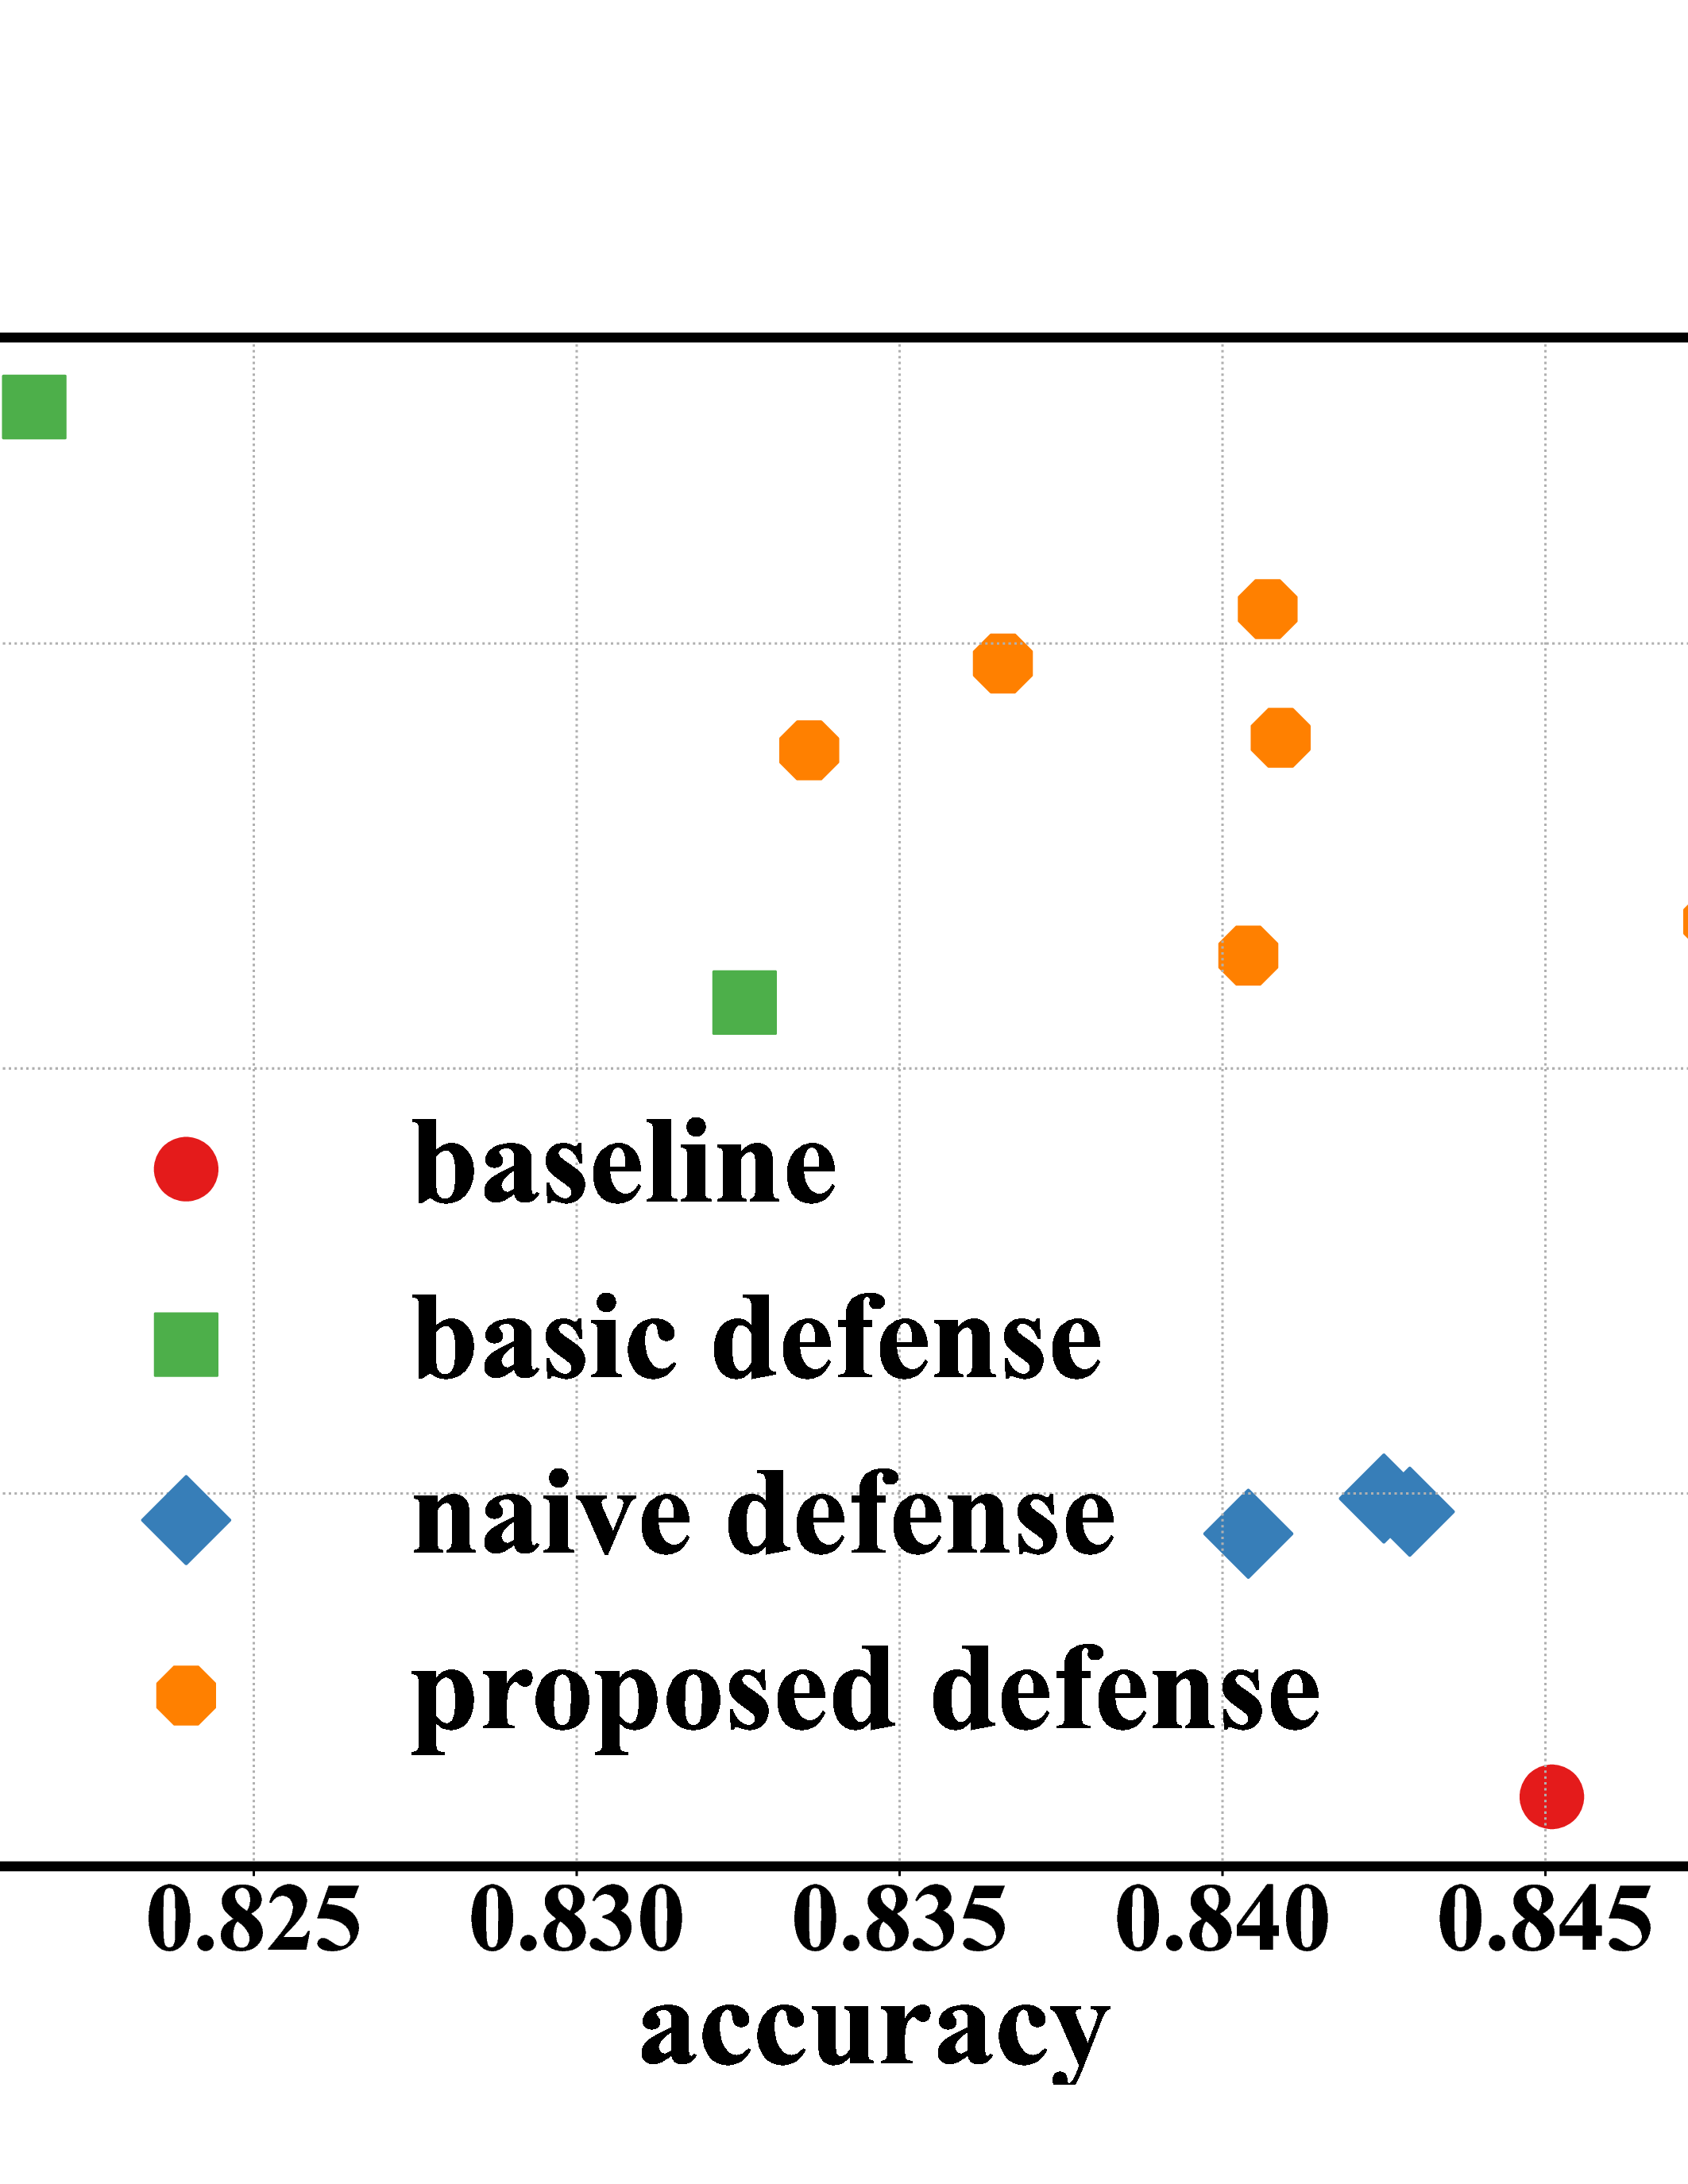}}		
		\caption{Three clients on Adult.}
		\label{fig:adult_multi_party}
	\end{minipage}
\end{figure}
%
%\begin{figure}[b]
%	\centering  %图片全局居中
%	\subfigure[Purchase, recall, $\alpha=0.05$]{
%		\label{fig:naive_defense1}
%		\includegraphics[width=0.22\textwidth]{figures/results/purchase/purchase_defense1.eps}}
%	\subfigure[Adult, error rate, $\alpha=0.05$]{
%		\label{fig:naive_defense2}
%		\includegraphics[width=0.22\textwidth]{figures/results/adult/adult_feature2_defense1.eps}}
%	\caption{The impact of privacy loss weight $\lambda$.}
%	\label{fig:naive_defense}
%\end{figure}
%\begin{figure}[h]
%	\centering  %图片全局居中
%	\subfigure[Client1, attack 9-category attribute.]{
%		\label{fig:adult_party1}
%		\includegraphics[width=0.22\textwidth]{figures/results/adult/adult_feature2_multi_party.eps}}
%	\subfigure[Client2, attack 15-category attribute.]{
%		\label{fig:adult_party2}
%		\includegraphics[width=0.22\textwidth]{figures/results/adult/adult_feature4_multi_party.eps}}		
%	\caption{Three clients on Adult.}
%	\label{fig:adult_multi_party}
%\end{figure}

\subsubsection{Attack performance vs. batch size.}
We present the attack performance over different batch sizes on Purchase and Credit using different privacy metrics (i.e. error rate, precision and f1-score) in Tab.~\ref{tab:all_batch_size}. The results demonstrate that as the batch size increases, the attack success rate is higher since a larger batch size means higher probability that data are collected from the same batch, which facilitates convergence.

\subsection{Defense}
Fig.~\ref{fig:all_defense1} and Fig.~\ref{fig:all_defense2} are the results of different defense methods for Purchase using different privacy metrics (i.e. precision and f1-score). 
Fig.~\ref{fig:all_defense3} is the defense result for COCO-QA using f1-score.
Fig.~\ref{fig:all_defense4} is the defense result for Adult where the adversary aims to attack a new 9-category attribute.

Figures show that the proposed defense can still achieve high privacy on different privacy metrics. On average, the proposed defense only brings $0.45\%$ accuracy drop on Purchase, $3.38\%$ on COCO-QA, and $0.64\%$ on Adult. 

\begin{figure}[t]
	\centering  %图片全局居中
	\subfigure[Purchase, binary classification of 300 attributes, random guess precision $0.5$]{
		\label{fig:all_defense1}
		\includegraphics[width=0.22\textwidth]{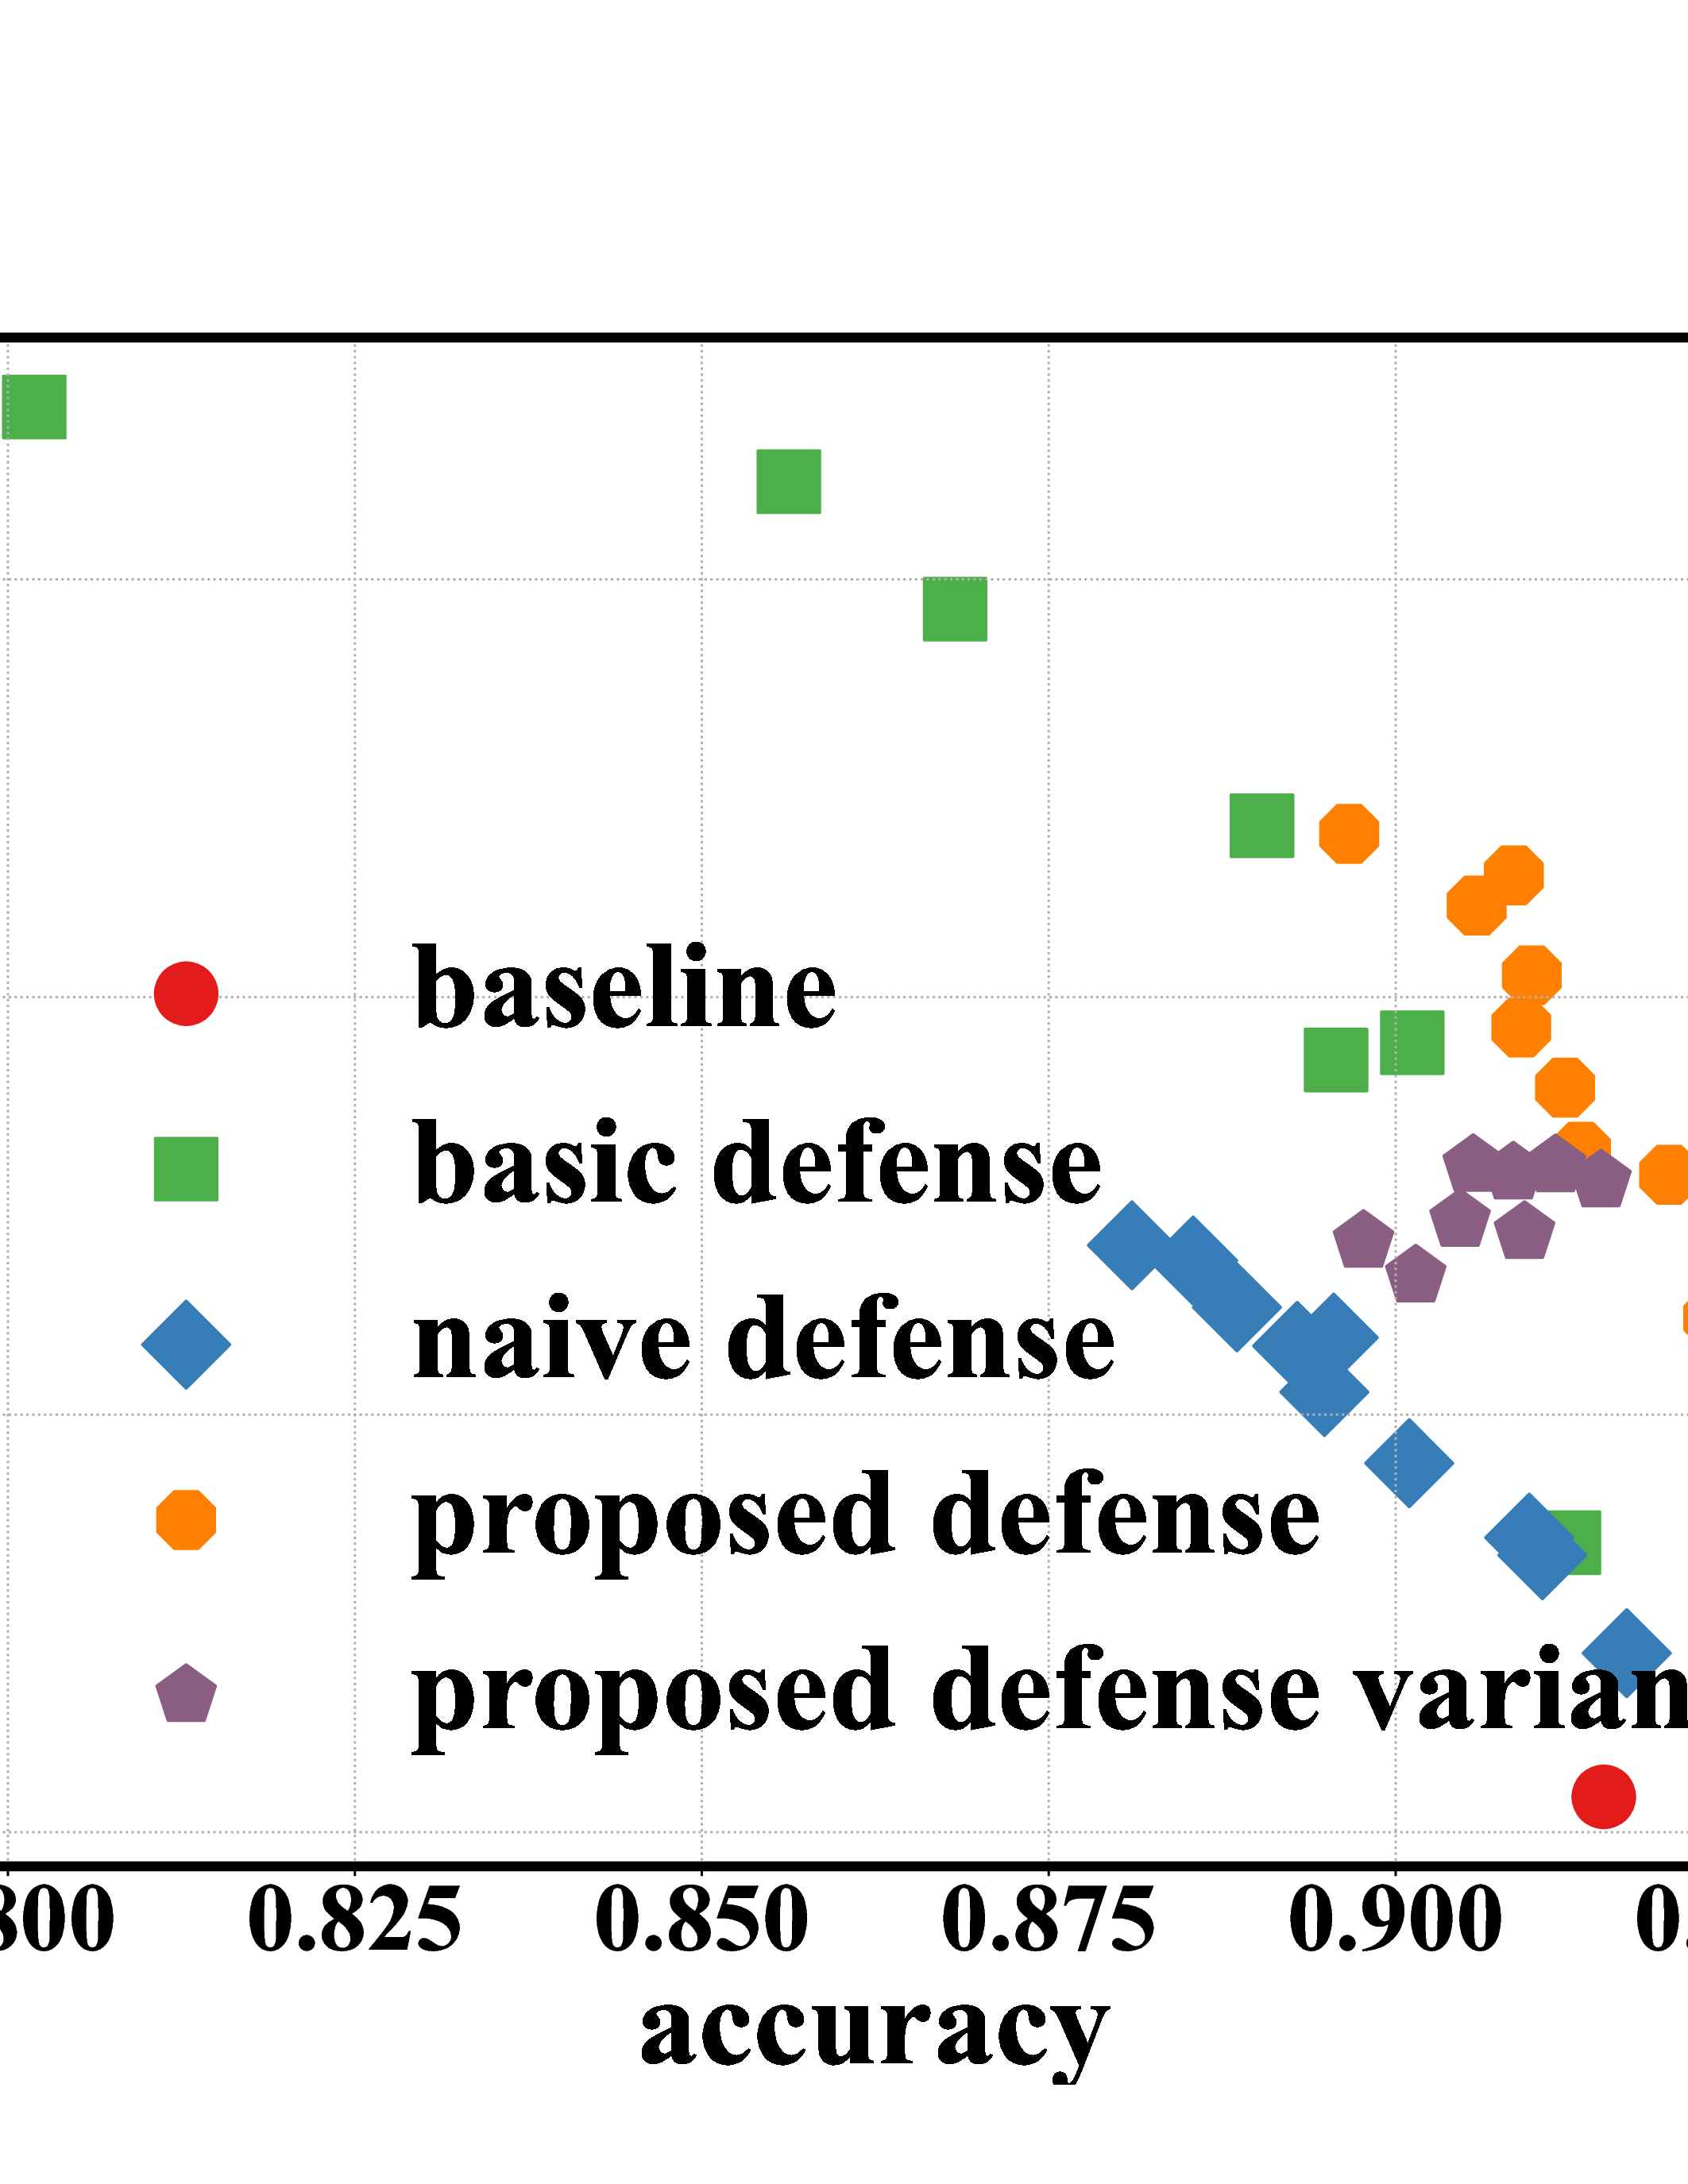}}
	\subfigure[Purchase, binary classification of 300 attributes, random guess f1-score $0.5$]{
		\label{fig:all_defense2}
		\includegraphics[width=0.22\textwidth]{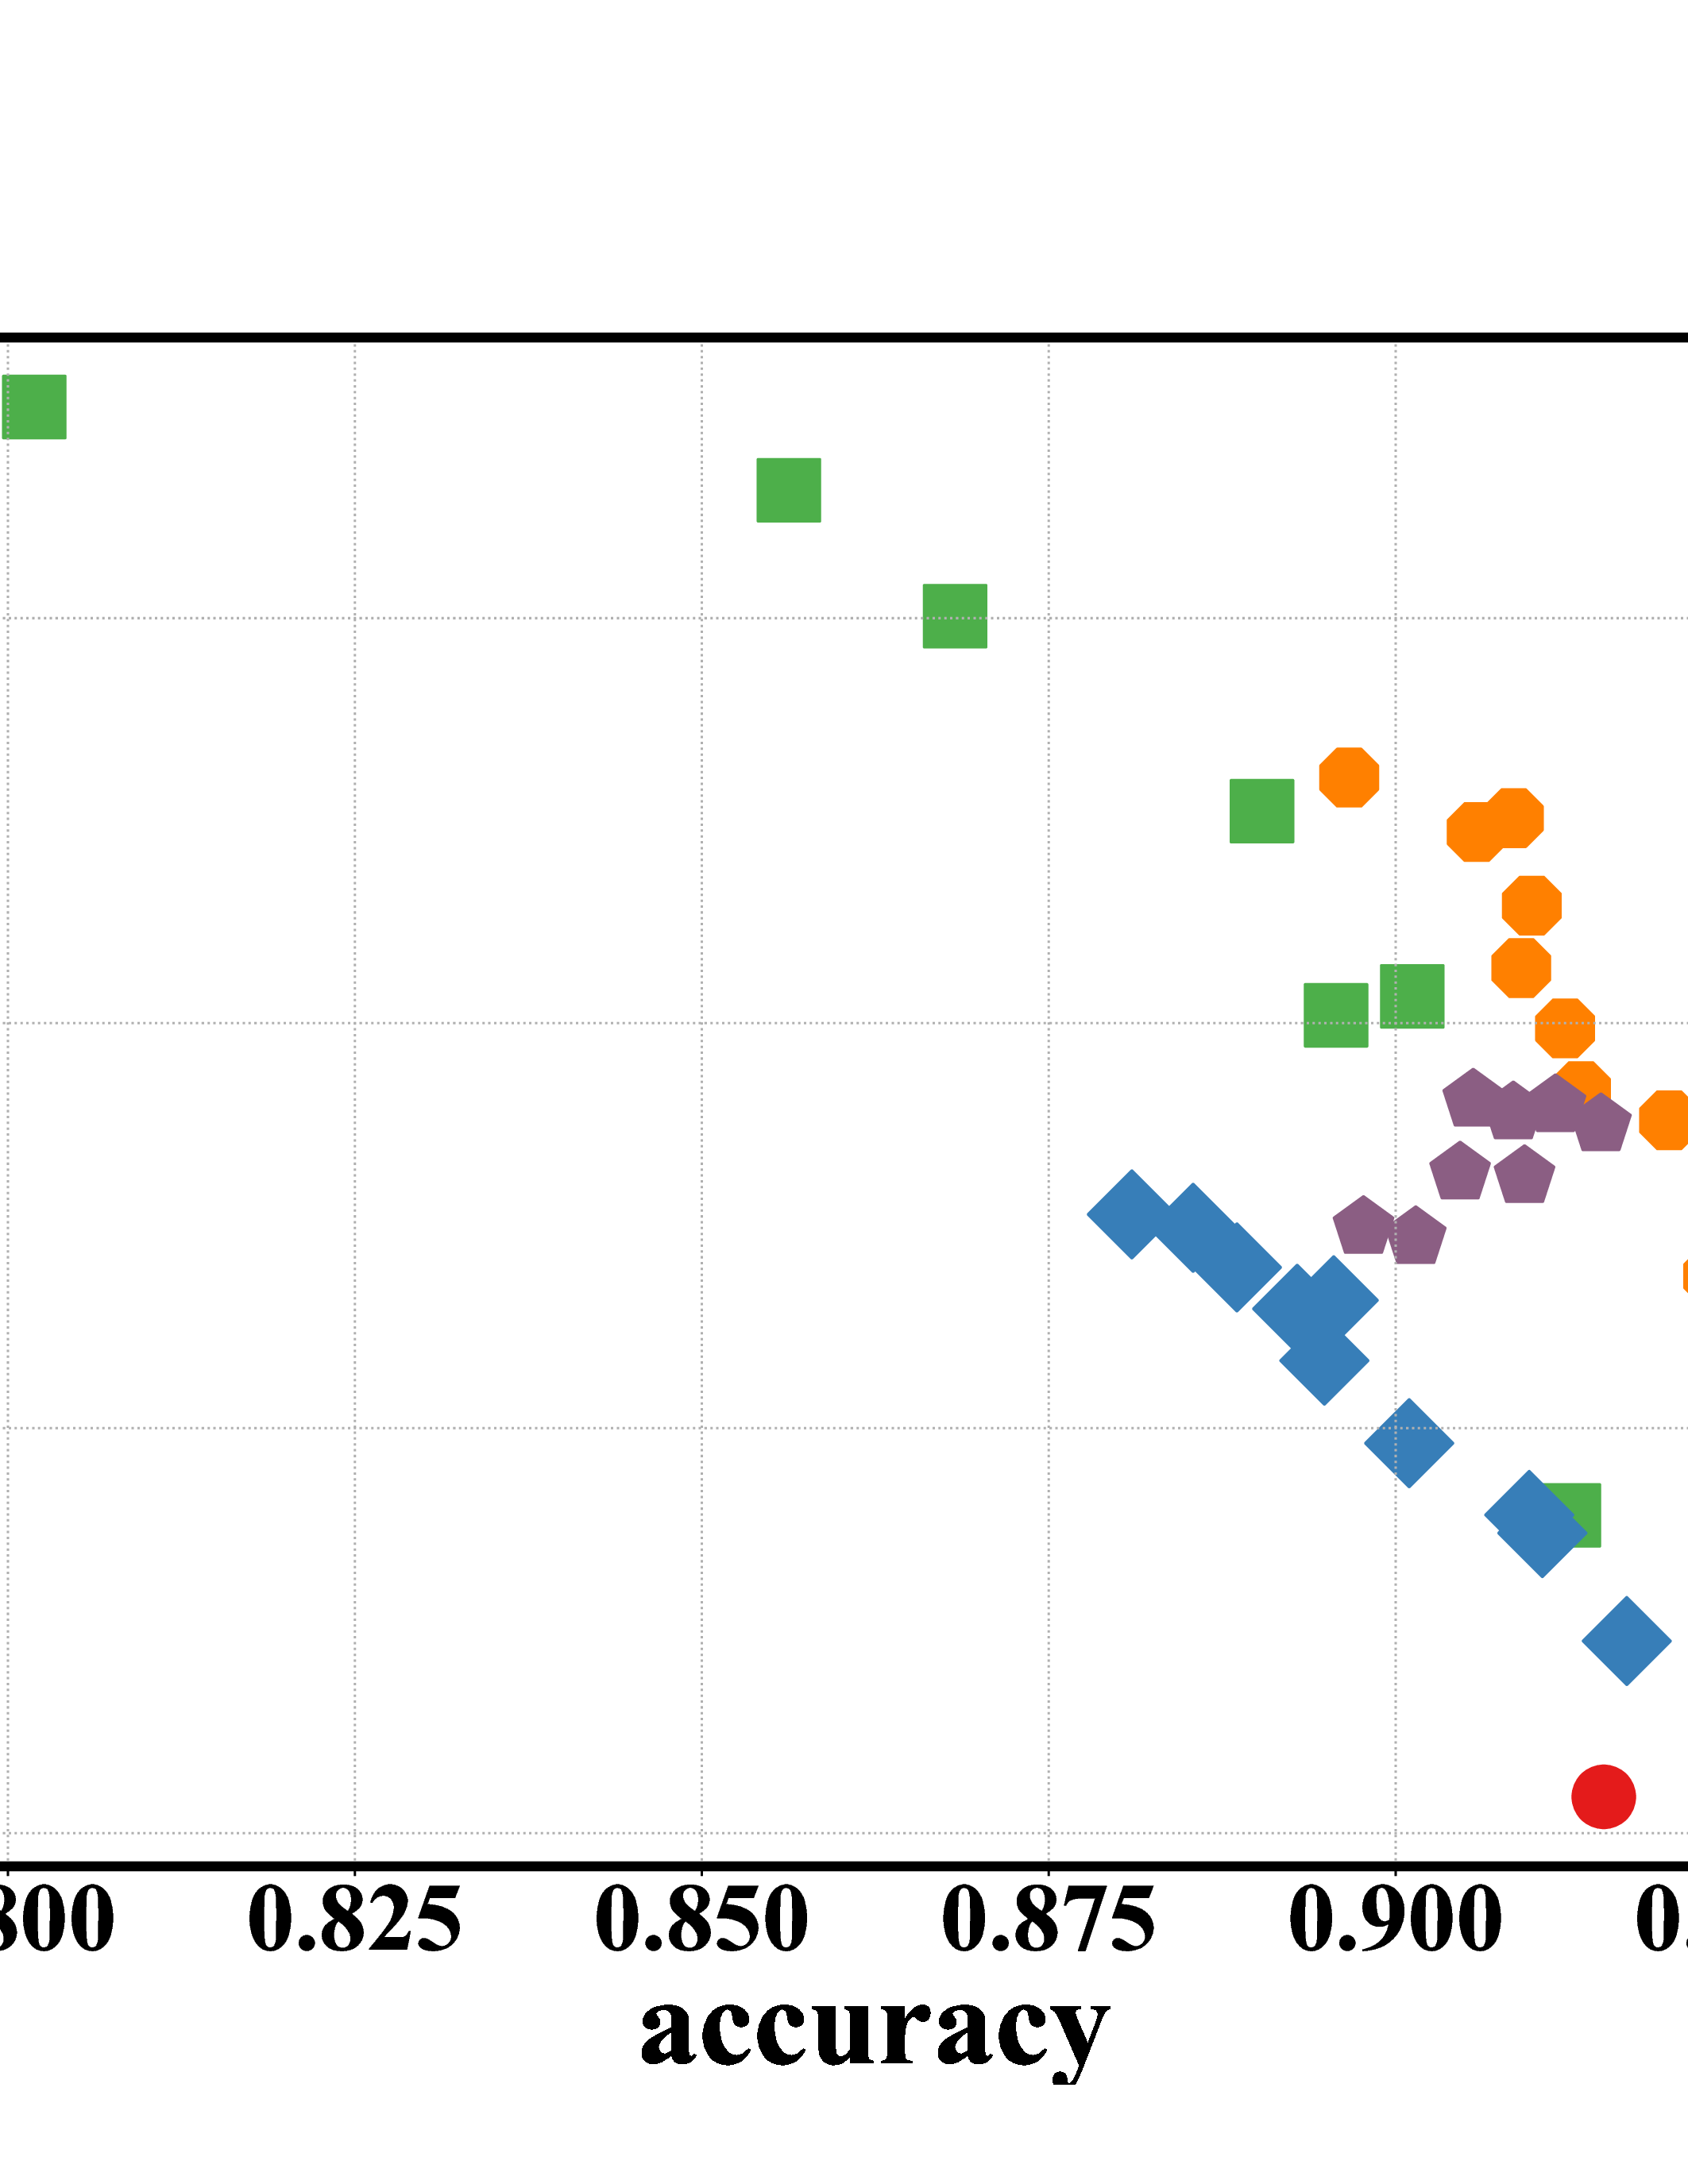}}
	\subfigure[COCO-QA, binary classification on multi-objects, random guess f1-score $0.0$ due to sparsity]{
		\label{fig:all_defense3}
		\includegraphics[width=0.22\textwidth]{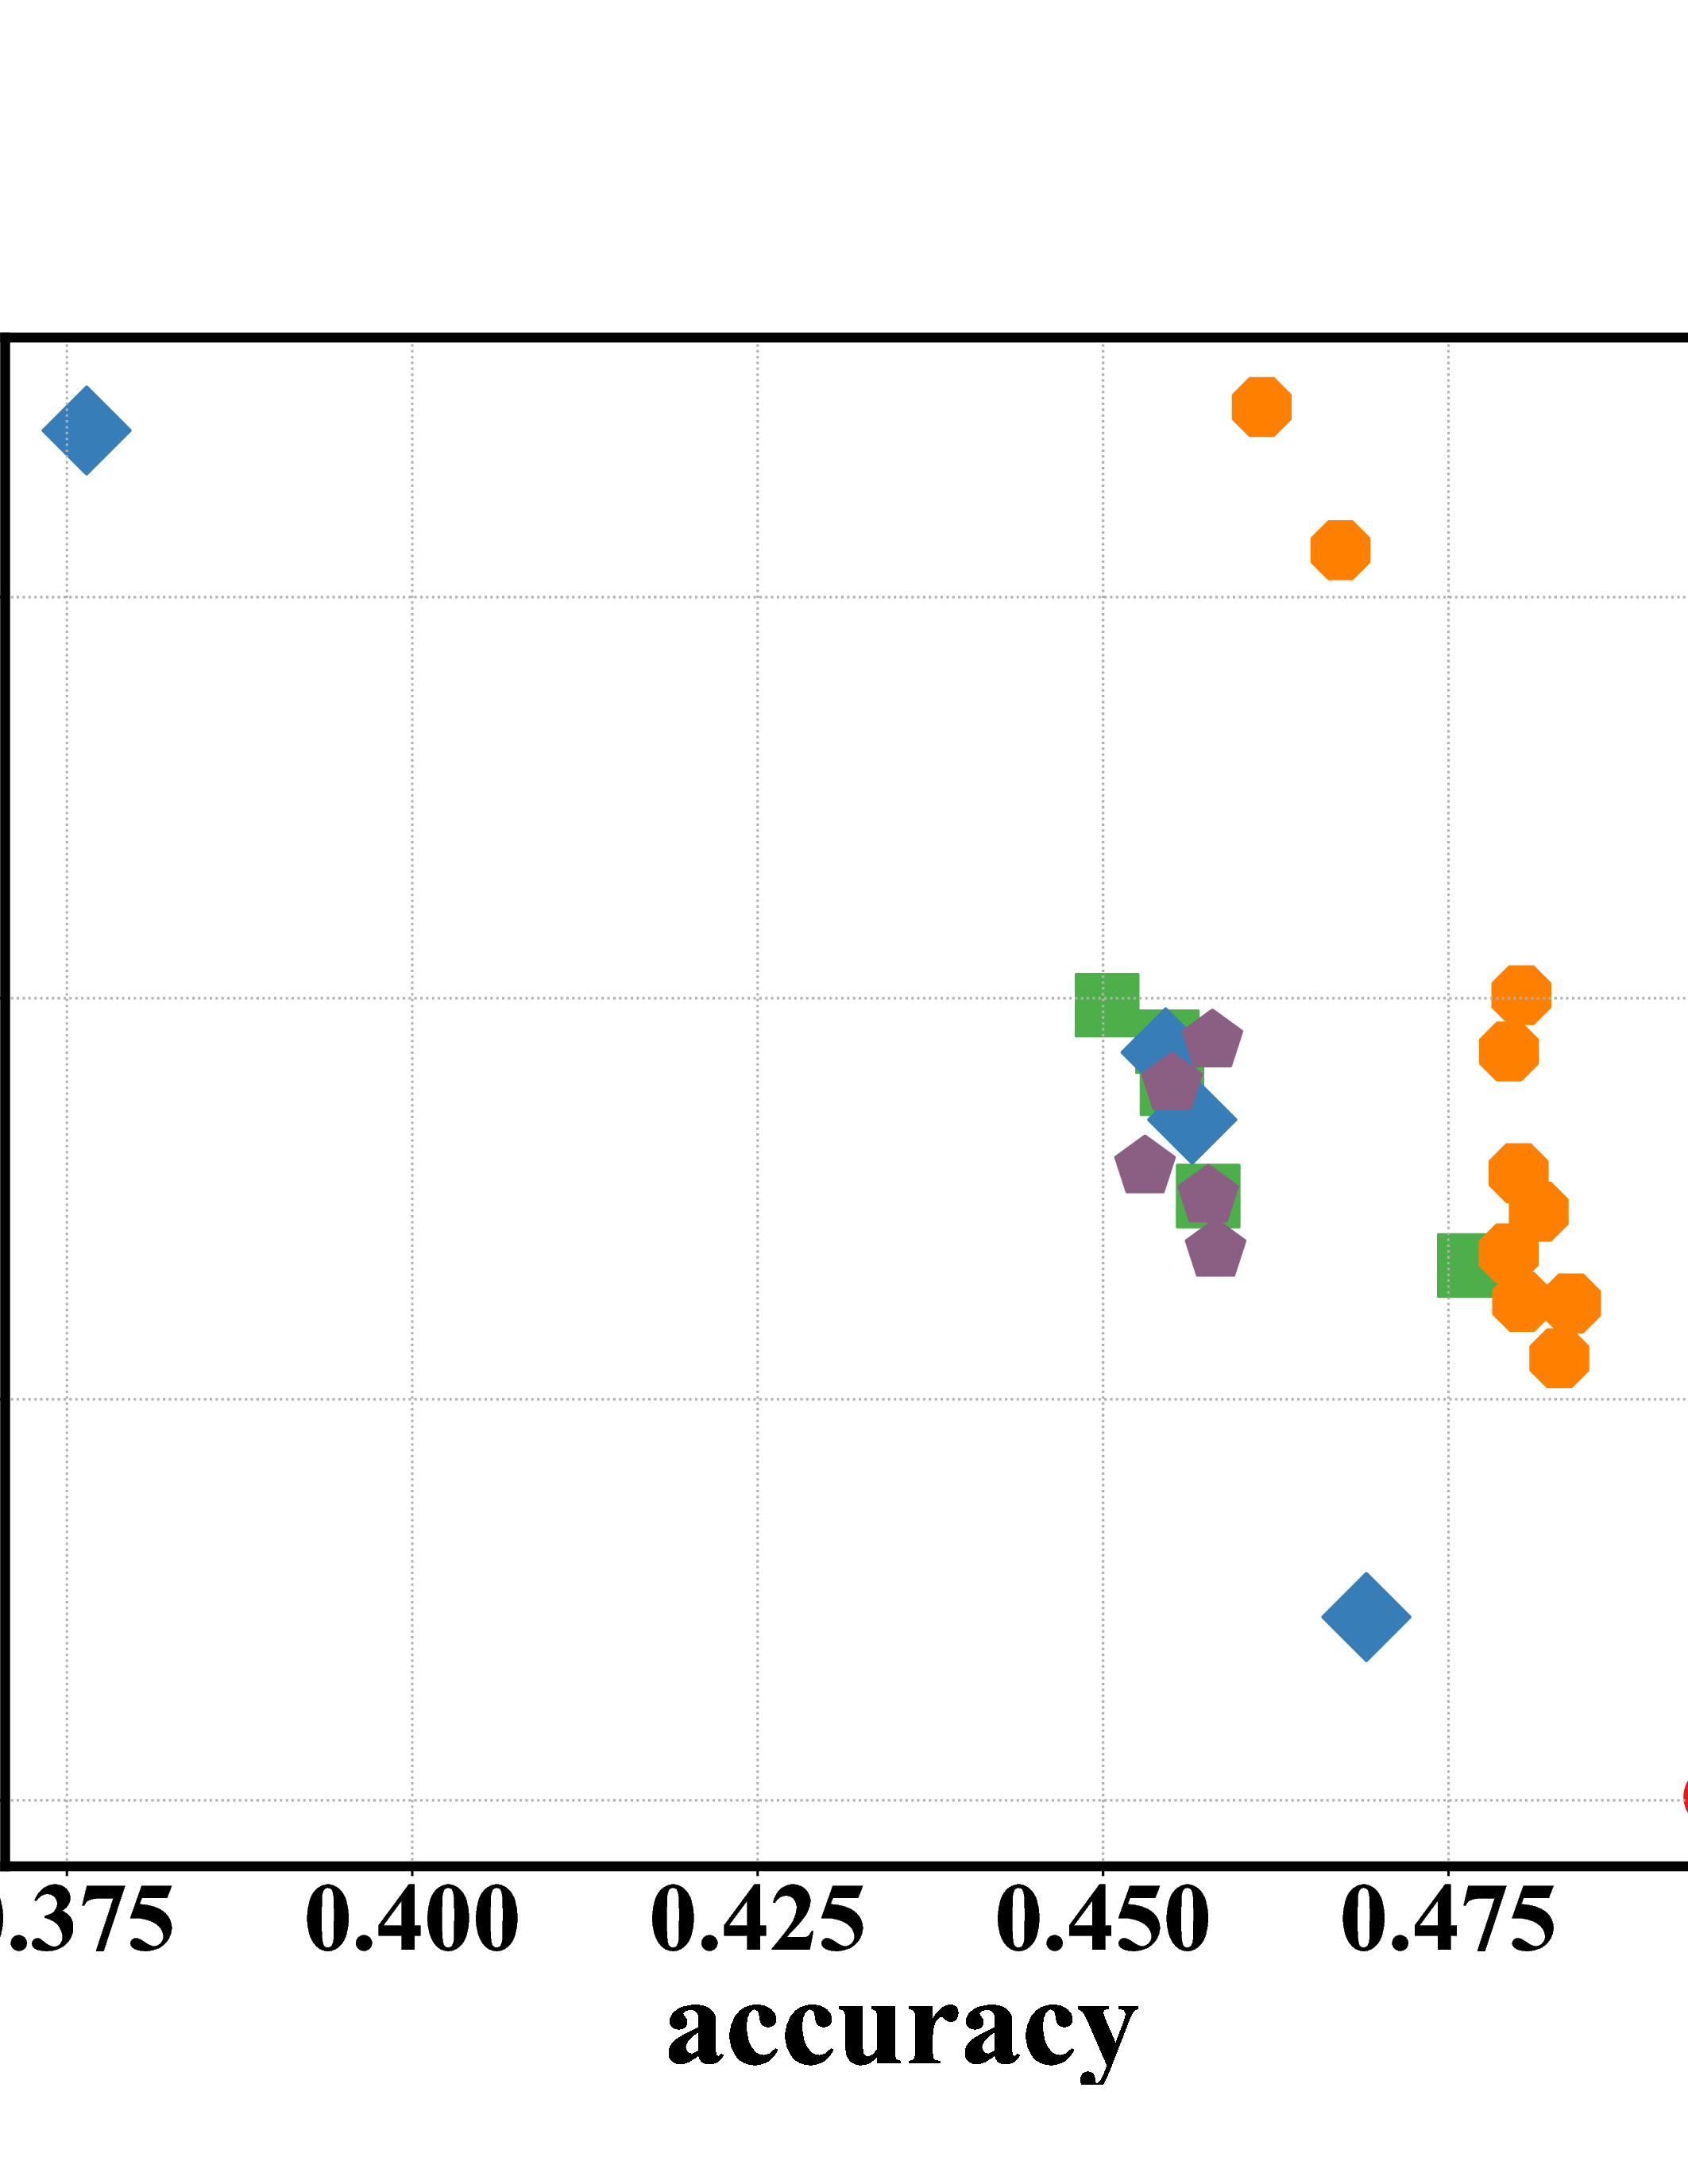}}
	\subfigure[Adult, 1-out-of-9 classification, random guess error rate $8/9$]{
		\label{fig:all_defense4}
		\includegraphics[width=0.22\textwidth]{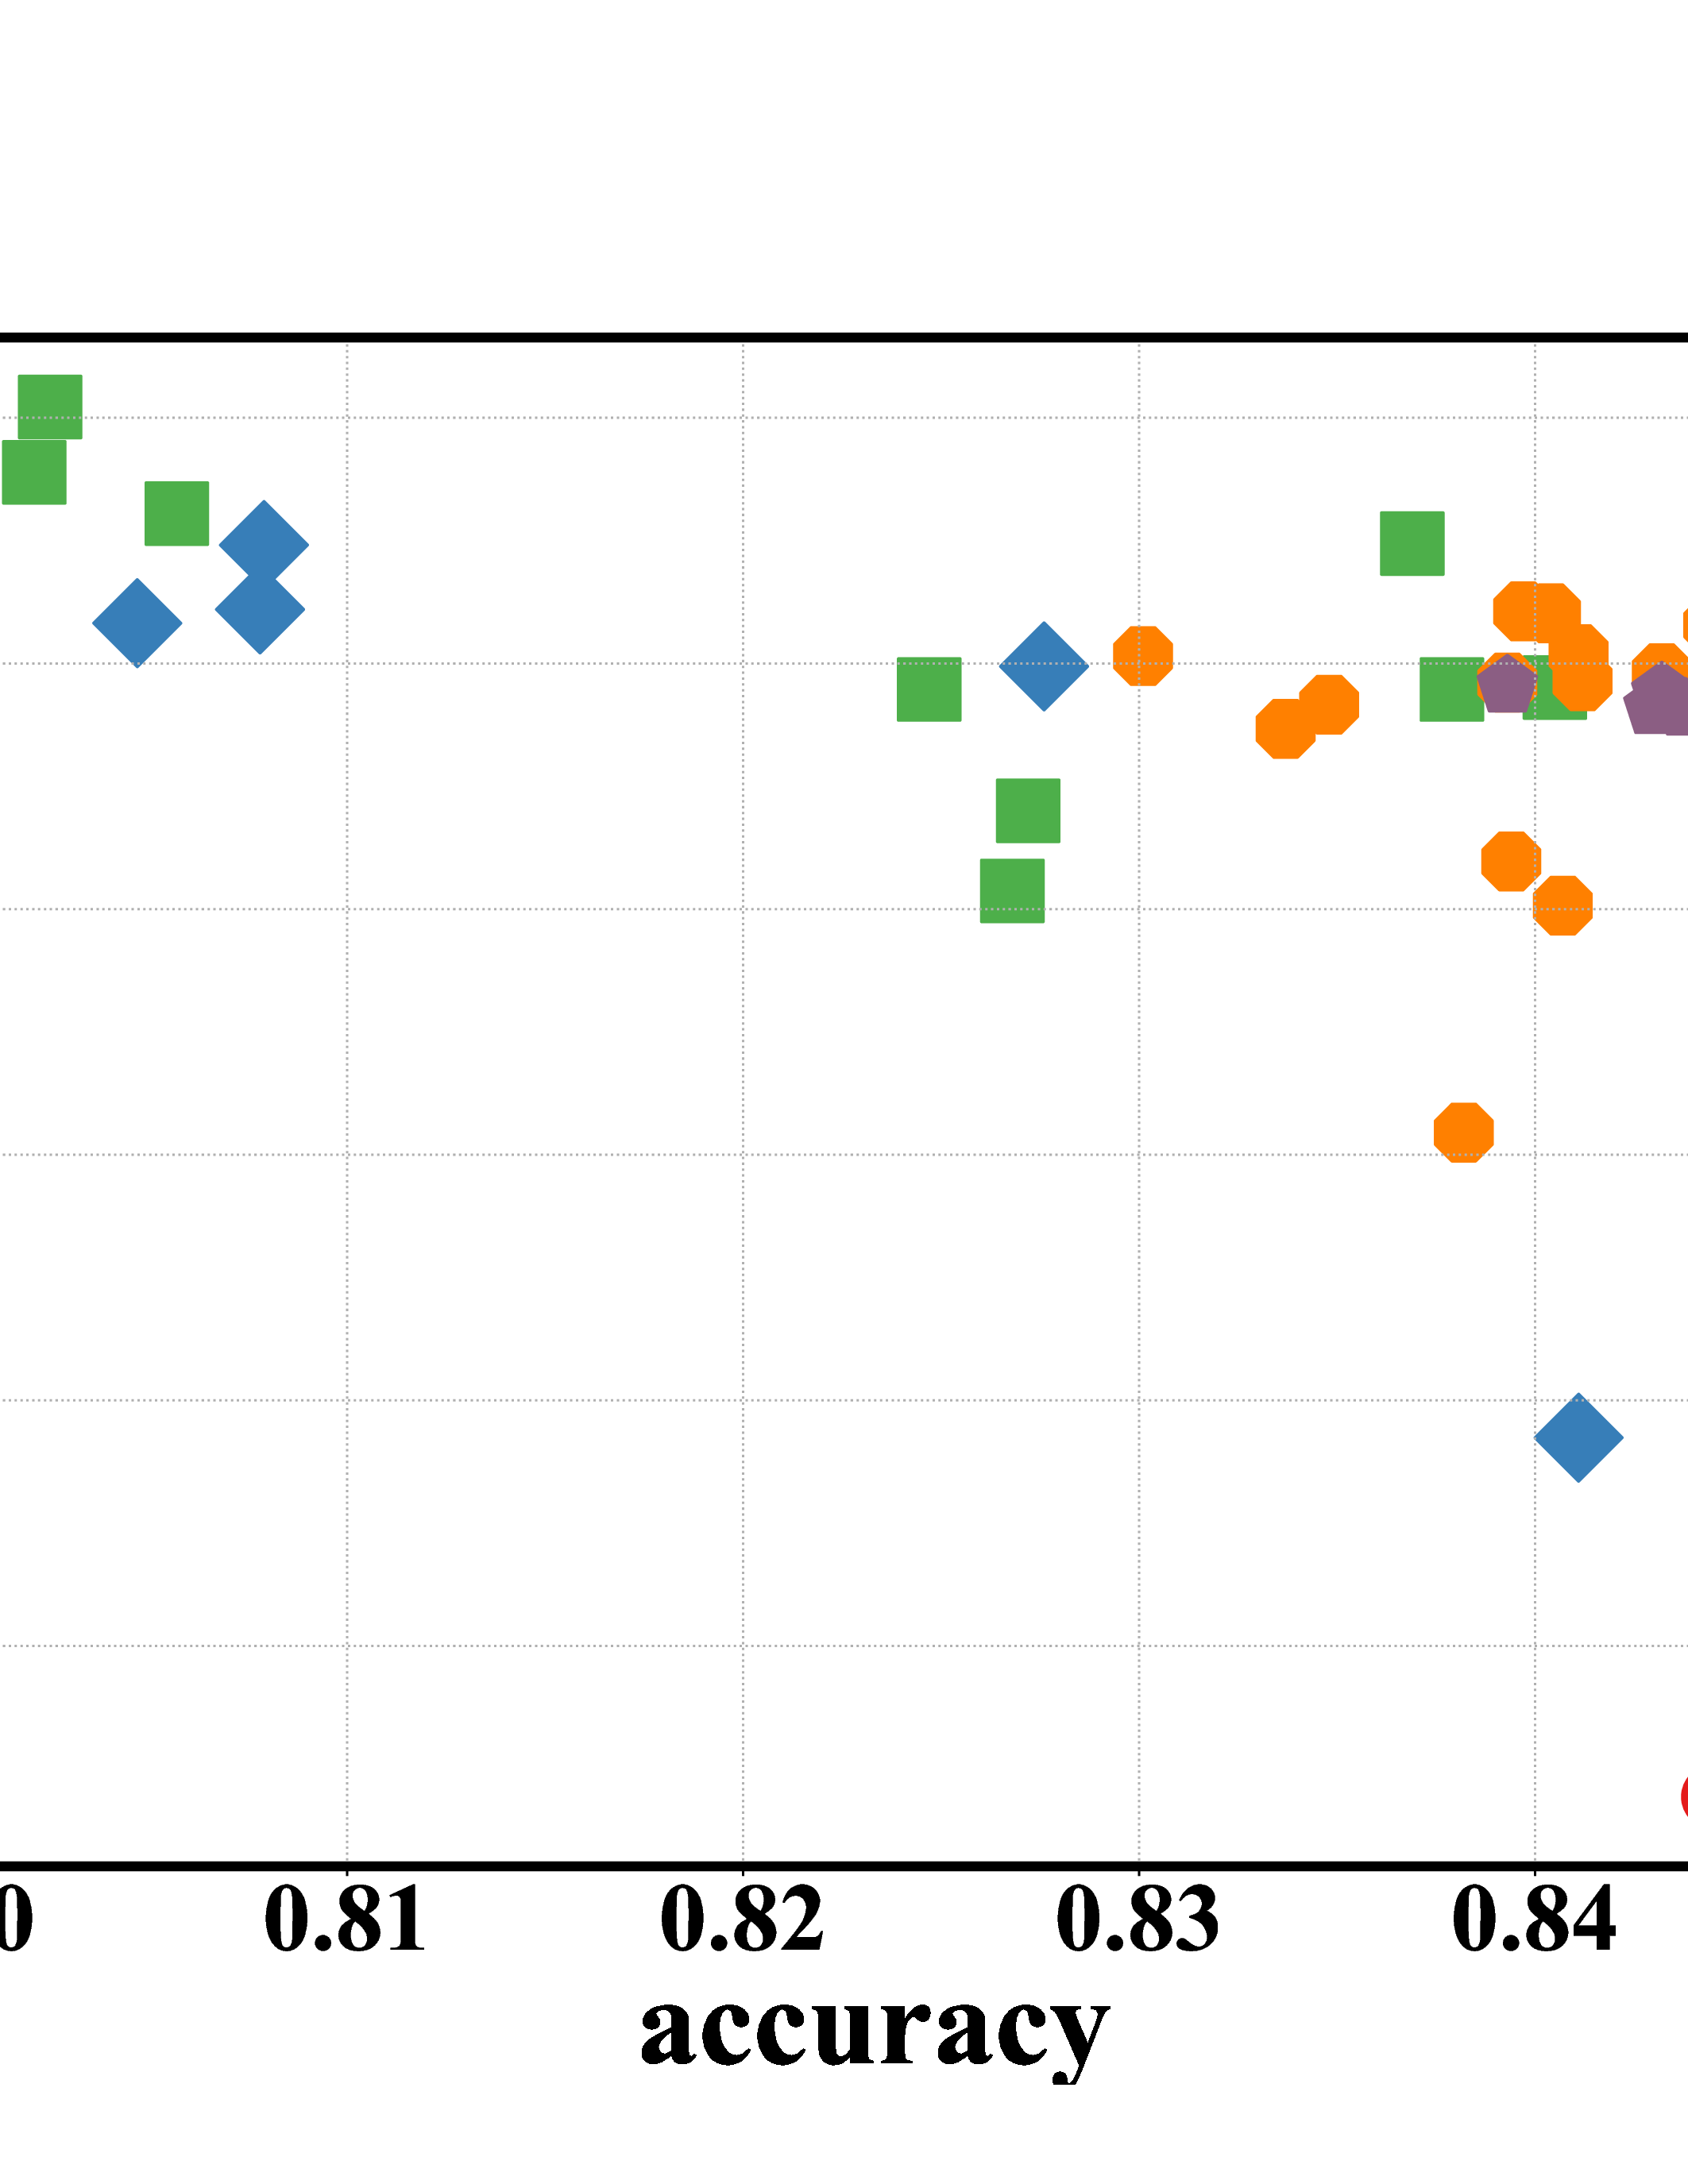}}
	\caption{Defense results using different privacy metrics. Legends are shared.}
	\label{fig:all_defense}
\end{figure}
\begin{table}[h]
	\scalebox{0.90}{
		\centering
		\begin{tabular}{ c | c | c | c | c }
			\toprule
			Dataset & Batch size & 32     & 128      & 256      \\ \hline
			\multirow{2}{*}{\begin{tabular}[c]{@{}c@{}}Purchase\\ (error rate)\end{tabular}} & Static & 0.0116 & 0.0099   & 0.0068  \\ \cline{2-5} 
			& Adaptive & 0.0081 & 0.0024 & 0.0012   \\ \hline
			\multirow{2}{*}{\begin{tabular}[c]{@{}c@{}}Purchase\\ (precision)\end{tabular}}    & Static & 0.9901 & 0.9906 & 0.9934 \\ \cline{2-5} 
			& Adaptive & 0.9915 & 0.9973 & 0.9984 \\ \hline
			\multirow{2}{*}{\begin{tabular}[c]{@{}c@{}}Purchase\\ (f1-score)\end{tabular}}     & Static & 0.9871 & 0.9890   & 0.9925   \\ \cline{2-5} 
			& Adaptive & 0.9910 & 0.9973   & 0.9984   \\ \hline
			\multirow{2}{*}{\begin{tabular}[c]{@{}c@{}}Credit\\ (MSE$\times 10^{-4}$)\end{tabular}}         & Static & 2.8092 & 1.9172   & 1.8033   \\ \cline{2-5} 
			& Adaptive & 3.7854 & 2.6557   & 2.3061   \\ 
			\bottomrule
		\end{tabular}
		\centering}
	\caption{Attack performance vs. batch size.}
	\label{tab:all_batch_size}
\end{table}

\subsubsection{Impact of privacy loss weight $\lambda$ in naive defence.}
We conduct the experiments on Purchase (Fig.~\ref{fig:naive_defense1}) using different privacy metrics and on Adult (Fig.~\ref{fig:naive_defense2}) using error rate. We observe a larger privacy loss weight $\lambda$ leads to accuracy drop and privacy improvement which is consistent with our intuition. Recall that the objective of native defense is $f(\cdot) + \lambda g(\cdot)$ and higher $\lambda$ means the vertical federated learning pays more attention to privacy and therefore leads to higher privacy.

\subsubsection{Multi party on Adult.}
Fig.~\ref{fig:adult_multi_party} is the results of three clients on Adult. One client is controlled by an honest-but-curious adversary and other benign clients try to protect their attributes. The adversary aims to attack a 9-category attribute and a 15-category attribute which respectively reside on the two benign clients. We observe that our proposed defense has balanced performance overall.
